# Supplementary material for: Surgical Data Science -- from Concepts toward Clinical Translation
Source: arXiv:2011.02284 source file (2021-07-30)
Supplement: Supplementary file 1 [file delphiRound2ResultsAgreement.pdf]

# Delphi Process on Surgical Data Science - Round 2

## Results: Agreement on premise, mission statements and goals

The survey of round 2 was completed by 40 participants. The distribution of responses related to the agreement on the premise, the mission statements and the goals is listed in the following sections.

# Premise

The following premise will be included for all missions: Unless otherwise specified, the premise for all of the following text is that: a) surgical data science represents the general context of the suggested phrases and b) “data” may pertain to any part of the patient care process (from initial presentation to long-term outcomes), may concern the patient, caregivers and/or technology used to deliver care and must be acquired, stored, and shared in accordance with regulatory constraints.

Do you agree with the premise?

| **Answer** | **Count** | **Percentage** |
| --- | --- | --- |
| Strongly Agree | 21 | 52.50% |
| Agree | 17 | 42.50% |
| Neither agree nor disagree | 2 | 5.00% |
| Disagree | 0 | 0.00% |
| Strongly Disagree | 0 | 0.00% |
| Comments | 7 | 17.50% |

# Area 1: Technical infrastructure

## Mission

**Mission Statement:** The mission statement shall cover the overarching mission corresponding to the technical infrastructure in healthcare institutions in one concise sentence. The original mission statement was “Make the data needed for training, testing and deploying SDS algorithms accessible and exchangeable, both live and retrospectively.”. The mission statement was supported by 92.1% (disagree/strongly disagree: 5.3%). Based on your comments, we revised the statement as follows: “Make the data needed for training, validating, evaluating and applying SDS algorithms safely accessible to and exchangeable between researchers and clinicians, both live and retrospectively.”

Do you agree with the revised mission statement?

| **Answer** | **Count** | **Percentage** |
| --- | --- | --- |
| Strongly Agree | 15 | 37.50% |
| Agree | 22 | 55.00% |
| Neither agree nor disagree | 2 | 5.00% |
| Disagree | 0 | 0.00% |
| Strongly Disagree | 1 | 2.50% |
| Comments | 10 | 25.00% |

# Goals

**NEW Goal 1.1:** Convince political and clinical stakeholders that an investment in clinical information infrastructure and dedicated data management and processing personnel is key to exploit the potential of artificial intelligence for interventional healthcare.

Do you agree with the new goal?

| Answer | Count | Percentage |
|---|---|---|
| Strongly Agree | 26 | 65.00% |
| Agree | 14 | 35.00% |
| Neither agree nor disagree | 0 | 0.00% |
| Disagree | 0 | 0.00% |
| Strongly Disagree | 0 | 0.00% |
| Comments | 7 | 17.50% |

**Goal 1.2 (previous goal 1.1):** The original phrasing was "Enhance clinical infrastructure in hospitals such that relevant data can be prospectively acquired and permanently stored.". 92.1% considered the goal as important/very important, and the previous phrasing was supported by 81.6% (disagree/strongly disagree: 13.2%). Based on your comments, we revised the statement as follows: "Enhance clinical information infrastructure including dedicated personnel resources in healthcare institutions such that relevant data can be prospectively, routinely, systematically acquired and stored in a user-friendly manner."

Do you agree with the revised goal?

| Answer | Count | Percentage |
|---|---|---|
| Strongly Agree | 26 | 65.00% |
| Agree | 12 | 30.00% |
| Neither agree nor disagree | 0 | 0.00% |
| Disagree | 2 | 5.00% |
| Strongly Disagree | 0 | 0.00% |
| Comments | 11 | 27.50% |

**Goal 1.3 (previous goal 1.2):** The original phrasing was "Enhance clinical infrastructure in hospitals such that data are easily exchangeable between systems.". 92.1% considered the goal as important/very important, and the previous phrasing was supported by 81.6% (disagree/strongly disagree: 10.5%). Based on your comments, we revised the statement as follows: "Enhance clinical information infrastructure in healthcare institutions such that data are exchangeable between data storage and acquisition systems and relatable to their clinical context."

Do you agree with the revised goal?

| Answer | Count | Percentage |
|---|---|---|
| Strongly Agree | 21 | 52.50% |
| Agree | 16 | 40.00% |
| Neither agree nor disagree | 1 | 2.50% |
| Disagree | 2 | 5.00% |
| Strongly Disagree | 0 | 0.00% |
| Comments | 9 | 22.50% |

**NEW Goal 1.4:** Develop standards for data storage with respect to duration and data quality.

Do you agree with the new goal?

| Answer | Count | Percentage |
|---|---|---|
| Strongly Agree | 18 | 45.00% |
| Agree | 16 | 40.00% |
| Neither agree nor disagree | 5 | 12.50% |
| Disagree | 1 | 2.50% |
| Strongly Disagree | 0 | 0.00% |
| Comments | 12 | 30.00% |

**NEW Goal 1.5:** Enhance clinical information infrastructure to enable real-time inference in interventional settings.

Do you agree with the new goal?

| Answer | Count | Percentage |
|---|---|---|
| Strongly Agree | 19 | 47.50% |
| Agree | 18 | 45.00% |
| Neither agree nor disagree | 2 | 5.00% |
| Disagree | 1 | 2.50% |
| Strongly Disagree | 0 | 0.00% |
| Comments | 7 | 17.50% |

**NEW Goal 1.6:** Build local and international collaborations and partnerships involving clinical, patient, academic, and industry stakeholders to implement goals 1.2-1.4 in an internationally coherent manner.

Do you agree with the new goal?

| Answer | Count | Percentage |
|---|---|---|
| Strongly Agree | 24 | 60.00% |
| Agree | 14 | 35.00% |
| Neither agree nor disagree | 1 | 2.50% |
| Disagree | 1 | 2.50% |
| Strongly Disagree | 0 | 0.00% |
| Comments | 11 | 27.50% |

# Area 2: Data annotation and sharing

## Mission

**Mission Statement:** The mission statement shall cover the overarching mission corresponding to data annotation and sharing in one concise sentence. The original mission statement was “Build up large annotated databases and facilitate sharing data across institutions.”. The mission statement was supported by 92.1% (disagree/strongly disagree: 5.3%). Based on your comments, we revised the statement as follows: “Facilitate sharing data across institutions and medical specialties and establish large annotated databases.”

Do you agree with the revised mission statement?

| Answer | Count | Percentage |
|---|---|---|
| Strongly Agree | 23 | 57.50% |
| Agree | 16 | 40.00% |
| Neither agree nor disagree | 0 | 0.00% |
| Disagree | 1 | 2.50% |
| Strongly Disagree | 0 | 0.00% |
| Comments | 8 | 20.00% |

## Goals

**Goal 2.1. (previous goal 2.3):** The original phrasing was “Establish shared ontologies for a standardized joint vocabulary.”. 84.2% considered the goal as important/very important, and the previous phrasing was supported by 81.6% (disagree/strongly disagree: 5.3%). Based on your comments, we revised the statement as follows: “Establish a common standardized ontology for surgical data science.”

Do you agree with the revised goal?

| Answer | Count | Percentage |
|---|---|---|
| Strongly Agree | 21 | 52.50% |
| Agree | 14 | 35.00% |
| Neither agree nor disagree | 2 | 5.00% |
| Disagree | 3 | 7.50% |
| Strongly Disagree | 0 | 0.00% |
| Comments | 5 | 12.50% |

**Goal 2.2. (previous goal 2.1):** The original phrasing was “Establish well-defined annotation standards and protocols.”. 94.7% considered the goal as important/very important, and the previous phrasing was supported by 94.7% (disagree/strongly disagree: 0.0%). Based on your comments, we revised the statement as follows: “Establish common annotation standards and protocols.”

Do you agree with the revised goal?

| Answer | Count | Percentage |
|---|---|---|
| Strongly Agree | 22 | 55.00% |
| Agree | 16 | 40.00% |
| Neither agree nor disagree | 1 | 2.50% |
| Disagree | 1 | 2.50% |
| Strongly Disagree | 0 | 0.00% |
| Comments | 4 | 10.00% |

**NEW Goal 2.3:** Establish best practices for assessing annotation quality.

Do you agree with the new goal?

| Answer | Count | Percentage |
|---|---|---|
| Strongly Agree | 23 | 57.50% |
| Agree | 15 | 37.50% |
| Neither agree nor disagree | 0 | 0.00% |
| Disagree | 2 | 5.00% |
| Strongly Disagree | 0 | 0.00% |
| Comments | 7 | 17.50% |

**Goal 2.4. (previous goal 2.2):** The original phrasing was “Establish best practices for assuring annotation quality.”. 84.2% considered the goal as important/very important, and the previous phrasing was supported by 81.6% (disagree/strongly disagree: 7.9%). Based on your comments, we will not revise the statement.

Do you agree with the original goal?

| Answer | Count | Percentage |
|---|---|---|
| Strongly Agree | 15 | 37.50% |
| Agree | 19 | 47.50% |
| Neither agree nor disagree | 4 | 10.00% |
| Disagree | 1 | 2.50% |
| Strongly Disagree | 1 | 2.50% |
| Comments | 8 | 20.00% |

**Goal 2.5. (previous goal 2.4):** The original phrasing was “Establish and promote annotation platforms that adhere to standards and protocols.”. 79.0% considered the goal as important/very important, and the previous phrasing was supported by 81.6% (disagree/strongly disagree: 5.3%). Based on your comments, we revised the statement as follows: “Develop and disseminate openly accessible platforms to enable adherence to annotation standards and protocols.”

Do you agree with the revised goal?

| Answer | Count | Percentage |
|---|---|---|
| Strongly Agree | 16 | 40.00% |
| Agree | 20 | 50.00% |
| Neither agree nor disagree | 3 | 7.50% |
| Disagree | 1 | 2.50% |
| Strongly Disagree | 0 | 0.00% |
| Comments | 6 | 15.00% |

**NEW Goal 2.6:** Establish best practices for user training in annotation.

Do you agree with the new goal?

| Answer | Count | Percentage |
|---|---|---|
| Strongly Agree | 16 | 40.00% |
| Agree | 20 | 50.00% |
| Neither agree nor disagree | 2 | 5.00% |
| Disagree | 2 | 5.00% |
| Strongly Disagree | 0 | 0.00% |
| Comments | 9 | 22.50% |

**Goal 2.7 (previous goal 2.5):** The original phrasing was "Establish platforms and workflows for sharing data.". 79% considered the goal as important/very important, and the previous phrasing was supported by 84.2% (disagree/strongly disagree: 2.6%). Based on your comments, we revised the statement as follows: "Establish platforms as well as new concepts and workflows for sharing data in a secure manner."

Do you agree with the revised goal?

| Answer | Count | Percentage |
|---|---|---|
| Strongly Agree | 15 | 37.50% |
| Agree | 21 | 52.50% |
| Neither agree nor disagree | 2 | 5.00% |
| Disagree | 2 | 5.00% |
| Strongly Disagree | 0 | 0.00% |
| Comments | 6 | 15.00% |

**Goal 2.8 (previous goal 2.6):** The original phrasing was "Provide more incentives for sharing and annotating data.". 71.1% considered the goal as important/very important, and the previous phrasing was supported by 78.9% (disagree/strongly disagree: 7.9%). Based on your comments, we revised the statement as follows: "Create more incentives for clinical staff and patients to share and annotate data."

Do you agree with the revised goal?

| Answer | Count | Percentage |
|---|---|---|
| Strongly Agree | 18 | 45.00% |
| Agree | 15 | 37.50% |
| Neither agree nor disagree | 2 | 5.00% |
| Disagree | 5 | 12.50% |
| Strongly Disagree | 0 | 0.00% |
| Comments | 6 | 15.00% |

**NEW Goal 2.9:** Enforce adherence to best practices, standards and protocols relevant to data annotation and sharing.

Do you agree with the new goal?

| Answer | Count | Percentage |
|---|---|---|
| Strongly Agree | 13 | 32.50% |
| Agree | 17 | 42.50% |
| Neither agree nor disagree | 3 | 7.50% |
| Disagree | 5 | 12.50% |
| Strongly Disagree | 2 | 5.00% |
| Comments | 15 | 37.50% |

# Area 3: Data analytics

## Mission

**Mission Statement:** The mission statement shall cover the overarching mission corresponding to the translational concepts for data science methods in one concise sentence. The original mission statement was “Make data science methods ready for clinical translation.”. The mission statement was supported by 76.3% (disagree/strongly disagree: 15.8%). Based on your comments, we revised the statement as follows: “Channel methods research according to key clinical objectives and metrics.”

Do you agree with the revised mission statement?

| Answer | Count | Percentage |
| --- | --- | --- |
| Strongly Agree | 10 | 25.00% |
| Agree | 18 | 45.00% |
| Neither agree nor disagree | 5 | 12.50% |
| Disagree | 7 | 17.50% |
| Strongly Disagree | 0 | 0.00% |
| Comments | 15 | 37.50% |

## Goals

**Goal 3.1:** The original phrasing was “Improve robustness and accuracy of algorithms.”. 89.5% considered the goal as important/very important, and the previous phrasing was supported by 89.5% (disagree/strongly disagree: 5.3%). Based on your comments, we revised the statement as follows: “Develop methods and validation concepts focused on robustness including generalization.”

Do you agree with the revised goal?

| Answer | Count | Percentage |
| --- | --- | --- |
| Strongly Agree | 20 | 50.00% |
| Agree | 15 | 37.50% |
| Neither agree nor disagree | 3 | 7.50% |
| Disagree | 2 | 5.00% |
| Strongly Disagree | 0 | 0.00% |
| Comments | 6 | 15.00% |

**Goal 3.2:** The original phrasing was “Enhance trust in AI-based solutions.”. 60.5% considered the goal as important/very important, and the previous phrasing was supported by 73.7% (disagree/strongly disagree: 7.9%). Based on your comments, we revised the statement as follows: “Develop methods and validation concepts focused on explainability.”

Do you agree with the revised goal?

| Answer | Count | Percentage |
| --- | --- | --- |
| Strongly Agree | 12 | 30.00% |
| Agree | 18 | 45.00% |
| Neither agree nor disagree | 5 | 12.50% |
| Disagree | 3 | 7.50% |
| Strongly Disagree | 2 | 5.00% |
| Comments | 15 | 37.50% |

**Goal 3.3:** The original phrasing was "Mitigate the need for large amounts of annotated data.". 68.4% considered the goal as important/very important, and the previous phrasing was supported by 81.6% (disagree/strongly disagree: 2.6%). Based on your comments, we revised the statement as follows: "Develop methods and validation concepts focused on learning efficiently from limited data."

Do you agree with the revised goal?

| Answer | Count | Percentage |
|---|---|---|
| Strongly Agree | 22 | 55.00% |
| Agree | 15 | 37.50% |
| Neither agree nor disagree | 1 | 2.50% |
| Disagree | 1 | 2.50% |
| Strongly Disagree | 1 | 2.50% |
| Comments | 7 | 17.50% |

**Goal 3.4 (previous goal 3.5):** The original phrasing was "Increase speed of algorithms to enable real-time inference.". 57.9% considered the goal as important/very important, and the previous phrasing was supported by 84.2% (disagree/strongly disagree: 5.3%). Based on your comments, we revised the statement as follows: "Develop methods and validation concepts focused on fast inference."

Do you agree with the revised goal?

| Answer | Count | Percentage |
|---|---|---|
| Strongly Agree | 11 | 27.50% |
| Agree | 22 | 55.00% |
| Neither agree nor disagree | 5 | 12.50% |
| Disagree | 1 | 2.50% |
| Strongly Disagree | 1 | 2.50% |
| Comments | 8 | 20.00% |

**NEW Goal 3.5:** Develop methods and validation concepts focused on dealing with and avoiding data biases and confounders.

Do you agree with the new goal?

| Answer | Count | Percentage |
|---|---|---|
| Strongly Agree | 20 | 50.00% |
| Agree | 14 | 35.00% |
| Neither agree nor disagree | 5 | 12.50% |
| Disagree | 1 | 2.50% |
| Strongly Disagree | 0 | 0.00% |
| Comments | 6 | 15.00% |

**Goal 3.6 (previous goal 3.4):** The original phrasing was “Generate thorough understanding of surgical processes.”. 78.9% considered the goal as important/very important, and the previous phrasing was supported by 71.1% (disagree/strongly disagree: 7.9%). Based on your comments, we revised the statement as follows: “Develop methods and validation concepts focused on the semantic understanding of surgical processes, including variability resulting from personnel- and patient-specific factors.”

Do you agree with the revised goal?

| Answer | Count | Percentage |
|---|---|---|
| Strongly Agree | 16 | 40.00% |
| Agree | 19 | 47.50% |
| Neither agree nor disagree | 3 | 7.50% |
| Disagree | 2 | 5.00% |
| Strongly Disagree | 0 | 0.00% |
| Comments | 9 | 22.50% |

**Goal 3.7 (previous goal 3.6):** The original phrasing was “Facilitate certification of algorithms.”. 68.4% considered the goal as important/very important, and the previous phrasing was supported by 65.8% (disagree/strongly disagree: 18.4%). Based on your comments, we revised the statement as follows: “Develop concepts and workflows for facilitating regulatory approval of algorithms.”

Do you agree with the revised goal?

| Answer | Count | Percentage |
|---|---|---|
| Strongly Agree | 21 | 52.50% |
| Agree | 15 | 37.50% |
| Neither agree nor disagree | 3 | 7.50% |
| Disagree | 1 | 2.50% |
| Strongly Disagree | 0 | 0.00% |
| Comments | 6 | 15.00% |

# Area 4: Clinical translation

## Mission

Mission Statement: The mission statement shall cover the overarching mission corresponding to the clinical translation in one concise sentence. The original mission statement was “Initiate paradigm shift in the clinics.”. The mission statement was supported by 50.0% (disagree/strongly disagree: 23.7%). Based on your comments, we revised the statement as follows: “Initiate a cultural shift towards data-driven clinical practice.”

Do you agree with the revised mission statement?

| Answer | Count | Percentage |
|---|---|---|
| Strongly Agree | 19 | 47.50% |
| Agree | 12 | 30.00% |
| Neither agree nor disagree | 5 | 12.50% |
| Disagree | 4 | 10.00% |
| Strongly Disagree | 0 | 0.00% |
| Comments | 7 | 17.50% |

## Goals

**Goal 4.1:** The original phrasing was “Catalyze clinical translation by generating first clinical SDS success stories.”. 84.2% considered the goal as important/very important, and the previous phrasing was supported by 79% (disagree/strongly disagree: 5.3%). Based on your comments, we revised the statement as follows: “Catalyze clinical translation by generating visible and impactful SDS success stories.”

Do you agree with the revised goal?

| Answer | Count | Percentage |
|---|---|---|
| Strongly Agree | 24 | 60.00% |
| Agree | 16 | 40.00% |
| Neither agree nor disagree | 0 | 0.00% |
| Disagree | 0 | 0.00% |
| Strongly Disagree | 0 | 0.00% |
| Comments | 0 | 0.00% |

**Goal 4.2:** The original phrasing was “Educate medical community about digitalization and data science.” 81.6% considered the goal as important/very important, and the previous phrasing was supported by 84.2% (disagree/strongly disagree: 5.3%). Based on your comments, we revised the statement as follows: “Improve transfer of knowledge between different SDS stakeholders.”

Do you agree with the revised goal?

| Answer | Count | Percentage |
|---|---|---|
| Strongly Agree | 20 | 50.00% |
| Agree | 18 | 45.00% |
| Neither agree nor disagree | 1 | 2.50% |
| Disagree | 1 | 2.50% |
| Strongly Disagree | 0 | 0.00% |
| Comments | 5 | 12.50% |

**Goal 4.3:** The original phrasing was “Ensure high-quality external validation of clinical SDS applications.” 76.3% considered the goal as important/very important, and the previous phrasing was supported by 68.4% (disagree/strongly disagree: 10.5%). Based on your comments, we revised the statement as follows: “Ensure high-quality external validation of SDS applications.”

Do you agree with the revised goal?

| Answer | Count | Percentage |
|---|---|---|
| Strongly Agree | 17 | 42.50% |
| Agree | 18 | 45.00% |
| Neither agree nor disagree | 4 | 10.00% |
| Disagree | 1 | 2.50% |
| Strongly Disagree | 0 | 0.00% |
| Comments | 2 | 5.00% |

**NEW Goal 4.4:** Develop new performance metrics for AI algorithms that measure clinically relevant parameters currently not accounted for in validation studies.

Do you agree with the new goal?

| Answer | Count | Percentage |
|---|---|---|
| Strongly Agree | 16 | 40.00% |
| Agree | 11 | 27.50% |
| Neither agree nor disagree | 9 | 22.50% |
| Disagree | 2 | 5.00% |
| Strongly Disagree | 2 | 5.00% |
| Comments | 10 | 25.00% |

**Goal 4.5 (previous goal 4.4):** The original phrasing was “Create resources for advancing SDS in the clinics.”. 68.4% considered the goal as important/very important, and the previous phrasing was supported by 57.9% (disagree/strongly disagree: 13.2%). Based on your comments, we revised the statement as follows: “Allocate economic, infrastructural and personnel resources within hospitals for SDS.”

Do you agree with the revised goal?

| Answer | Count | Percentage |
|---|---|---|
| Strongly Agree | 21 | 52.50% |
| Agree | 13 | 32.50% |
| Neither agree nor disagree | 5 | 12.50% |
| Disagree | 0 | 0.00% |
| Strongly Disagree | 1 | 2.50% |
| Comments | 7 | 17.50% |

**NEW Goal 4.6:** Build public trust in SDS and boost public enthusiasm to spark patient demand.

Do you agree with the new goal?

| Answer | Count | Percentage |
|---|---|---|
| Strongly Agree | 15 | 37.50% |
| Agree | 17 | 42.50% |
| Neither agree nor disagree | 8 | 20.00% |
| Disagree | 0 | 0.00% |
| Strongly Disagree | 0 | 0.00% |
| Comments | 7 | 17.50% |

**NEW Goal 4.7:** Establish SDS as a career path in hospitals.

Do you agree with the new goal?

| **Answer** | **Count** | **Percentage** |
|---|---|---|
| Strongly Agree | 12 | 30.00% |
| Agree | 20 | 50.00% |
| Neither agree nor disagree | 5 | 12.50% |
| Disagree | 3 | 7.50% |
| Strongly Disagree | 0 | 0.00% |
| Comments | 8 | 20.00% |

**NEW Goal 4.8:** Develop widely accepted concepts for obtaining patient consent to data sharing while considering SDS as a dynamic field with unforeseeable changes in future data usage and application.

Do you agree with the new goal?

| **Answer** | **Count** | **Percentage** |
|---|---|---|
| Strongly Agree | 18 | 45.00% |
| Agree | 15 | 37.50% |
| Neither agree nor disagree | 5 | 12.50% |
| Disagree | 2 | 5.00% |
| Strongly Disagree | 0 | 0.00% |
| Comments | 7 | 17.50% |

**NEW Goal 4.9:** Establish clear and widely accepted liability and medical insurance regulations for data-driven clinical practice, with particular focus on cases of AI failure or human rejection of AI recommendations.

Do you agree with the new goal?

| **Answer** | **Count** | **Percentage** |
|---|---|---|
| Strongly Agree | 11 | 27.50% |
| Agree | 20 | 50.00% |
| Neither agree nor disagree | 6 | 15.00% |
| Disagree | 3 | 7.50% |
| Strongly Disagree | 0 | 0.00% |
| Comments | 7 | 17.50% |
