# Supplementary material for: Surgical Data Science -- from Concepts toward Clinical Translation
Source: arXiv:2011.02284 source file (2021-07-30)
Supplement: Supplementary file 2 [file initiatives.tex]

\section*{\appendixtitleFull}
%\section{Surgical Data Science initiatives}
\label{app:initiatives}

\begin{center}
\tablefirsthead{%
  \toprule
  \multicolumn{1}{l}{Project title} &
  \multicolumn{1}{l}{Description} &
  \multicolumn{1}{l}{Funding source} &
  \multicolumn{1}{l}{Period} &
  \multicolumn{1}{l}{Publication} \\
  \midrule }
\tablehead{%
  \midrule
  \multicolumn{5}{l}{\small\sl continued from previous page} \\
  \toprule
  \multicolumn{1}{l}{Project title} &
  \multicolumn{1}{l}{Description} &
  \multicolumn{1}{l}{Funding source} &
  \multicolumn{1}{l}{Period} &
  \multicolumn{1}{l}{Publication} \\
  \midrule }
\tabletail{%
  \midrule
  \multicolumn{5}{r}{\small\sl continued on next page} \\
  \midrule }
\tablelasttail{}
\topcaption{Surgical Data Science initiatives}
\begin{supertabular}{p{3cm} p{4cm} p{4cm} p{1.5cm} p{3cm}}
Surgical Data Science Initiative &
  Surgical data science aims to improve the quality of interventional healthcare and its   value through the capture, organization, analysis and modelling of data. &
  National Center of Tumor Disease (NCT), German Cancer Research Center (DKFZ) &
  since 2015 &
  Maier-Hein, L. 2017 DOI 10.1038/s41551-017-0132-7; Maier-Hein, L. 2018 arXiv:1806.03184; http://www.surgical-data-science.org/ \\
RONNA &
  Upgradeable robotic neuro-navigation system and open for development under the H2020   SurgIOM project &
  ERDF - European   Regional Development Fund {[}2014-2016{]}, Faculty of Mechanical Engineering and   Naval Architecture, Clinical Hospital Dubrava, Croatian Institute for Brain   Research (Croatian Institute of Technology) {[}2011-2013{]} &
  since 2011 &
  Jerbić et al.   2020; Dlaka et al. 2017 \\
Tomorrow’s health Territory - Investment of the future program “Innovative Territory” &
  Innovations for healthcare (real-time access to data, telemedicine, deployment of e-health; Set up of regional digital platform to develop innovative e-health services. &
  Priesm, Better, IHU &
  2020-2024 &
   \\
ARAILIS - Augmented Reality and Artificial Intelligence &
  Research soft-tissue navigation and visualization based on AI-assisted methods &
   &
   &
   \\
supported Laparoscopic Imagery in Surgery &
&
  Sächsische Aufbaubank (SAB) &
  2020-2023 &
   \\
CeTI - Centre for Tactile Internet with Human-in-the-Loop &
  Research   robot-assisted surgery: Prediction of surgical actions for human-machine collaboration and sensor-based surgical training.  &
  German Research Foundation (DFG), EXC 2050/1 &
  2019-2025 &
   \\
CoBot - Colorectal robotic assistant for laparoscopic surgery &
  Research  robot-assisted surgery: Development of context-aware assistance functions for colorectal surgeries &
  Else Kröner   Fresenius Center for Digital Health &
  2019-2021 &
   \\
   SurgOmics &
   Prediction of adverse events in surgery based on the AI-based analysis of process features &
   Federal Ministry of Health (BMG) &
   2020 - 2023 &
   \\
BOOSTER &
  Developing   personalized medicine for strokes in emergency situations to provide faster   and better emergency care to a larger number of stroke victims. &
  INSA INRIA &
  2019-2024 &
   \\
IamRONNA   - Intelligent Autonomous Mobile RONNA &
  Development of   an autonomous omnidirectional mobile platform equipped with a propulsion   system, 3D vision and laser sensors for application to other medical devices   as well as to other tasks within operating rooms and hospital spaces. &
  Adris Foundation &
  2019-2021 &
   \\
CRTA   - Regional Center of Excellence for Robotic Technologies &
  Operating   theatre specialized for neurosurgical applications but also for general   surgery. Validation of concepts of the SurgIOM for neurosurgery and for   sensorization of laparoscopic instruments. &
  ERDF - European   Regional Development Fund &
  2018-2021 &
   \\
Augmented   Reality Surgical System iSurgeon &
  Medical and   technical experts with experience in computer-assisted surgery identified   four research areas with a high potential for sustainably improving surgical   oncology: (1) functional imaging based on biophotonics, (2) multimodal data   visualization through augmented reality, (3) reproducible imaging by means of   robotics, and (4) context-aware visualization based on surgical data science. &
  Federal Ministry   for Economic Affairs and Energy (BMWi) &
  2018-2020 &
  Maier-Hein, L.,   Gockel, I., Speidel, S. et al. Intraoperative Bildgebung und Visualisierung.   Onkologe 26, 31–43 (2020). https://doi.org/10.1007/s00761-019-00695-4 \\
NERO   - Neurosurgical Robot &
  Development of   head phantoms and base frames for stereotactic neurosurgery. &
  ERDF - European   Regional Development Fund &
  2017-2021 &
   \\
OP 4.1 Smart Services II &
  Concept for the   design of a platform to bring apps (software innovation) into the operating   room. &
  Federal Ministry   for Economic Affairs and Energy (BMWi) &
  08/2017-02/2020 &
  OP 4.1: A   User-Centered Platform for the Operation Room of the Future K. März, L.   Mündermann, M. Nolden, T. Simpfendörfer, C. Gasch, T. Ross, S. Onogur, J.   Metzger, C. Feldmann, J. Fallert, M. Hohenfellner, L. Maier-Hein {[}IPCAI 2019{]} \\
FastPath   - Innovative pathways for minimally invasive surgery patients &
  Innovative   patient care pathways adapted to image guided minimally invasive surgery and   methods measure relevant patient and health economics outcomes. &
  IHU, Medtronic &
  01/2016-01/2021 &
   \\
DeepSurg   - ANR JCJC - National Project &
  AI/DL methods   for the analysis of clinical activities in hybrid procedures using multiple   RGBD ceiling-mounted cameras &
  UNISTRA, IHU &
  2016-2021 &
   \\
CONDOR - Connected Optimized Network \& Data in Operating Rooms. Video standards   \& infra-structure in Operating Room &
  Video standard   and infrastructure for the recording and live streaming of surgical data and   metadata. Computer vision tools for the analysis of surgery &
  BPI France, IHU,   UNISTRA &
  10/2016-09/2020 &
   \\
InnOPlan,   Smart Data Technologies &
  Concepts for   connecting devices and IT-Systems and resulted in a smart data platform. &
  BMWi &
  01/2015-03/2018 &
   \\
ACRON   - A new concept of Applied Cognitive RObotics in clinical Neuroscience &
  Novel algorithms   (Šuligoj et al. 2017; 2018) for precise patient localization in neurosurgery   from the ACRON project will be used in the SurgIOM project for maximally   automating certain steps of the neurosurgical procedure. &
  Croatian Science   Foundation (HRZZ) &
  2014-2018 &
   \\
Endoscopy meets computer science: Precise navigation for minimally-invasive surgery &
   &
  Klaus Tschira Stiftung &
  2014-2016 &
   \\
DFG Collaborative Research Project (SFB) 125: Cognition-guided surgery:    “Knowledge-based navigated liver surgery” &
   &
  Deutsche Forschungsgemeinschaft (DFG) &
  07/2012-06/2017 &
   \\
DFG   Research Training Group 1126: Intelligent Surgery: “Planning and navigation   in ablation therapy” (PI) &
   &
  DFG &
  06/2012-03/2014 &
   \\
DFG   Research Training Group 1126: Intelligent Surgery: “Navigated liver   resection” (PI) &
   &
  DFG &
  06/2012-03/2014 &
   \\
OR.NET   - Secure dynamic networking in the operating room and clinic &
  Cross-vendor   concepts and standards (IEEE 11073 SDC) for the dynamic and secure networking   of medical devices and IT systems in the OR and in clinics. &
  BMBF &
  09/2012-04/2016 &
   \\
X-RAIS &
  AI tool for the   analysis of medical images based on neural networks and Radiomics techniques. &
  SRY &
   &
   \\
Smart   Image &
  The advent of   laparoscopic cholecystectomy almost 30 years ago would change forever the way   surgeons visualize and interact with target anatomy Patients continue to   benefit from different yet related image guided therapies that also allow   access to pathology by minimally invasive means.  As we continue to   depend upon images to guide and inform patient interventions it is   instructive to review the advances made in surgical visualization over its   recent history and look forward to issues that will need to be addressed   toward optimization of interventional visualization.  These issues will   be reviewed from the perspective of a clinician,  not a computer scientist   nor a physicist, with attention also paid to the often neglected topics of   ergonomics and human factors considerations in surgical visualization. &
   &
   &
   \\
OR Black Box: using data to improve surgical safety &
  OR Black Box aims to improve patient safety and outcomes by characterizing intraoperative errors, events, and distractions which allows better surgical coaching and improvements. This product records synchronized data of multiple sensor feeds in the OR such as the video of the surgical scene, audio of the conversations among the surgical team, patient vital signs, feedback from electronic surgical instruments, and analyses the recorded data to provide comprehensive, objective, and clinically relevant insights into the perioperative environment. &
   &
  2017 &
  M. G. Goldenberg, J. Jung, and T. P. Grantcharov, “Using Data to Enhance Performance and Improve Quality and Safety in Surgery,” JAMA Surg., vol. 152, no. 10, pp. 972–973, 01 2017, doi: 10.1001/jamasurg.2017.2888.\newline
  J. J. Jung, P. Jüni, G.   Lebovic, and T. Grantcharov, “First-year Analysis of the Operating Room Black   Box Study,” Ann. Surg., vol. 271, no. 1, pp. 122–127, 2020, doi:   10.1097/SLA.0000000000002863.\\
AI4OR,   A Network Initiative for Context-Aware Operating Theaters &
  Create   innovative solutions to context-awareness in operating theaters, with a   particular focus on surgical process modeling, analysis and recognition of   surgical processes, and cognitive surgical robotics, primarily using AI algorithms &
   &
  since 2018 &
   \\
Multidisciplinary Computational Anatomy (MCA) &
  Multidisciplinary Computational Anatomy (MCA) supported by the Japan MEXT grant has been   established to integrate the medical images with information along four axes such as time, space, function and pathology. MCA model is a prediction model of those information with medical images. MCA-based medicine with AI is one of the solutions to solve the difficulties of current medical problems. &
   &
  since 2017 &
   \\
SAGES AI Taskforce &
   &
   &
   &
   \\
CARSS Initiative &
   &
   &
   &
   \\
SAGES Video Annotation Consensus Conference &
   &
   &
   &
   \\
\bottomrule
\end{supertabular}
\label{tab:initiatives}
\end{center}
