# Supplementary material for: Surgical Data Science -- from Concepts toward Clinical Translation
Source: arXiv:2011.02284 source file (2021-07-30)
Supplement: Supplementary file 3 [file questionnaire.tex]

\section*{\appendixtitleFull}
%\section{Questionnaire}
\label{app:questionnaire}

\begin{center}
%\sffamily\small
\tablefirsthead{%
  \toprule
  \multicolumn{1}{l}{ID} &
  \multicolumn{1}{l}{Question} \\
  \midrule }
\tablehead{%
  \midrule
  \multicolumn{2}{l}{\small\sl continued from previous page} \\
  \toprule
  \multicolumn{1}{l}{ID} &
  \multicolumn{1}{l}{Question} \\
  \midrule }
\tabletail{%
  \midrule
  \multicolumn{2}{r}{\sffamily\small\sl continued on next page} \\
  \midrule }
\tablelasttail{}
\topcaption{Questions along with the workshop registration form.}
\sffamily\small
\begin{supertabular}{p{0.6cm} p{14cm}}
\multicolumn{2}{l}{General information} \\
\midrule
Q01 &
What is your background?\newline
Options (multiple selections allowed):
\begin{itemize}
\item Academic: Clinical
\item Academic: Engineering
\item Clinical
\item Industrial
\item Other
\end{itemize}
\\
Q02 &
What is your role?\newline
Options (single selection):
\begin{itemize}
\item Board member/member of organizing committee
\item Professor/Academic group leader
\item Industry
\item PhD Student
\item Undergraduate
\item Postdoc
\item Other
\end{itemize}
\\
Q03 &
Do you want to be acknowledged in a publication of the workshop results?\newline
Options: Yes or No
\\
Q04 &
What is your main incentive for registration to the workshop?\newline
Options (single selection and/or free text):
\begin{itemize}
\item Learning about SDS
\item Meeting SDS experts/networking
\item Advancing the field
\item Being part of the upcoming paper
\item Other (please specify)
\end{itemize}
\\ \midrule
\multicolumn{2}{l}{Successes related to Surgical Data Science}
\\ \midrule
Q05 &
Please name a prominent surgical data science \enquote{success story} (e.g. a clinical application that has been shown to benefit from surgical data science or new insights that were generated based on surgical data science techniques). Describe what you mean by success in this case.
\\
Q06 &
Which research paper in the field of surgical data science has impressed you the most so far?
\\ \midrule
\multicolumn{2}{l}{Challenges related to Surgical Data Science}
\\ \midrule
Q07 &
What are the most critical challenges related to exploiting the potential of surgical data science?
\\
Q08 &
What is lacking in the existing public data sets?
\\
Q09 &
What do you consider as the most urgent issue/problem that needs to be discussed in the workshop (e.g. standards)?
\\ \midrule
\multicolumn{2}{l}{Future of Surgical Data Science}
\\ \midrule
Q10 &
Please list at least one surgical data science (clinical) application that can be regarded as a (relatively) low hanging fruit (i.e. could be addressed in a relatively short period of time).
\\
Q11 &
What should be the next SDS challenge (open competition)?
\\ \midrule
\multicolumn{2}{l}{Personal experience with Surgical Data Science}
\\ \midrule
Q12 &
What public data set have you found the most useful for your research in SDS so far?
\\
Q13 &
What was your biggest failure in SDS, even though it looked promising at the beginning, to avoid others making the same mistake?
\\
Q14 &
What is your advice for avoiding these problems?
\\ \midrule
\multicolumn{2}{l}{Joint Surgical Data Science Project}
\\ \midrule
Q15 &
Would you be interested to work on a joint surgical data science project with other workshop attendees?
\\
Q16 &
Do you (potentially) have data to contribute to such a project?
\\
Q17 &
If yes, what kind of data?
\\ \midrule
\multicolumn{2}{l}{Where do we stand?}
\\ \midrule
Q18 &
What do you regard as the most important developments in the field since the last workshop in June 2016?
\\
Q19 &
Surgical Data Science failures: Are you aware of projects that have failed (optionally and preferably: name them)?
\\
Q20 &
What was the (main) reason for failure?
\\
\bottomrule
\end{supertabular}
\label{tab:questionnaire}
\end{center}
