# Supplementary material for: Surgical Data Science -- from Concepts toward Clinical Translation
Source: arXiv:2011.02284 source file (2021-07-30)
Supplement: Supplementary file 4 [file questionnaireResults.tex]

\section*{\appendixtitleFull}
%\section{Results of questionnaire}
\label{app:questionnaireResults}

\subsection{General information}

\noindent \newline \textit{\textbf{Q01:} What is your background?}

\begin{figure}[pos=h]
  \begin{subfigure}[c]{0.4\textwidth}
    \includegraphics[width=\textwidth, trim=4cm 1cm 4cm 1cm, clip]{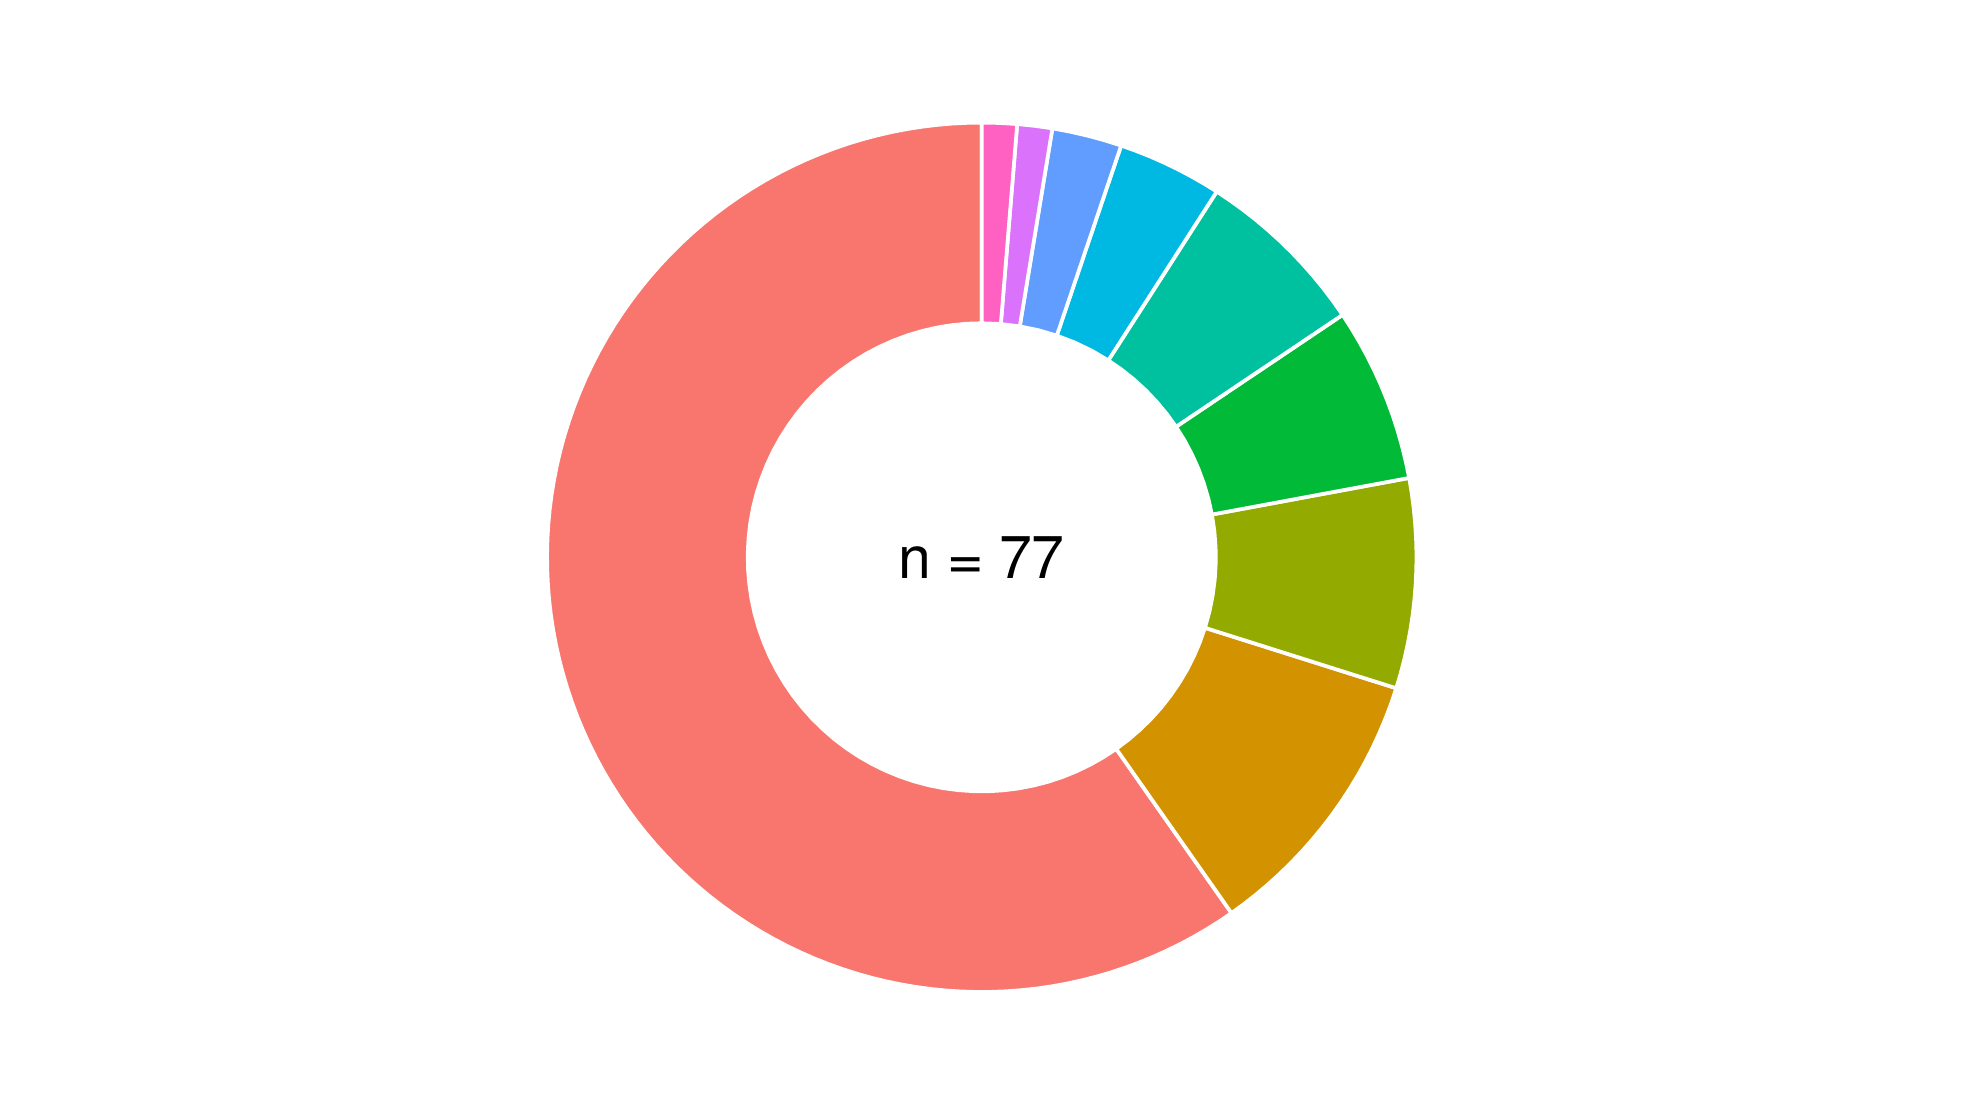}
  \end{subfigure}
  \hfill
  \begin{subfigure}[c]{0.59\textwidth}
    \includegraphics[height=5cm, trim=4.5cm 2cm 0cm 2cm, clip]{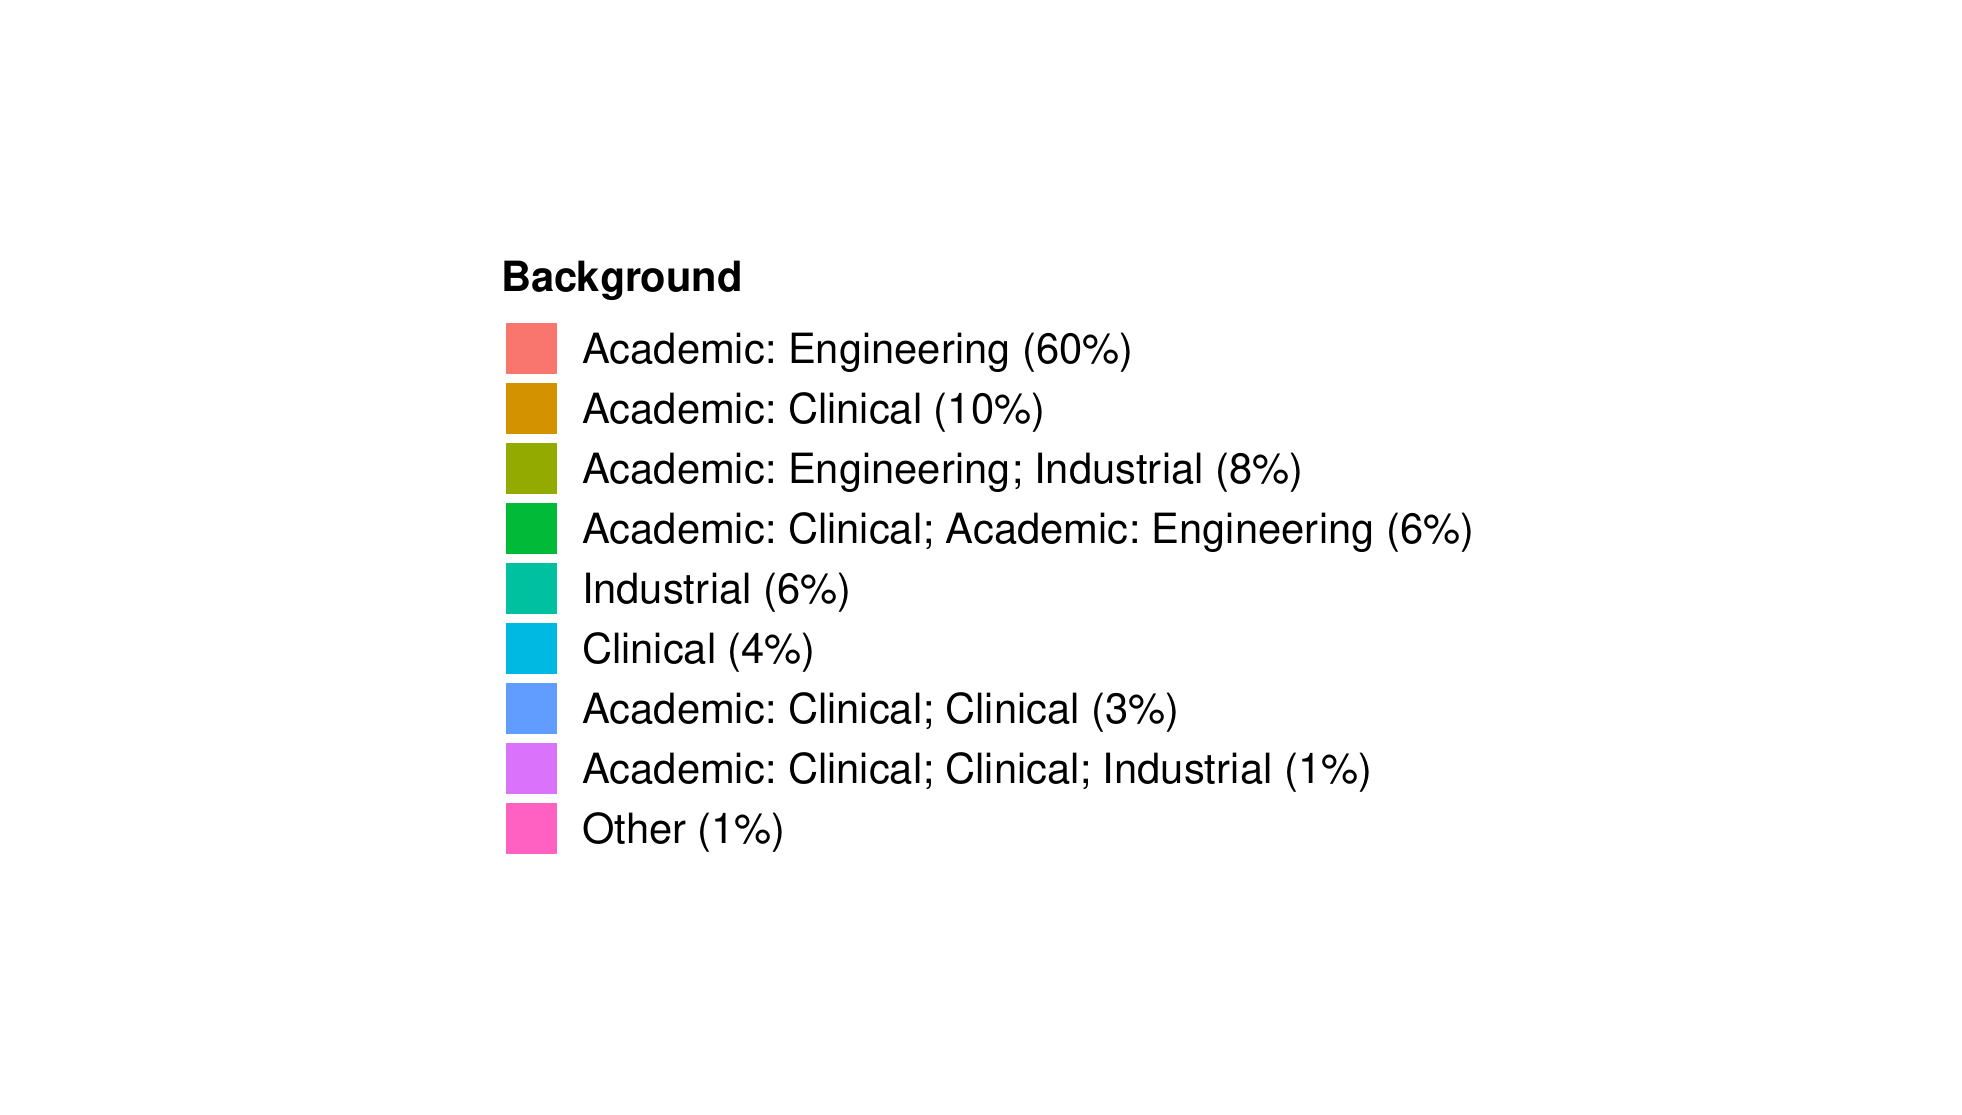}
  \end{subfigure}
\end{figure}

\noindent \textit{\textbf{Q02:} What is your role?}

\begin{figure}[pos=h]
  \begin{subfigure}[c]{0.4\textwidth}
    \includegraphics[width=\textwidth, trim=4cm 1cm 4cm 1cm, clip]{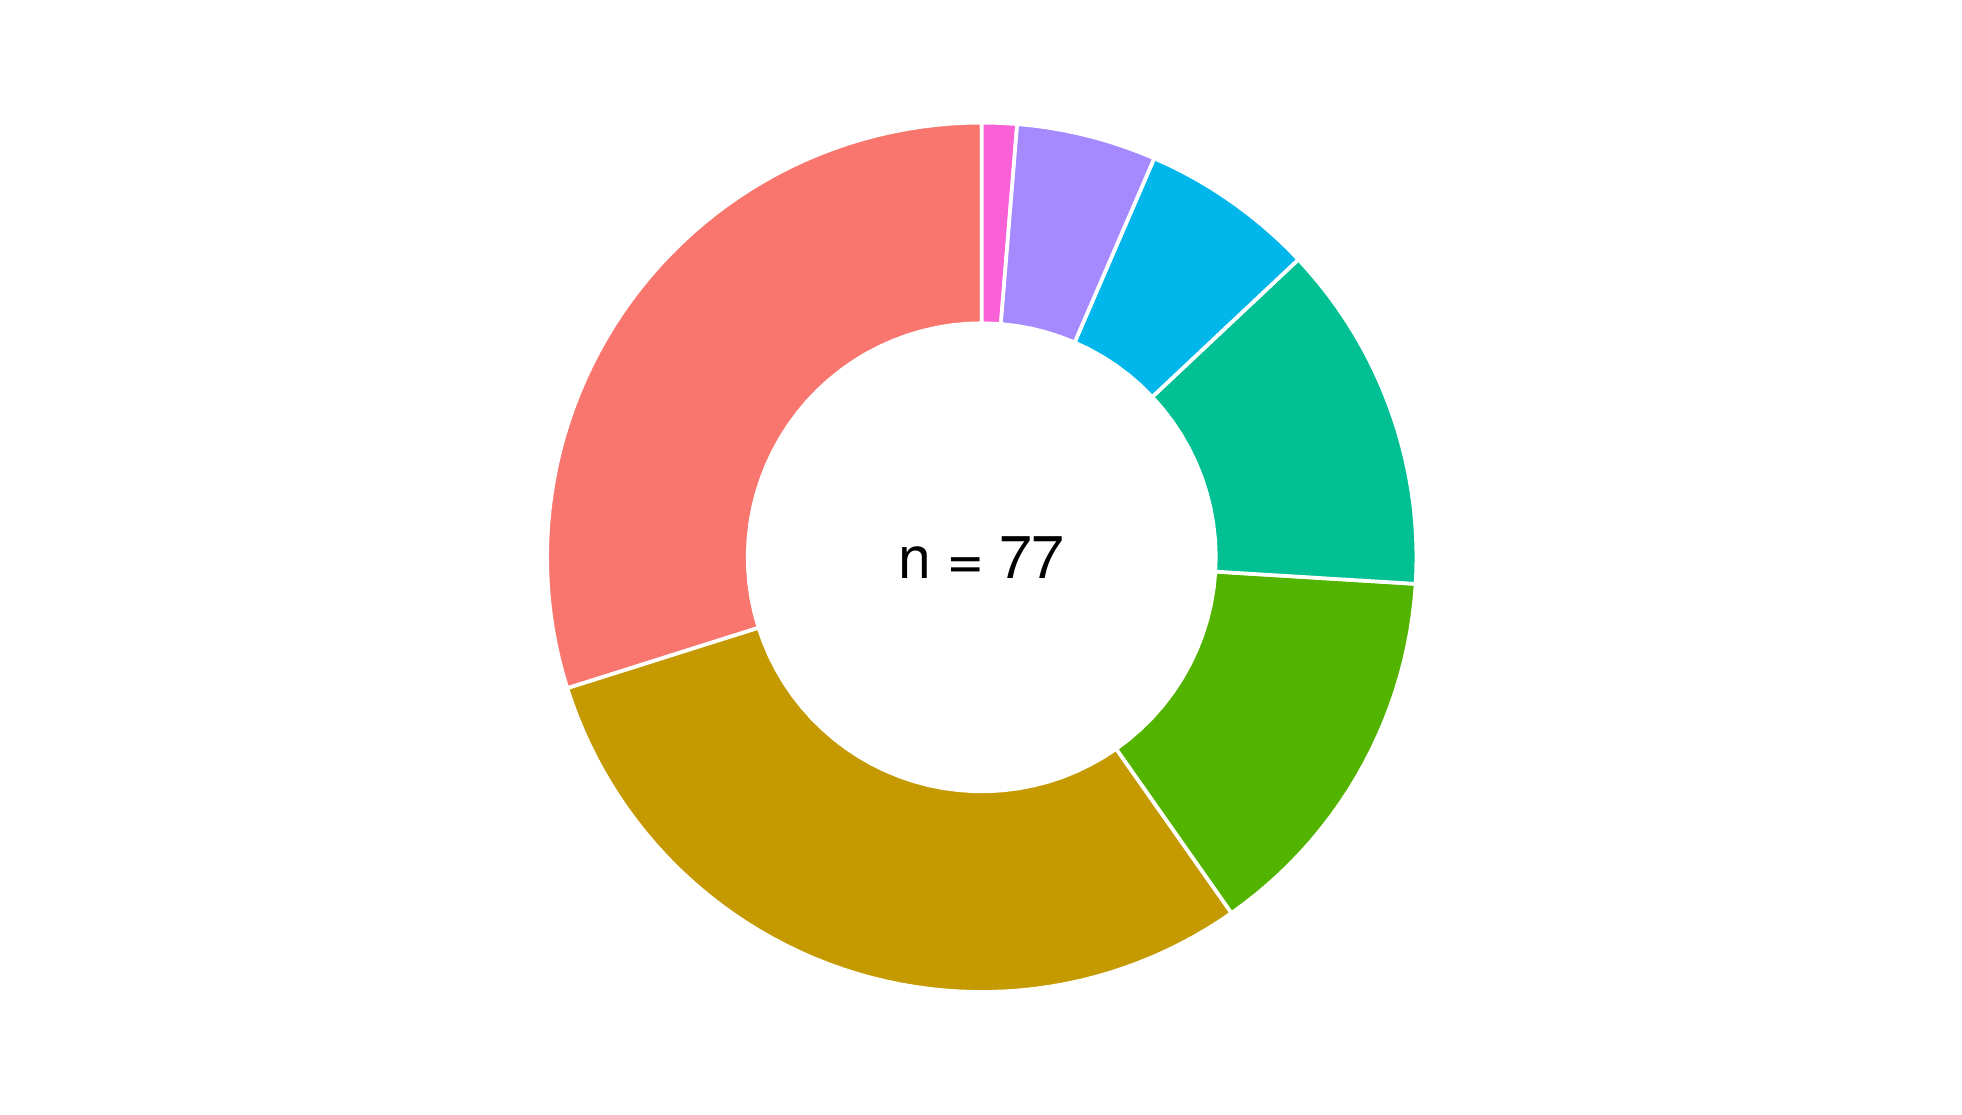}
  \end{subfigure}
  \hfill
  \begin{subfigure}[c]{0.59\textwidth}
    \includegraphics[height=5cm, trim=4cm 2cm 0cm 2cm, clip]{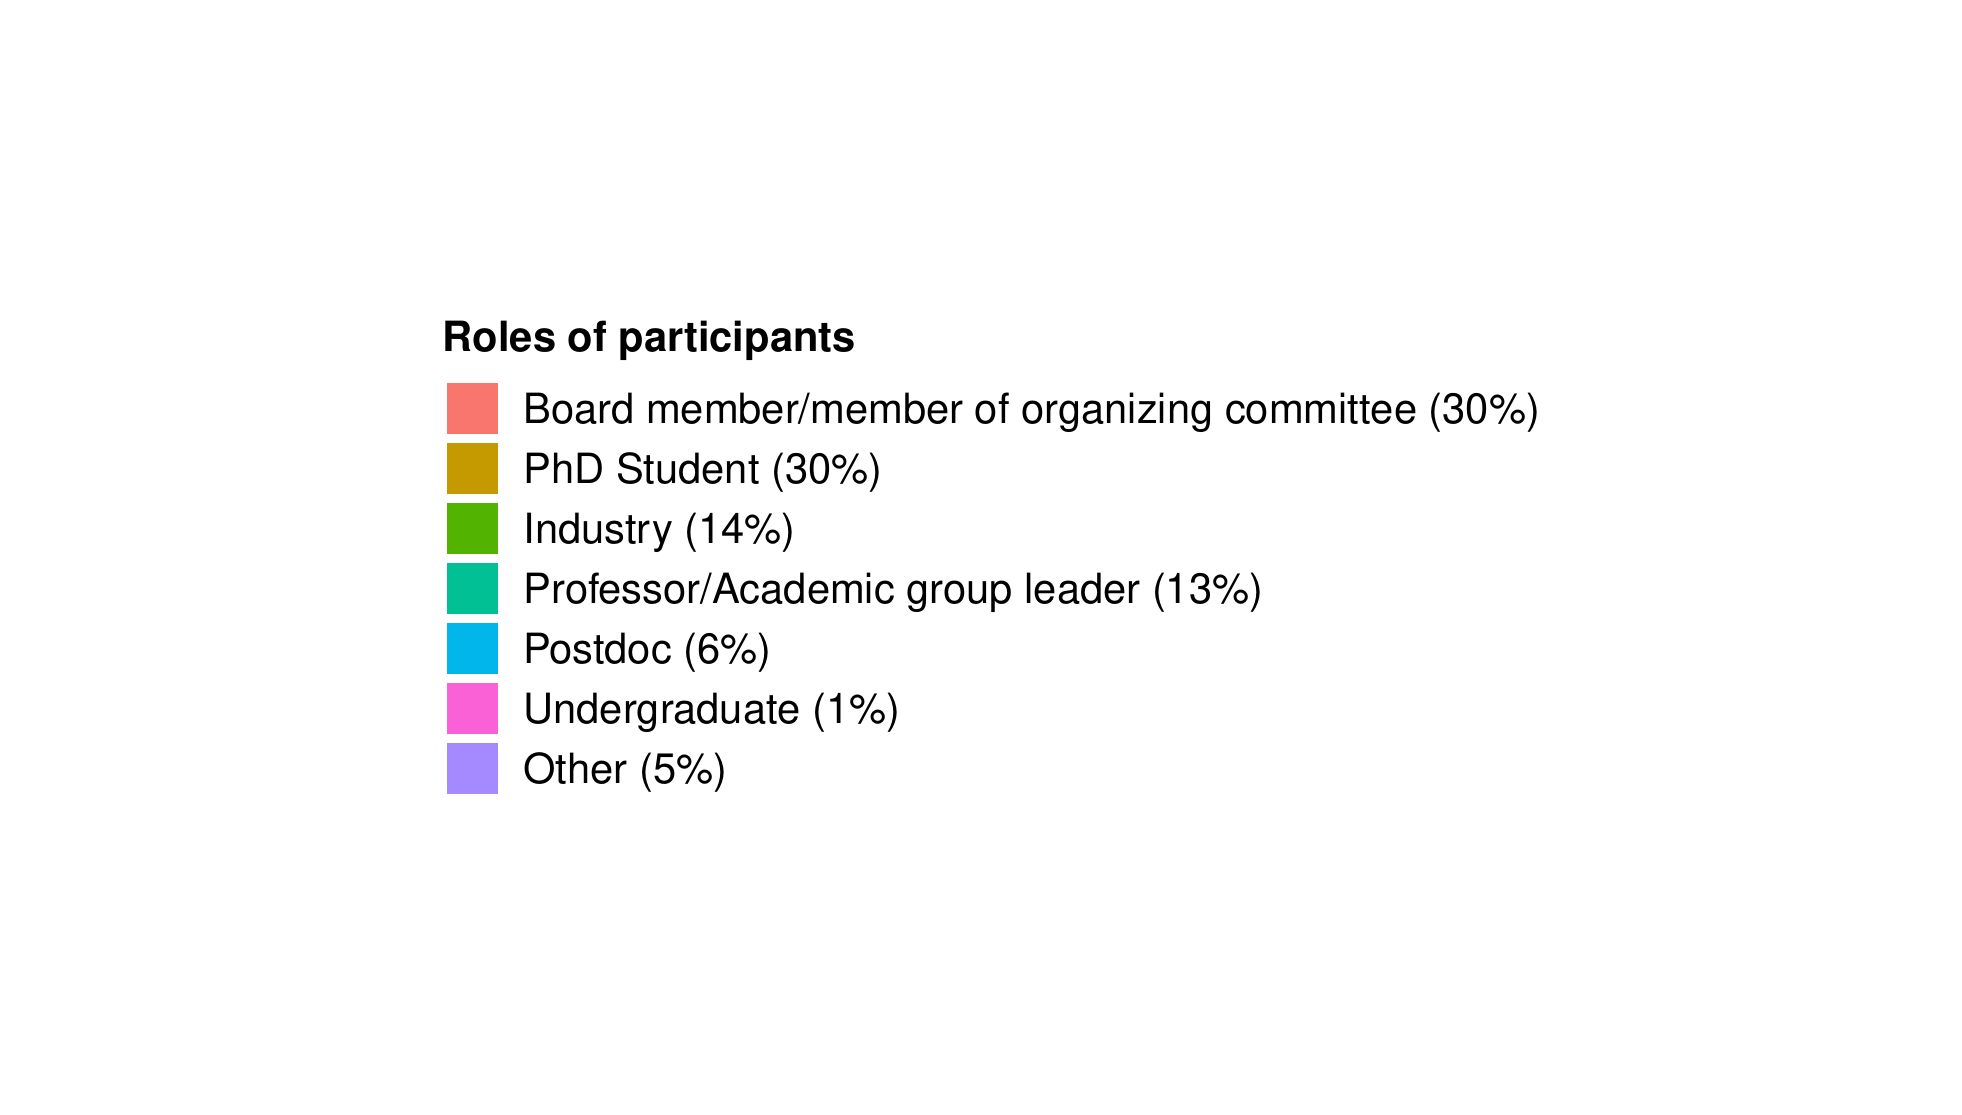}
  \end{subfigure}
\end{figure}

\noindent \textit{\textbf{Q03:} Do you want to be acknowledged in a publication of the workshop results?}

\begin{figure}[pos=h]
  \begin{subfigure}[c]{0.4\textwidth}
    \includegraphics[width=\textwidth, trim=4cm 1cm 4cm 1cm, clip]{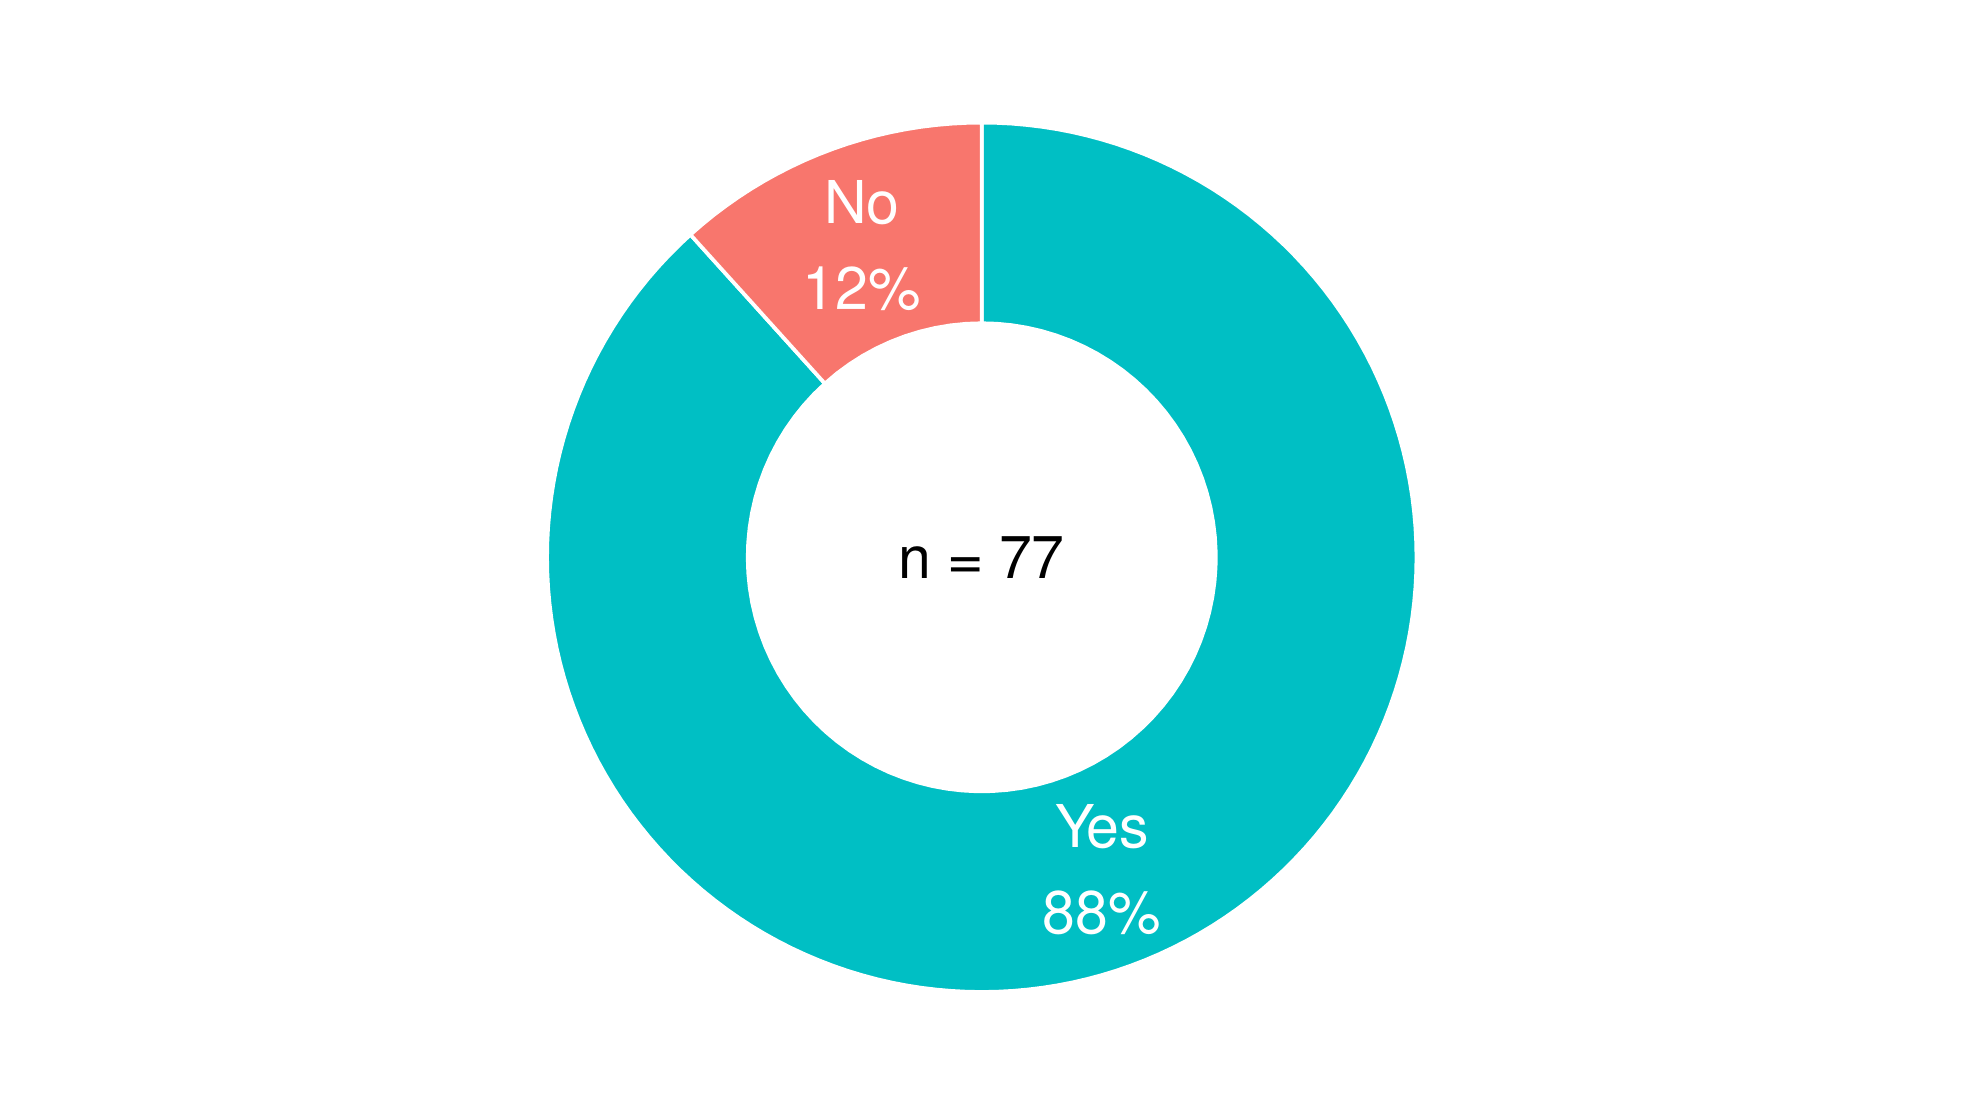}
  \end{subfigure}
  \hfill
  \begin{subfigure}[c]{0.59\textwidth}
    \includegraphics[height=5cm]{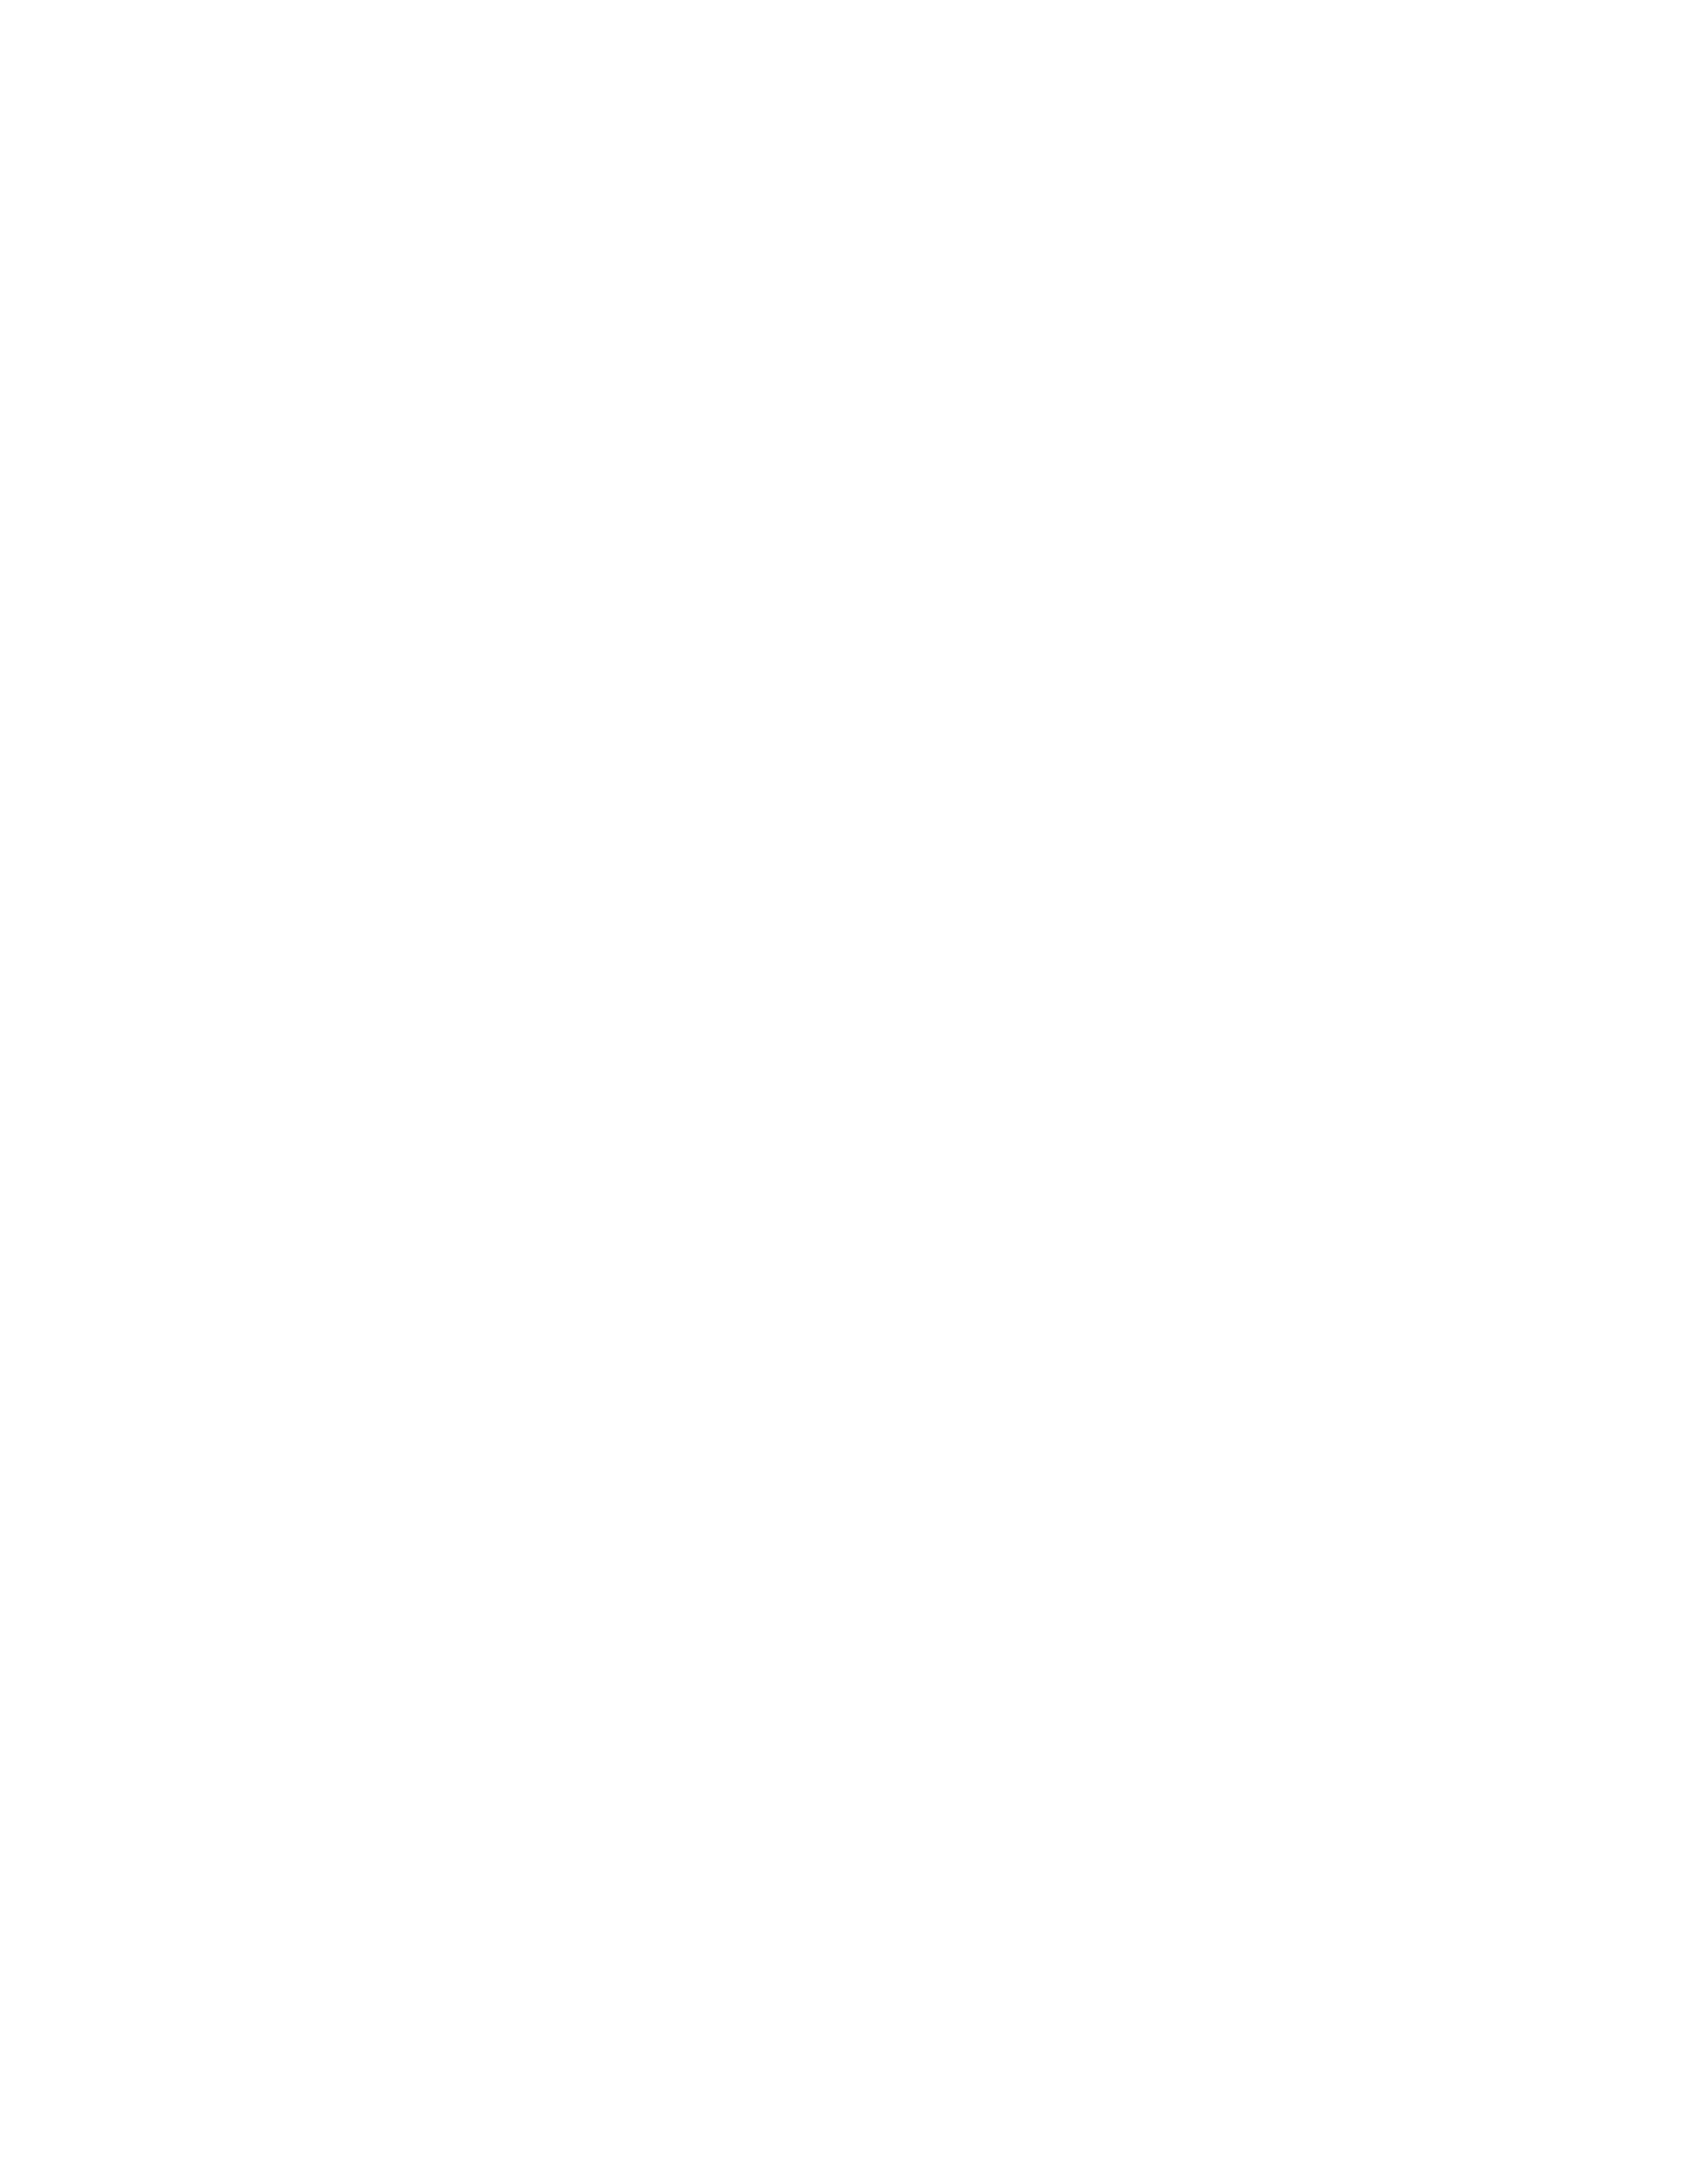}
  \end{subfigure}
\end{figure}

\newpage
\noindent \textit{\textbf{Q04:} What is your main incentive for registration to the workshop?}

\begin{figure}[pos=h]
  \begin{subfigure}[c]{0.4\textwidth}
    \includegraphics[width=\textwidth, trim=4cm 1cm 4cm 1cm, clip]{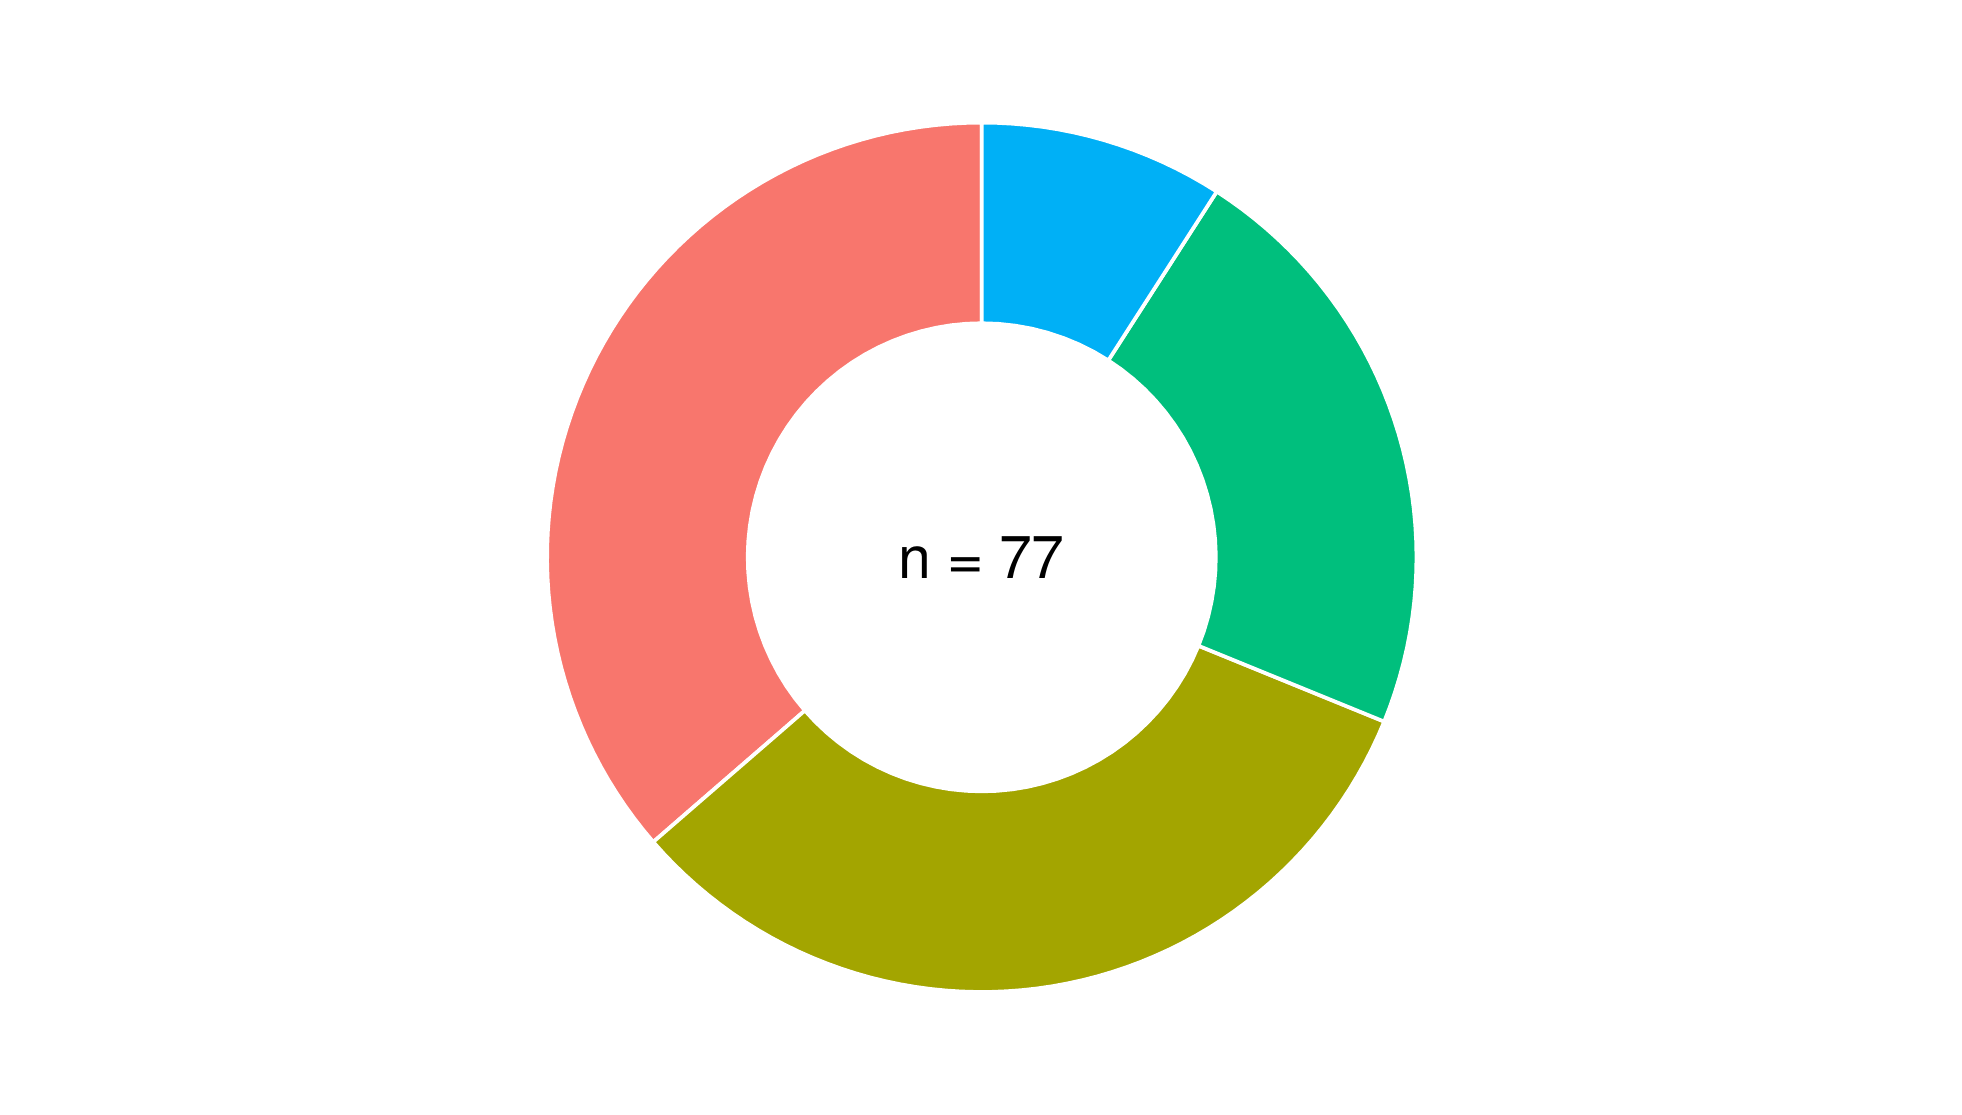}
  \end{subfigure}
  \hfill
  \begin{subfigure}[c]{0.59\textwidth}
    \includegraphics[height=5cm, trim=5.5cm 2cm 0cm 2cm, clip]{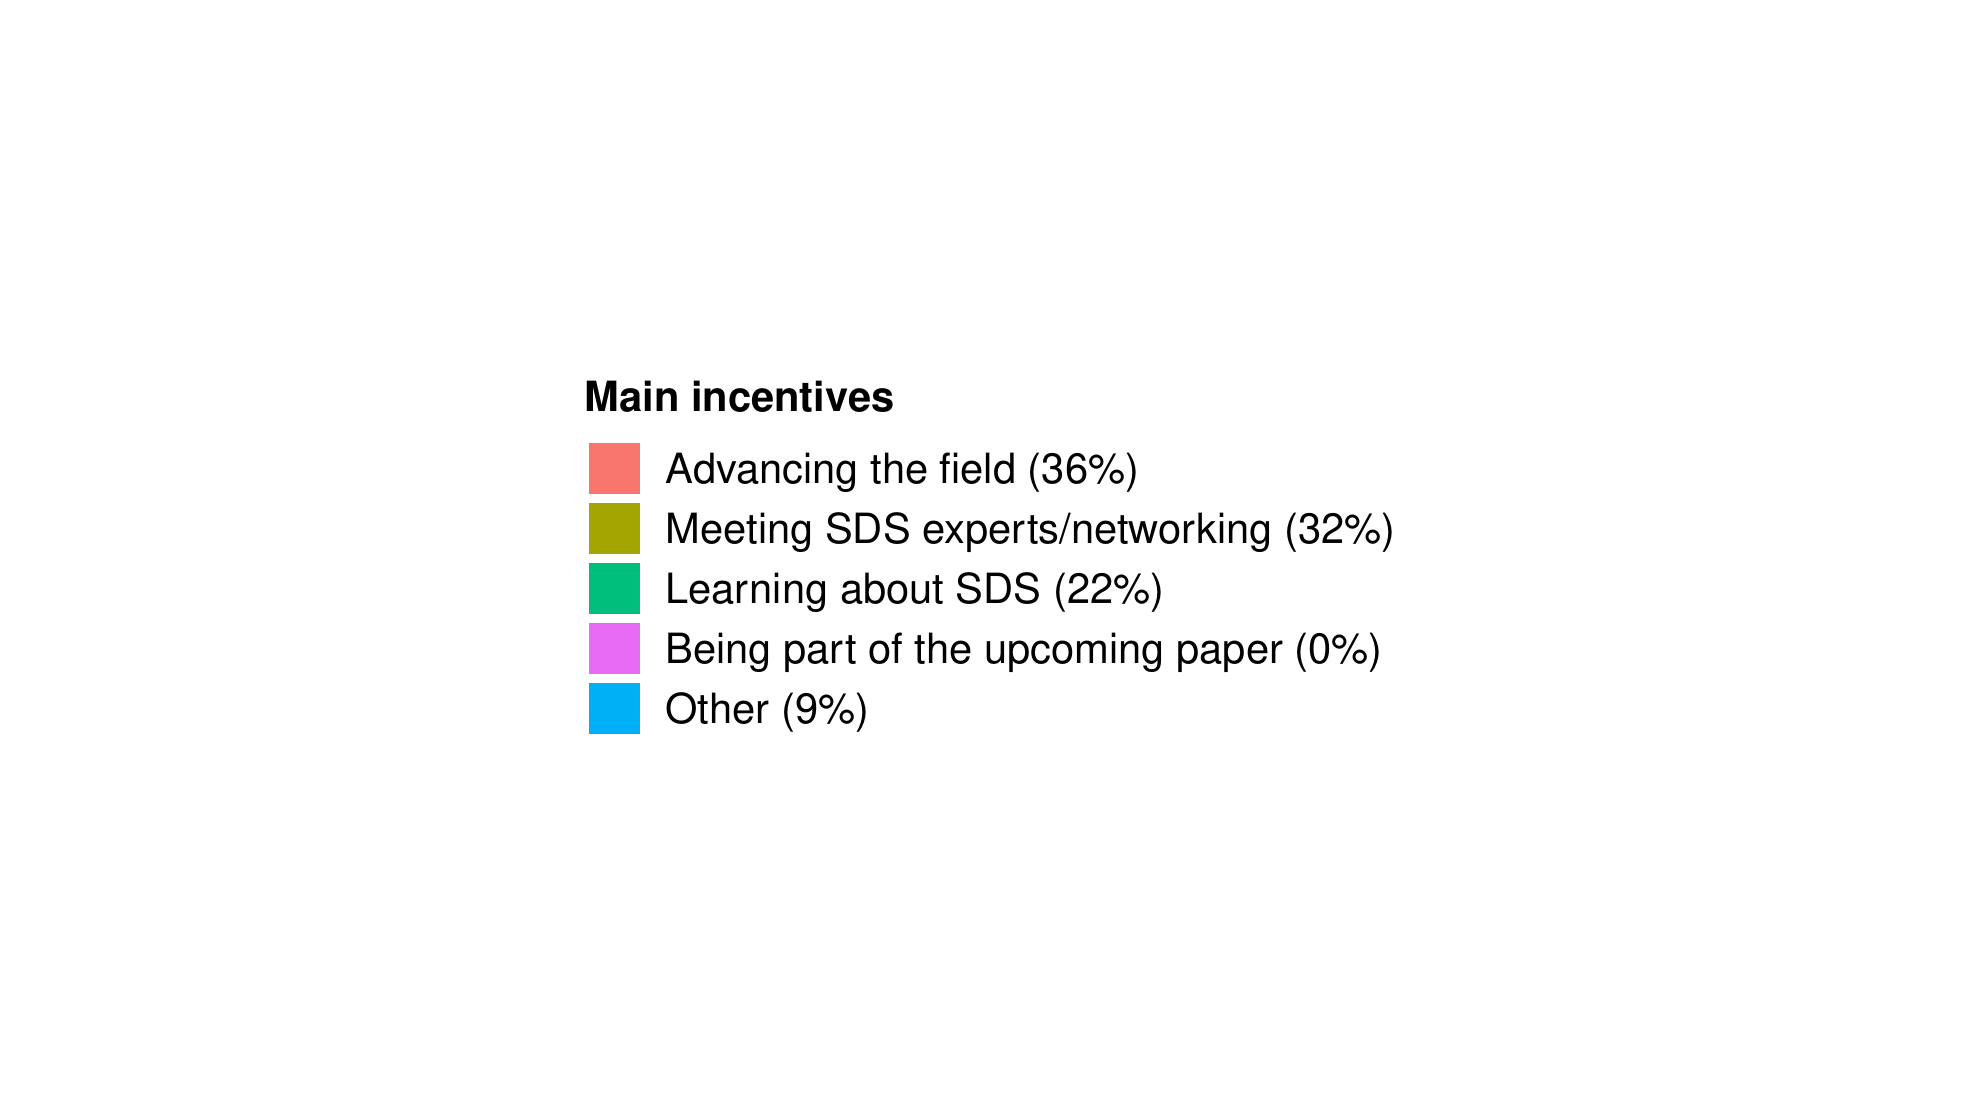}
  \end{subfigure}
\end{figure}

\subsection{Successes related to Surgical Data Science}

\noindent \newline \textit{\textbf{Q05:} Please name a prominent surgical data science \enquote{success story} (e.g. a clinical application that has been shown to benefit from surgical data science or new insights that were generated based on surgical data science techniques). Describe what you mean by success in this case.}

\noindent \newline 87\% of participants responded to this question. 81 partial replies were extracted from the free text and categorized. Of these, 68\% named projects, systems, and (fields of) applications in different levels of detail. The most prominent project is the OR Black Box led by \citeappendix{appendix:goldenberg_using_2017} (7 mentions). Surgical workflow analysis is the most promising field of application (4 mentions), followed by the work of the \citeappendix{appendix:camma_camma_nodate} group (3 mentions). 9\% mentioned that they were not aware of any success story. Participants were also struggling with the definition of a \enquote{success story} in the field of surgical data science and came up with definitions of what success is in their understanding (17\%).

\begin{figure}[pos=h]
  \begin{subfigure}[c]{0.4\textwidth}
    \includegraphics[width=\textwidth, trim=4cm 1cm 4cm 1cm, clip]{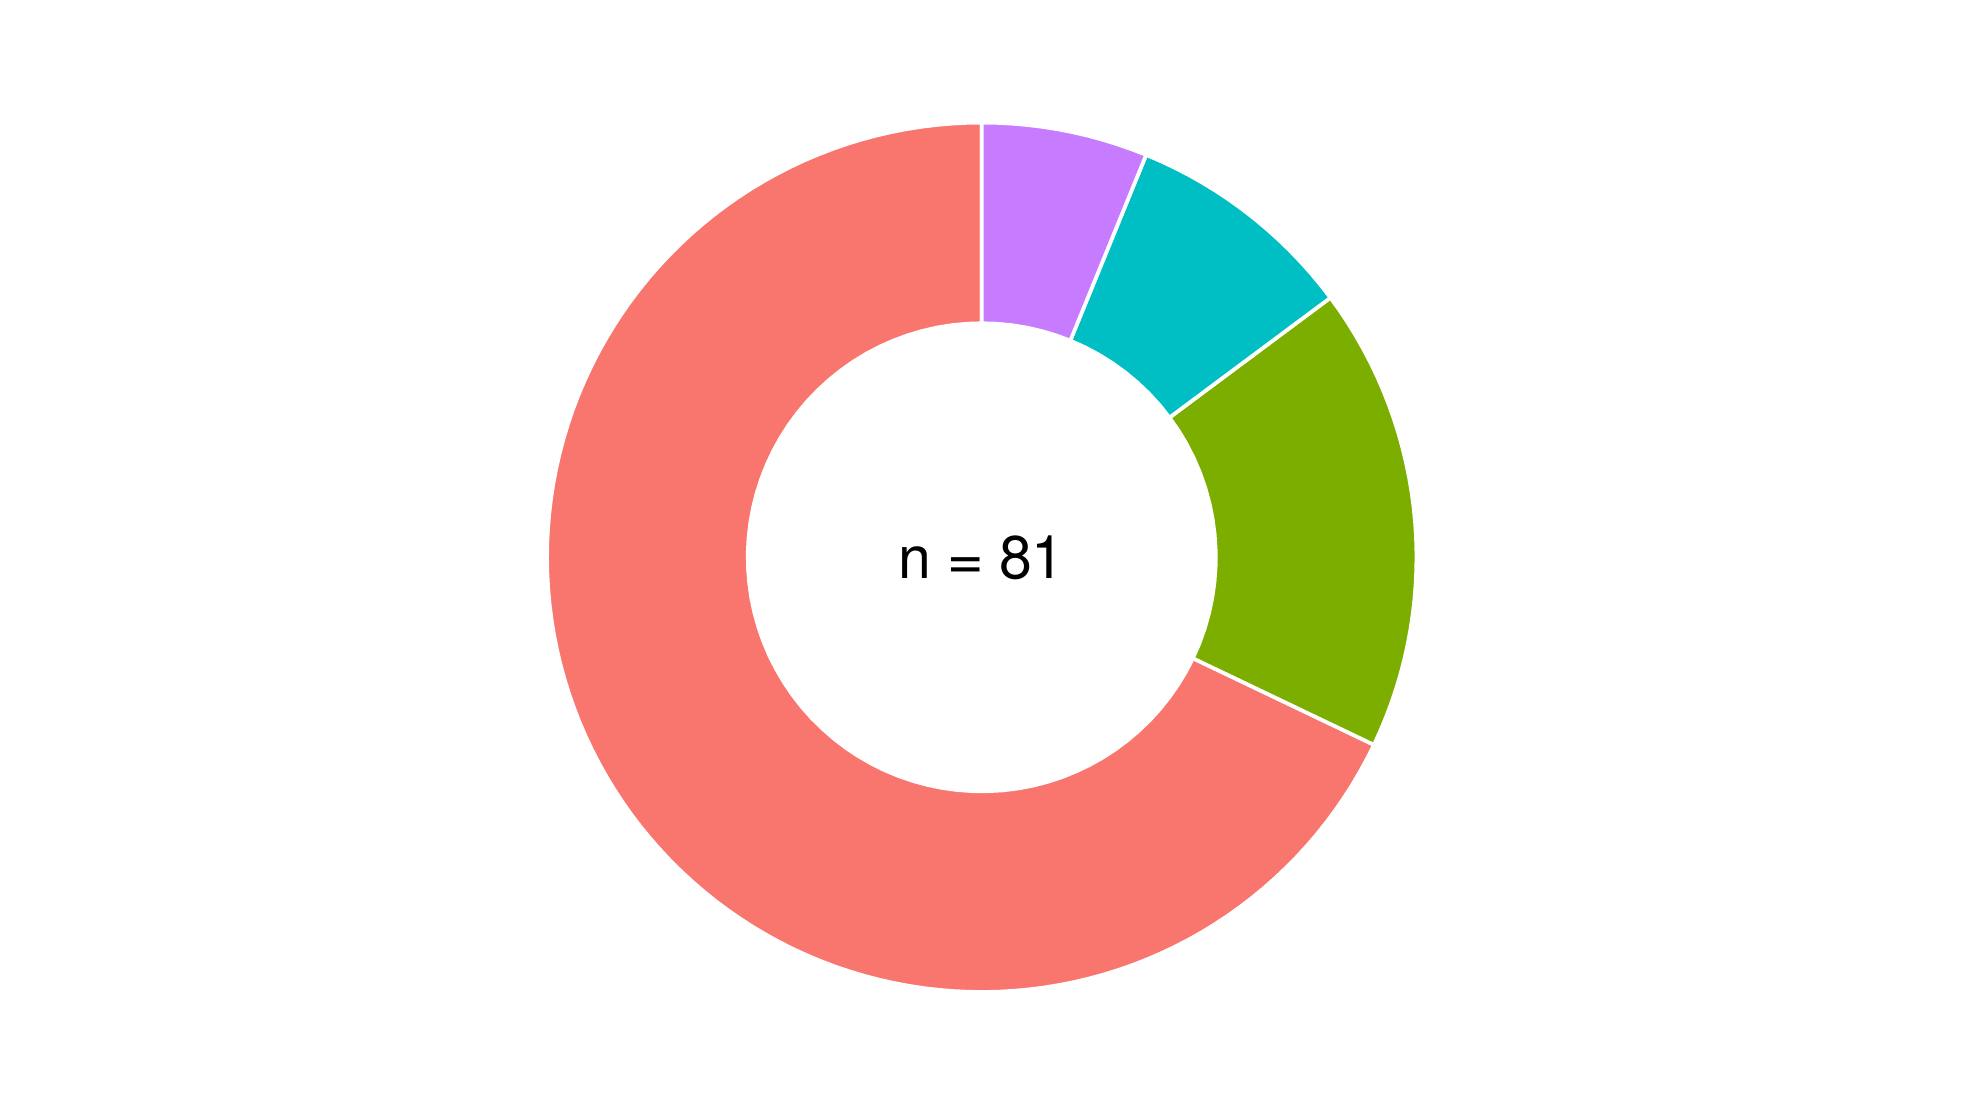}
  \end{subfigure}
  \hfill
  \begin{subfigure}[c]{0.59\textwidth}
    \includegraphics[height=5cm, trim=5.5cm 2cm 0cm 2cm, clip]{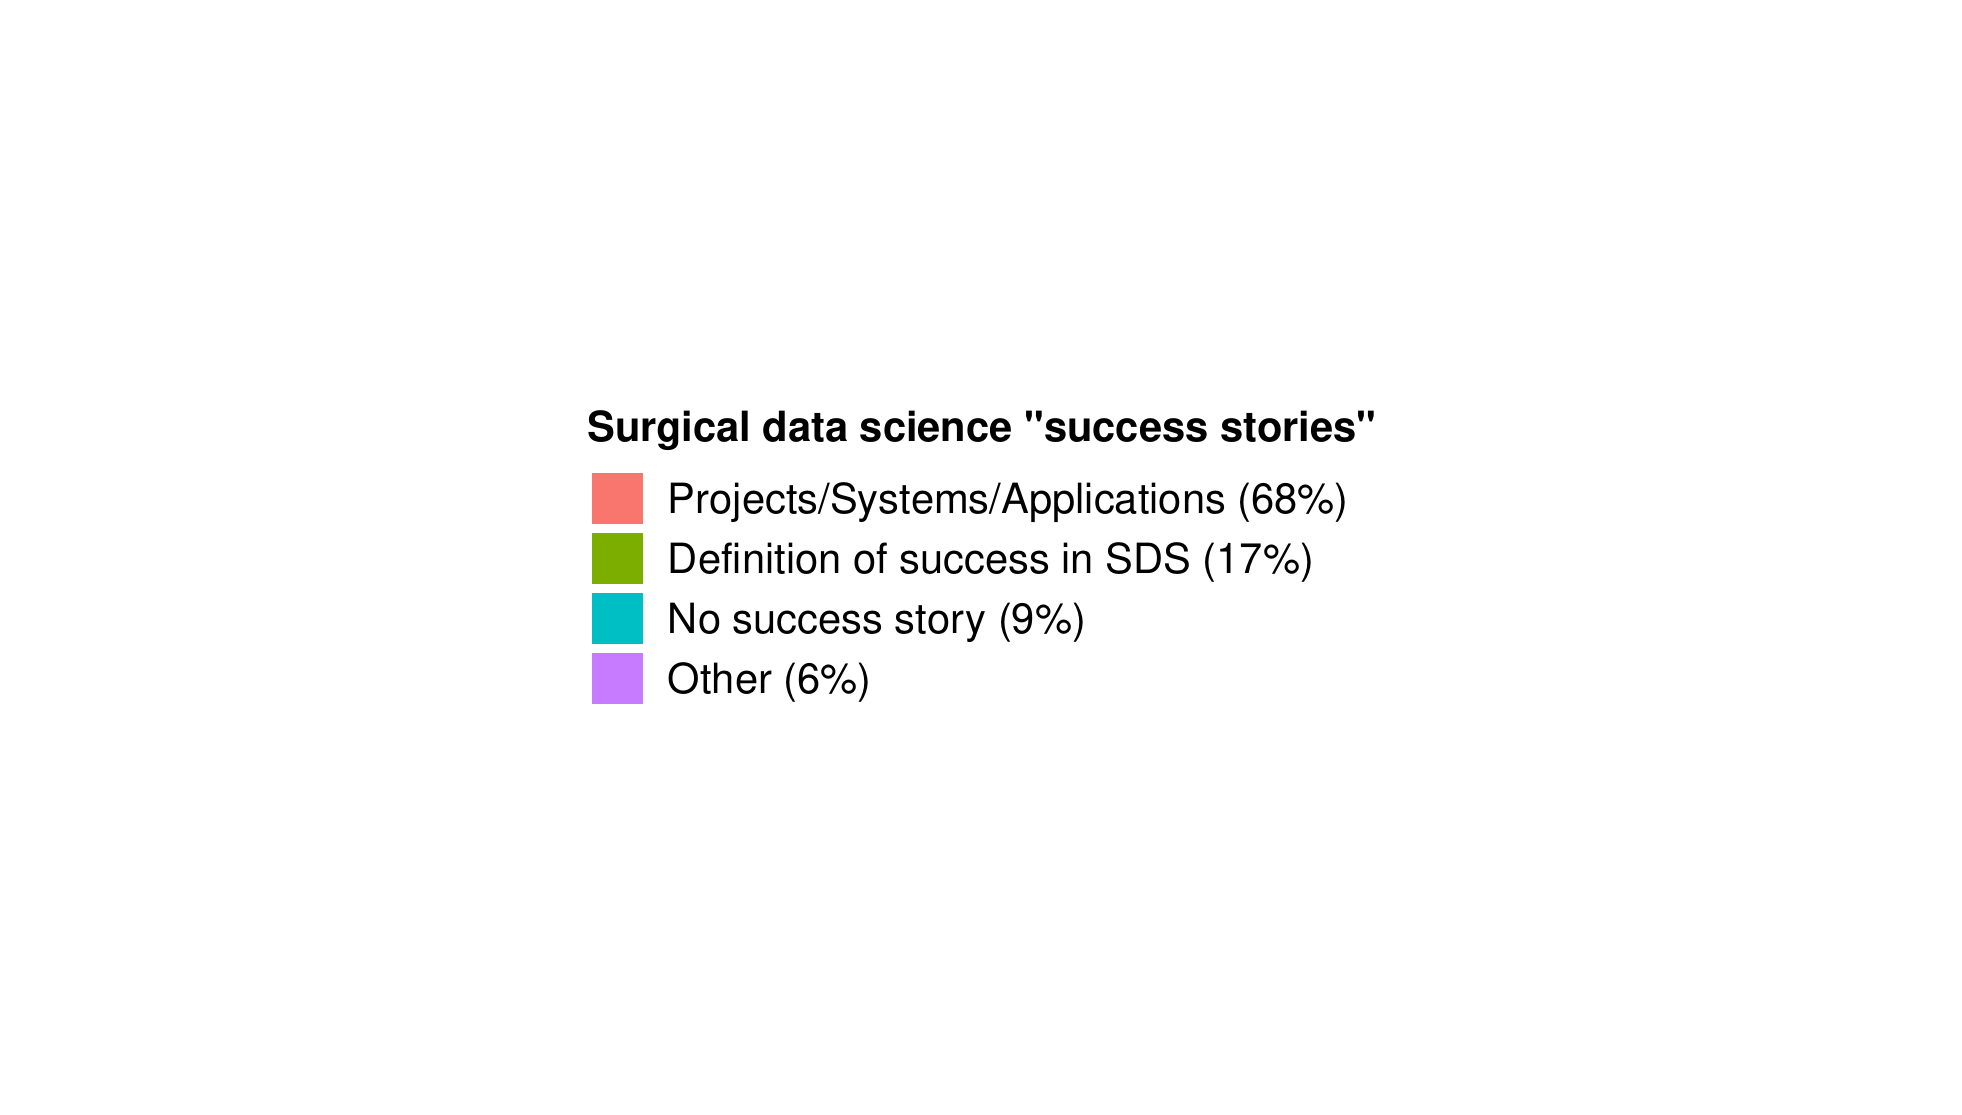}
  \end{subfigure}
\end{figure}

\noindent \textit{\textbf{Q06:} Which research paper in the field of surgical data science has impressed you the most so far?}

\noindent \newline 80\% of the participants responded to this question. 62 partial replies were extracted from the free text and categorized. 81\% of the replies contained references to identifiable publications. The most frequently named publication was \citeappendix{appendix:maier-hein_surgical_2017} (30\%), which originated from the first workshop on surgical data science. 80\% of these nominations were from participants that did not author this paper. With two nominations \citeappendix{appendix:shademan_supervised_2016} was the second most named publication. All other publications were nominated once.

\newpage
\subsection{Challenges related to Surgical Data Science}

\noindent \newline \textit{\textbf{Q07:} What are the most critical challenges related to exploiting the potential of surgical data science?}

\noindent \newline 90\% of participants responded to this question. 142 partial replies were extracted from the free text and categorized.

\begin{figure}[pos=h]
  \begin{subfigure}[c]{0.4\textwidth}
    \includegraphics[width=\textwidth, trim=4cm 1cm 4cm 1cm, clip]{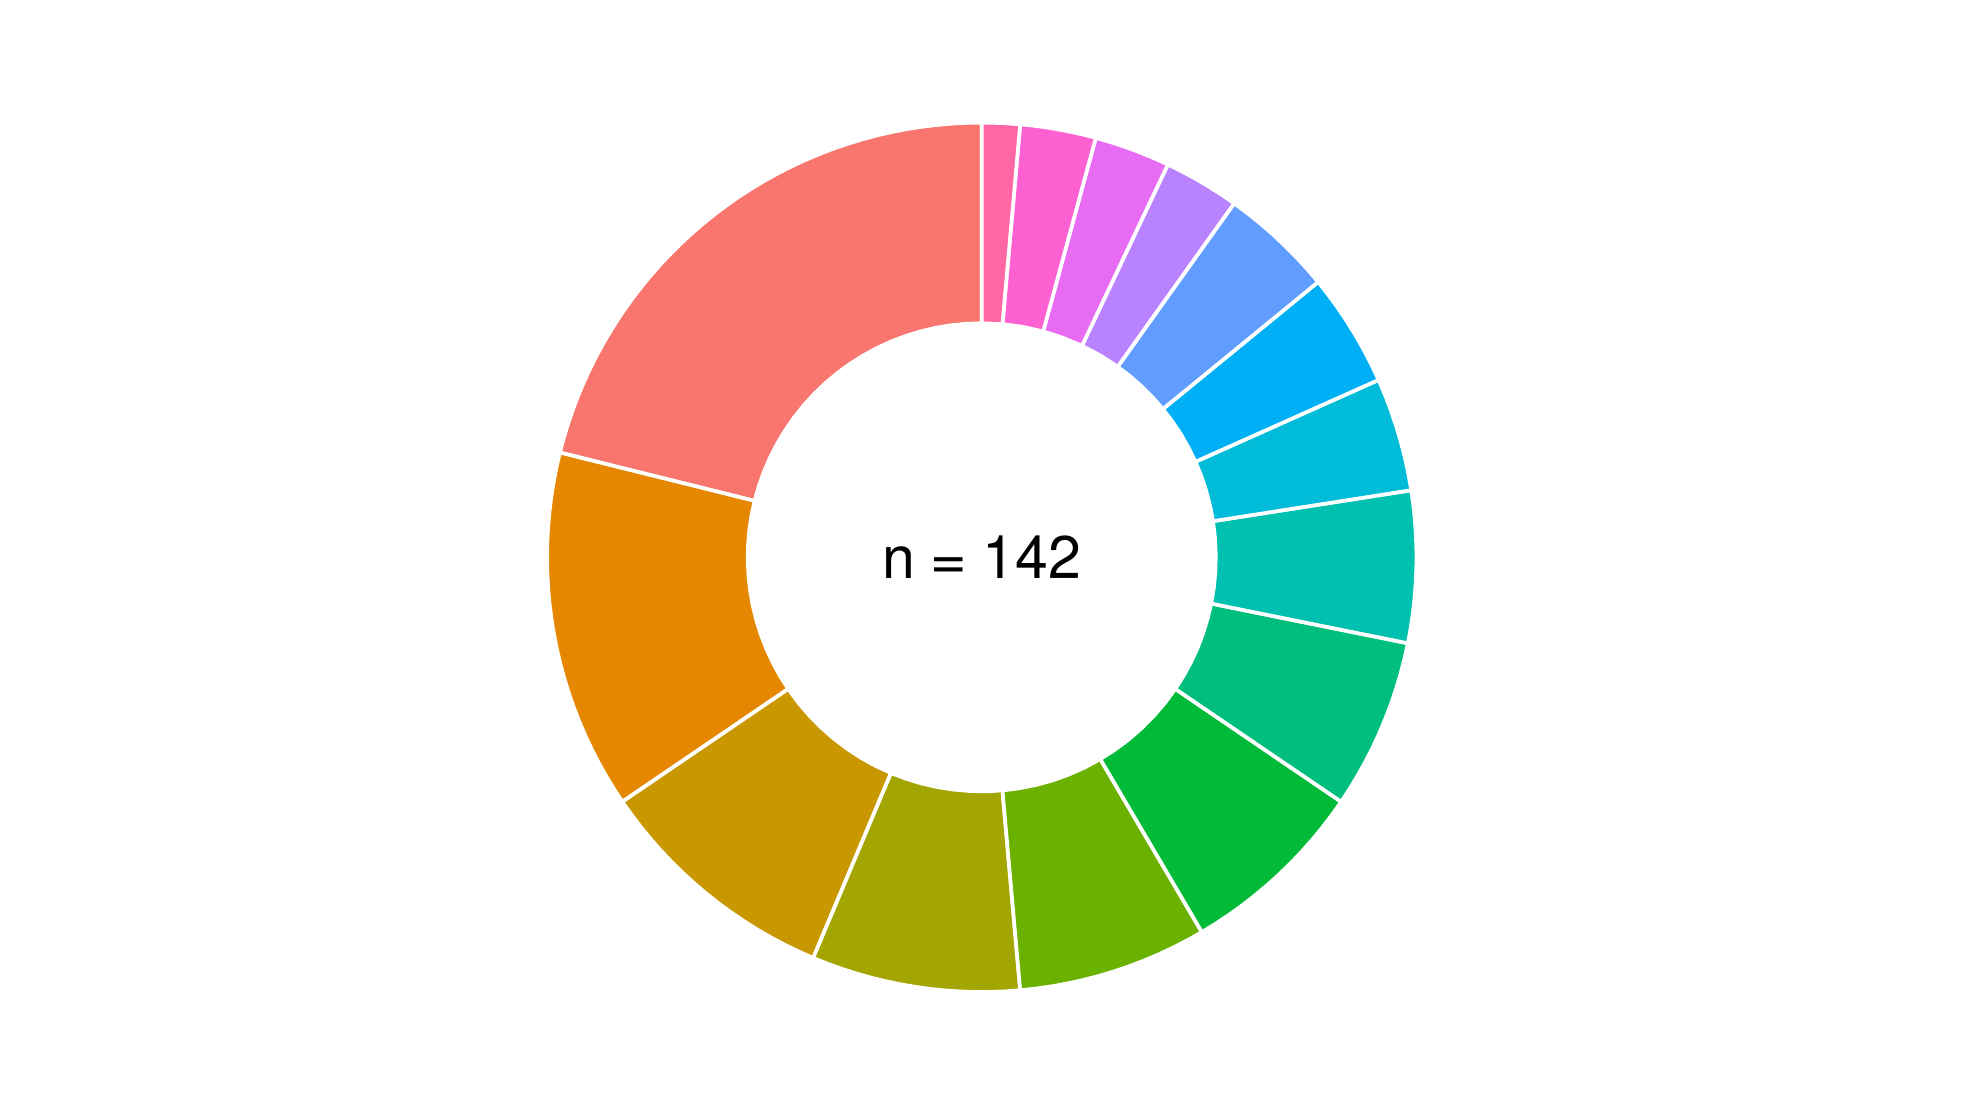}
  \end{subfigure}
  \hfill
  \begin{subfigure}[c]{0.59\textwidth}
    \includegraphics[height=8cm, trim=4cm 0cm 0cm 0cm, clip]{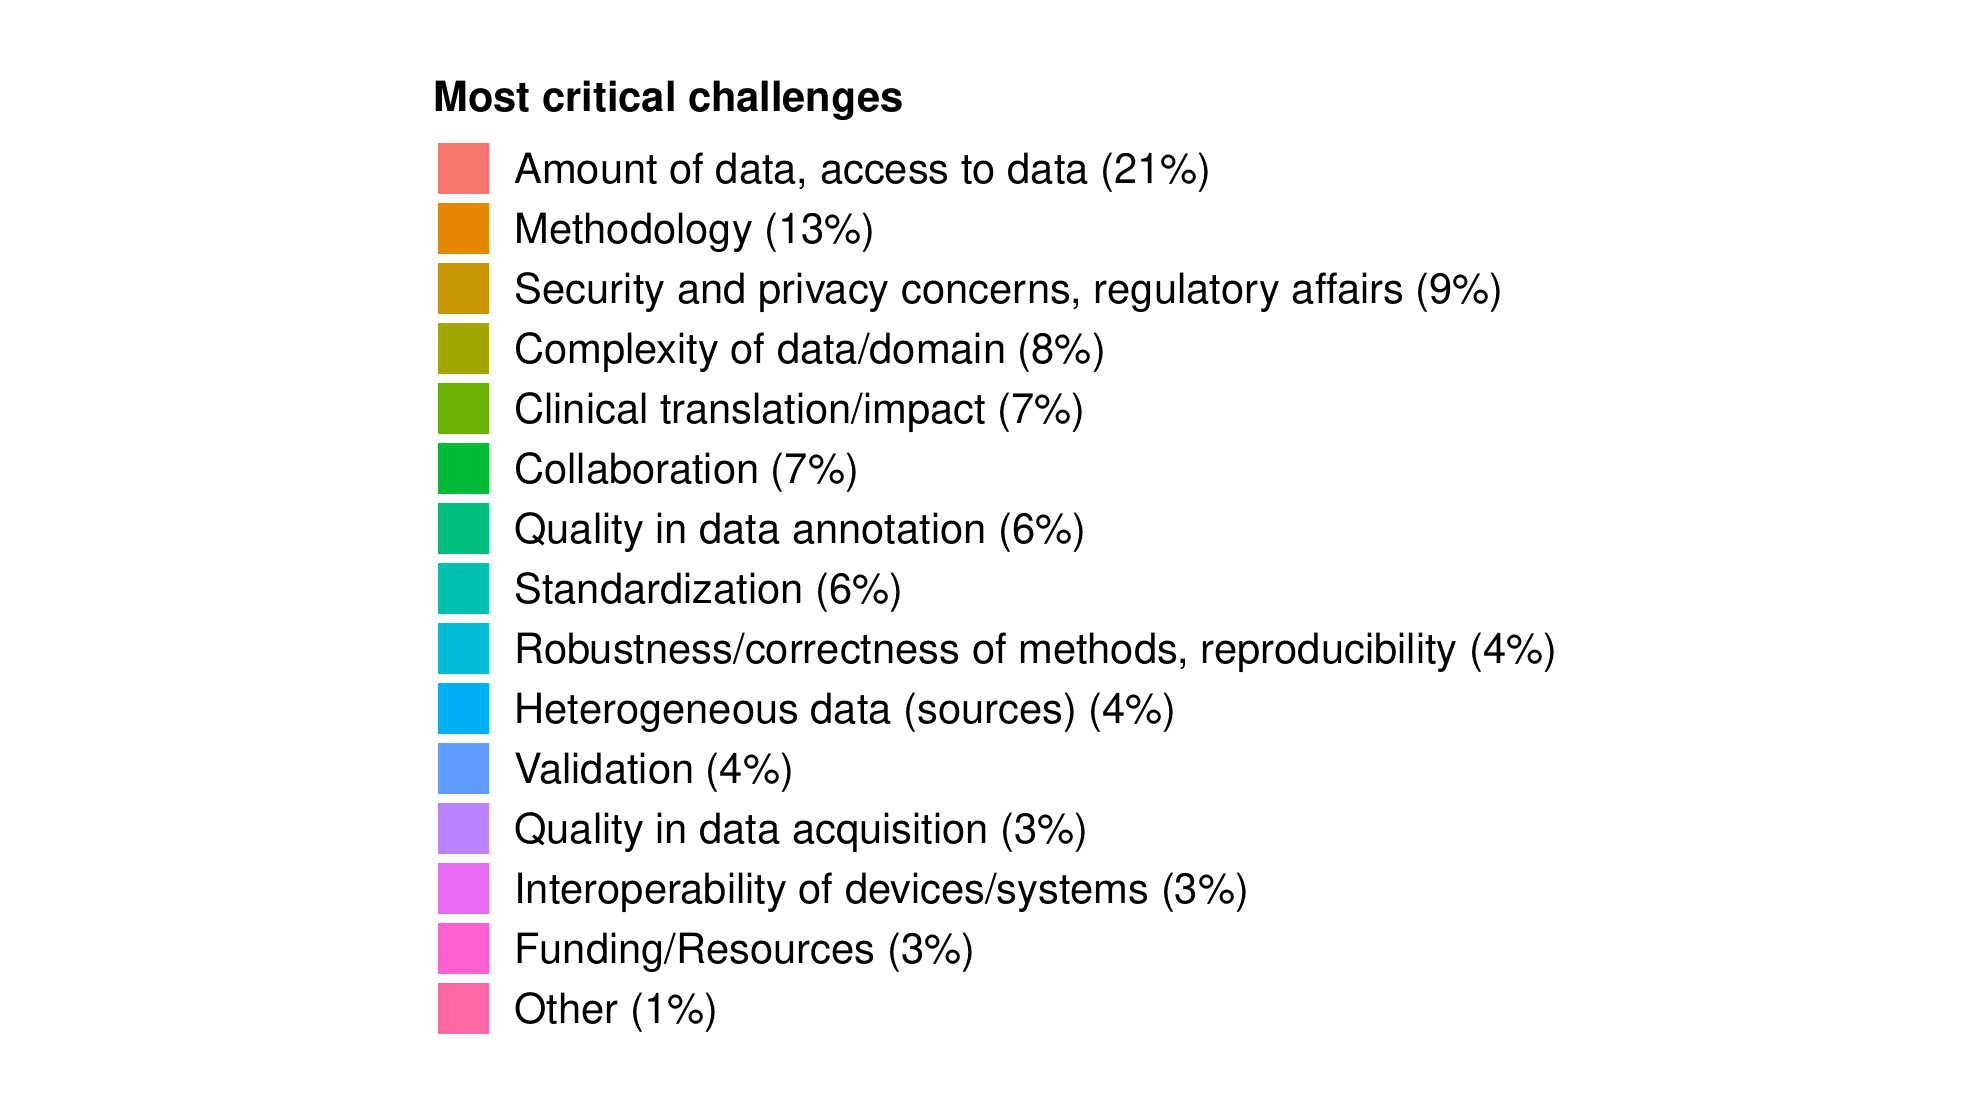}
  \end{subfigure}
\end{figure}

\noindent \textit{\textbf{Q08:} What is lacking in the existing public data sets?}

\noindent \newline 81\% of participants responded to this question. 82 partial replies were extracted from the free text and categorized.

\begin{figure}[pos=h]
  \begin{subfigure}[c]{0.4\textwidth}
    \includegraphics[width=\textwidth, trim=4cm 1cm 4cm 1cm, clip]{figures/q08_lack_in_public_data sets_plot.pdf}
  \end{subfigure}
  \hfill
  \begin{subfigure}[c]{0.59\textwidth}
    \includegraphics[height=5cm, trim=5.5cm 2cm 0cm 2cm, clip]{figures/q08_lack_in_public_data sets_legend.pdf}
  \end{subfigure}
\end{figure}

\newpage
\noindent \textit{\textbf{Q09:} What do you consider as the most urgent issue/problem that needs to be discussed in the workshop (e.g. standards)?}

\noindent \newline 84\% of participants responded to this question. 96 partial replies were extracted from the free text and categorized.

\begin{figure}[pos=h]
  \begin{subfigure}[c]{0.4\textwidth}
    \includegraphics[width=\textwidth, trim=4cm 1cm 4cm 1cm, clip]{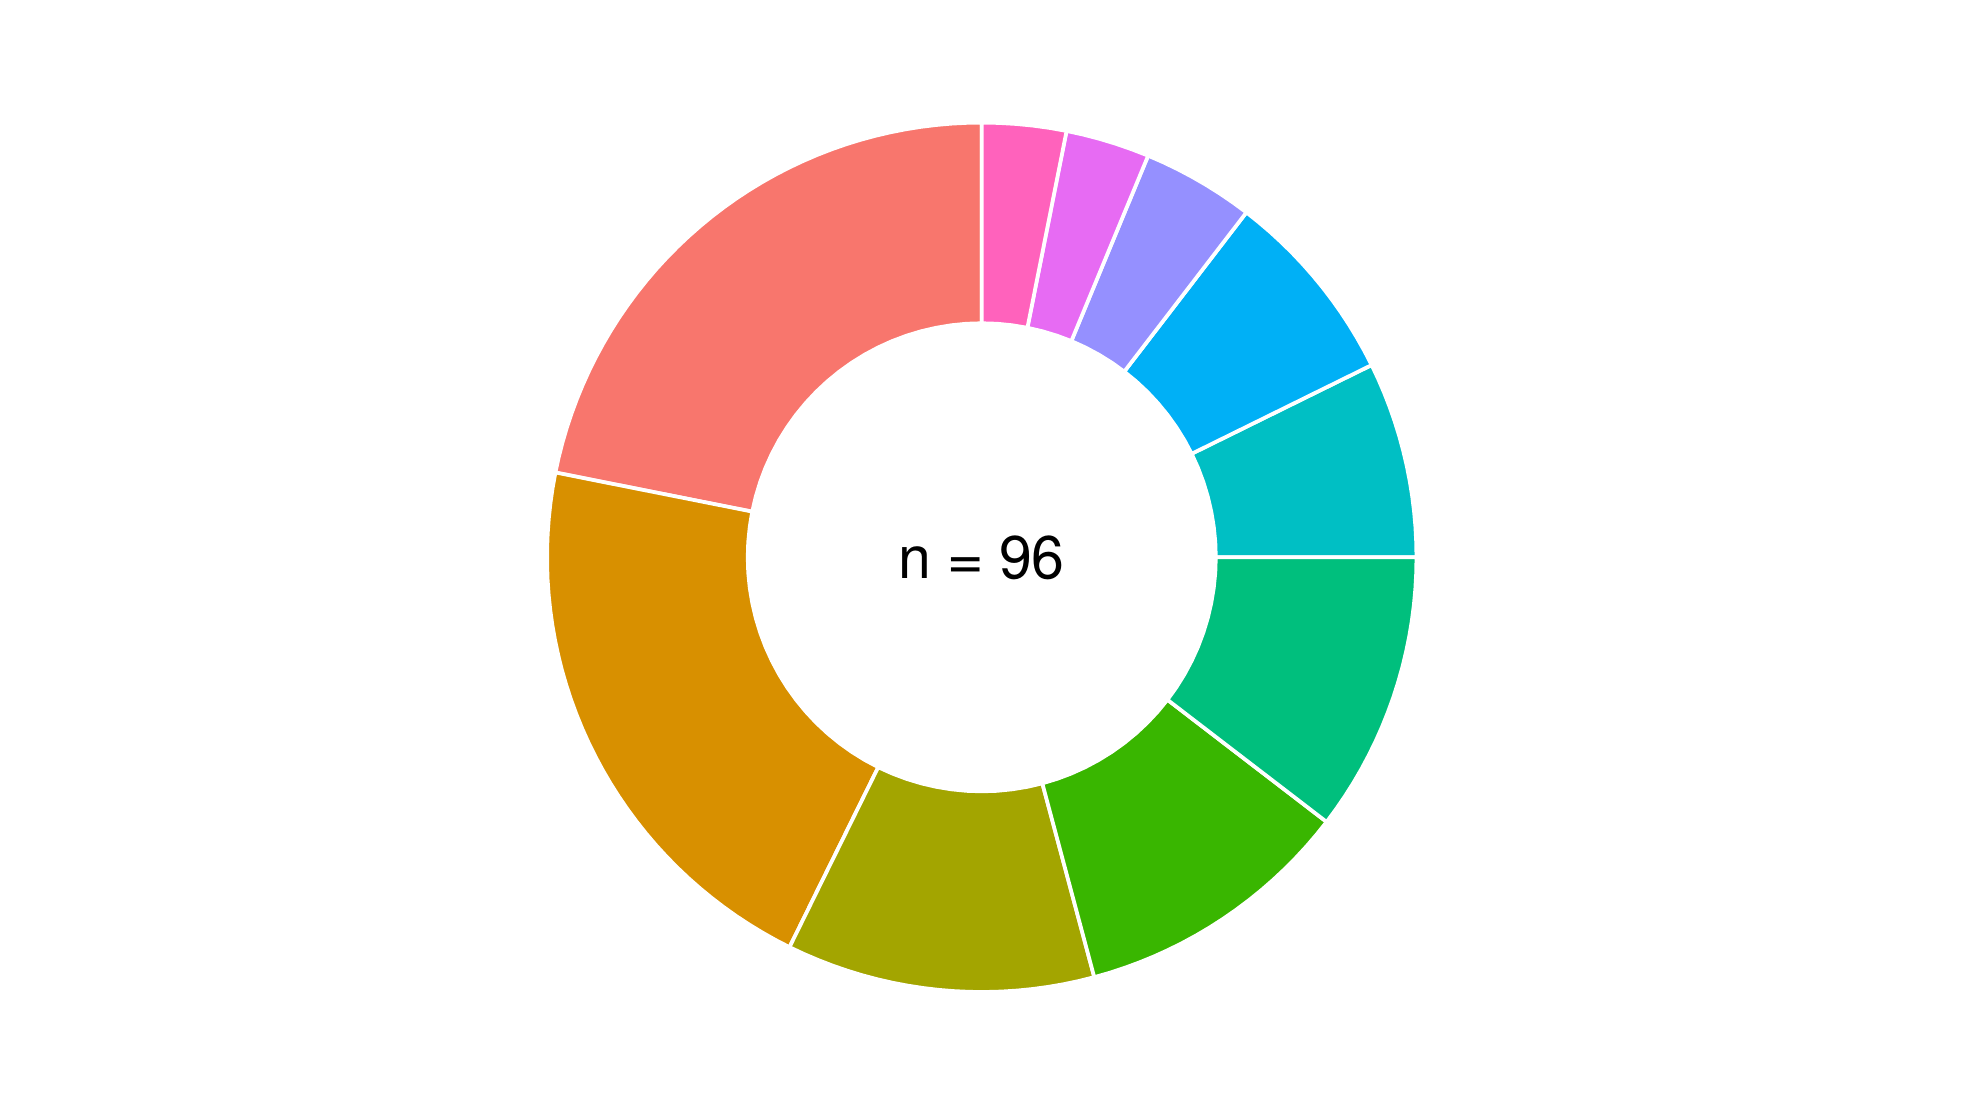}
  \end{subfigure}
  \hfill
  \begin{subfigure}[c]{0.59\textwidth}
    \includegraphics[height=5cm, trim=4.5cm 2cm 0cm 2cm, clip]{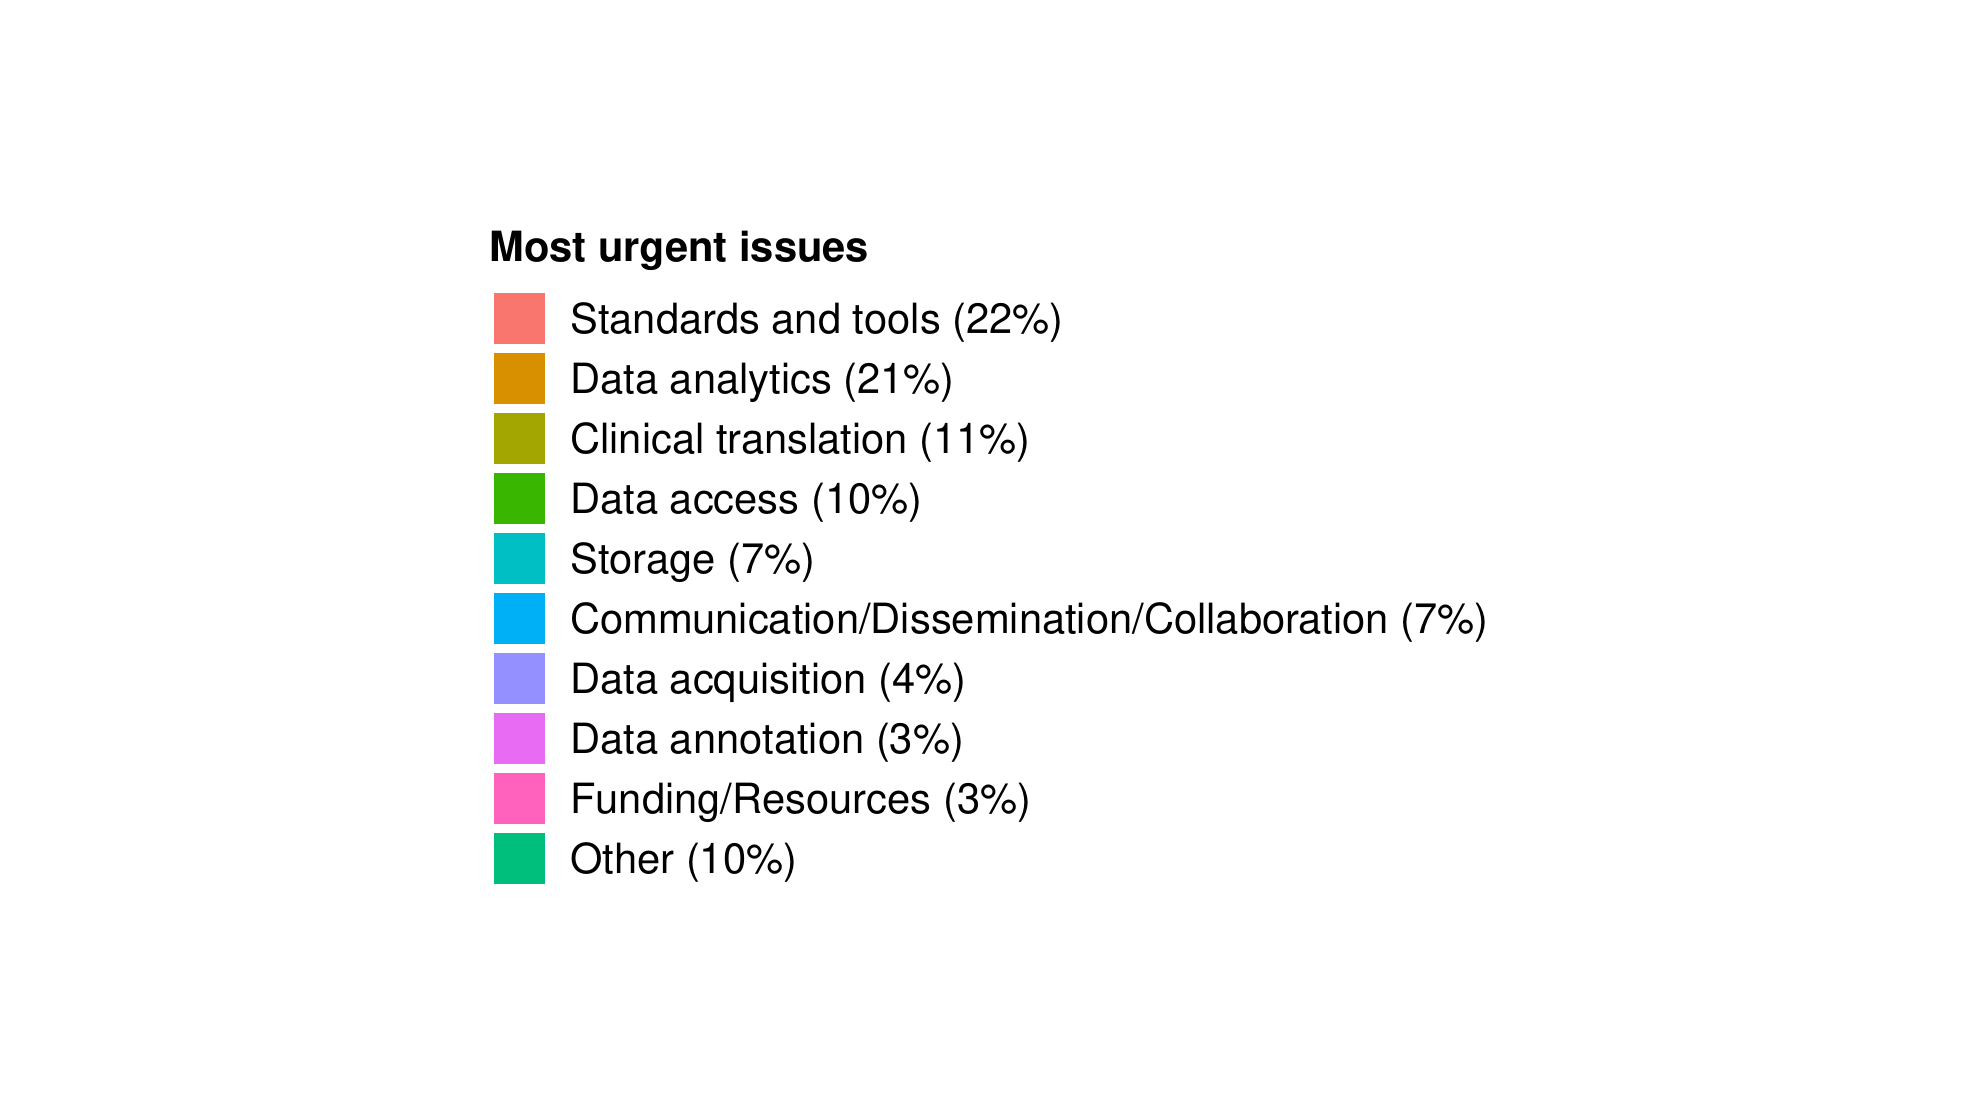}
  \end{subfigure}
\end{figure}

\noindent \textit{\textbf{Q10:} Please list at least one surgical data science (clinical) application that can be regarded as a (relatively) low hanging fruit (i.e. could be addressed in a relatively short period of time).}

\noindent \newline 79\% of participants responded to this question. 70 partial replies were extracted from the free text and categorized. Of these, 7\% expressed doubts that low hanging fruit exist. 92\% of the replies contained fields and applications of low hanging fruit, including instrument segmentation, skill assessment and training, tracking, prediction of outcome and duration as well as sharing data and tools. These sub-categories were nominated more than twice. 1\% of the replies contained a definition of high hanging fruit.

%\vspace{\baselineskip}

\noindent \newline \textit{\textbf{Q11:} What should be the next SDS challenge (open competition)?}

\noindent \newline 71\% of participants responded to this question. 67 partial replies were extracted from the free text and categorized. Of these, 40\% of replies contain nominations of challenges that cannot be assigned to any of the categories.

\begin{figure}[pos=h]
  \begin{subfigure}[c]{0.4\textwidth}
    \includegraphics[width=\textwidth, trim=4cm 1cm 4cm 1cm, clip]{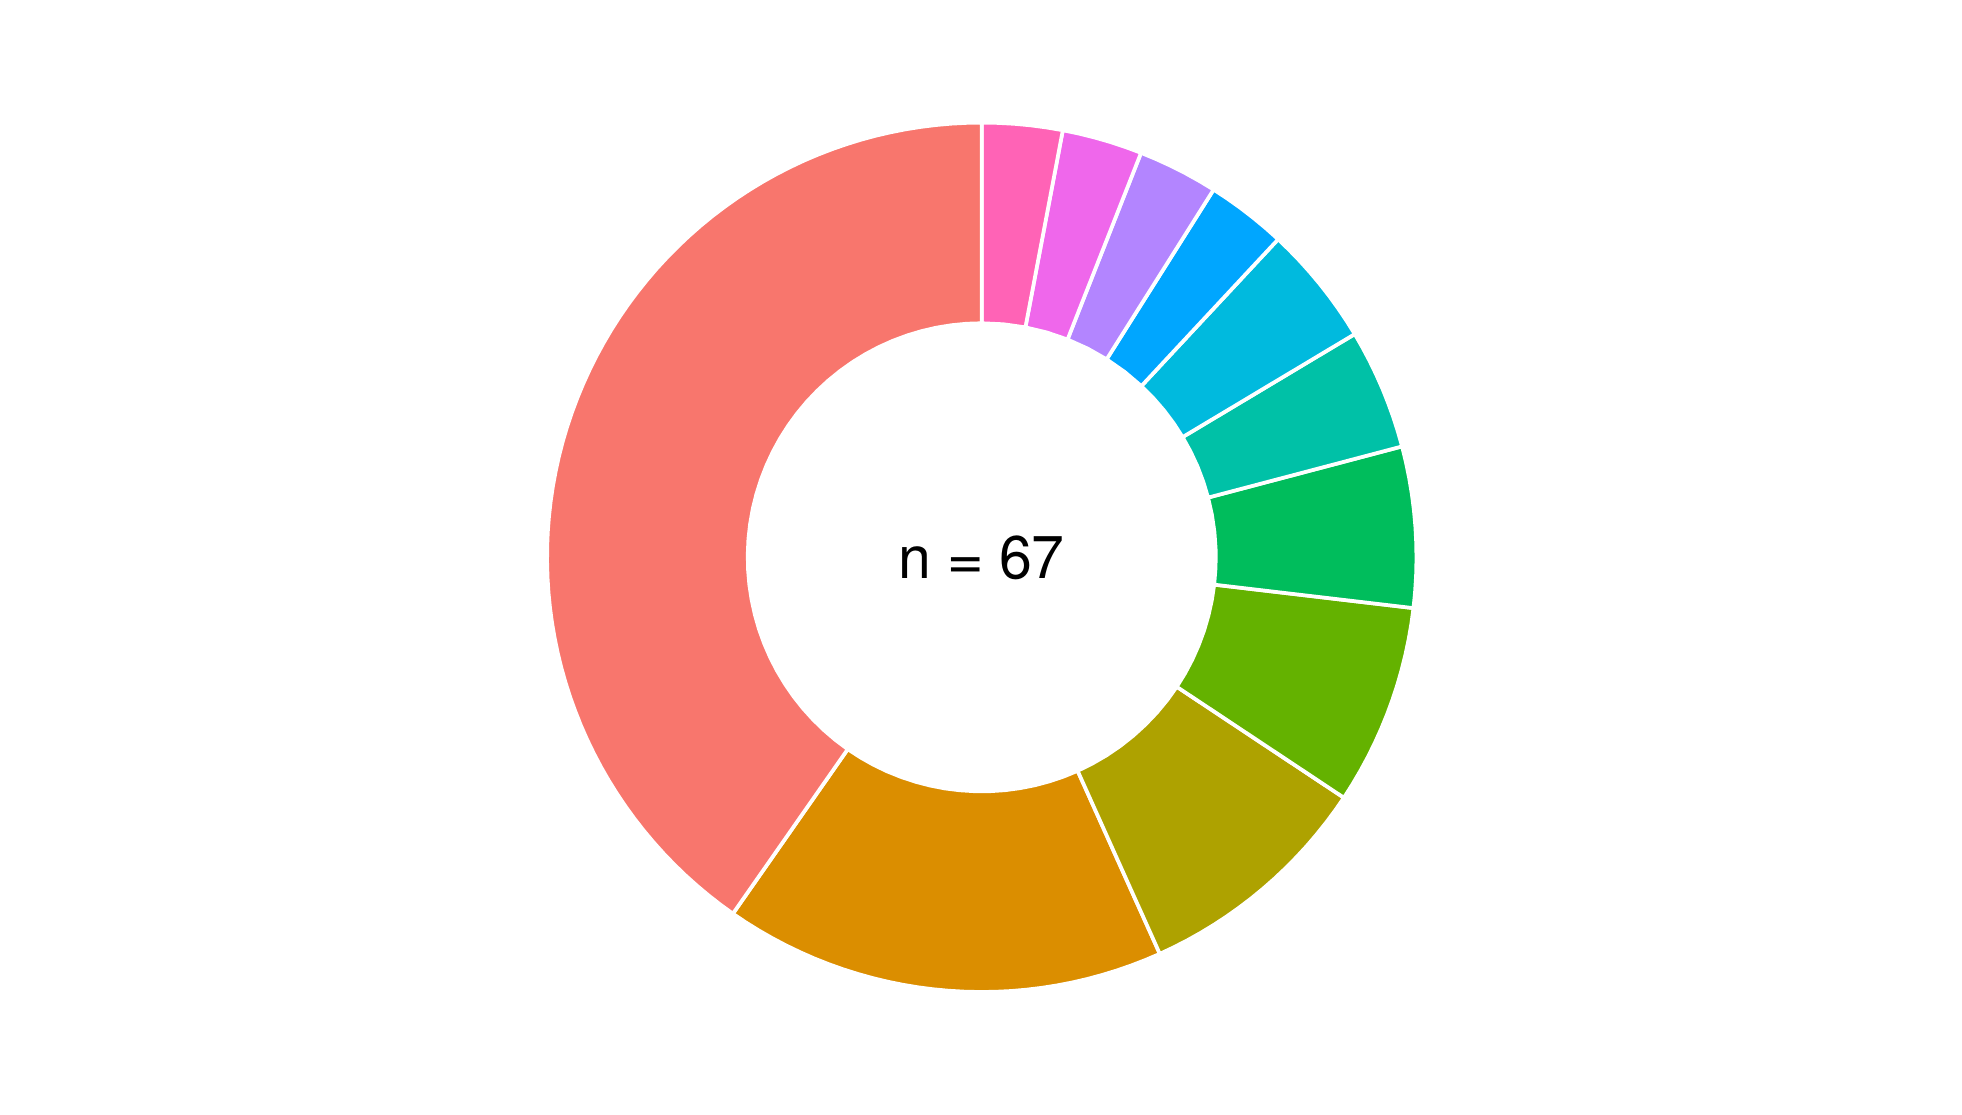}
  \end{subfigure}
  \hfill
  \begin{subfigure}[c]{0.59\textwidth}
    \includegraphics[height=5cm, trim=6.5cm 2cm 0cm 2cm, clip]{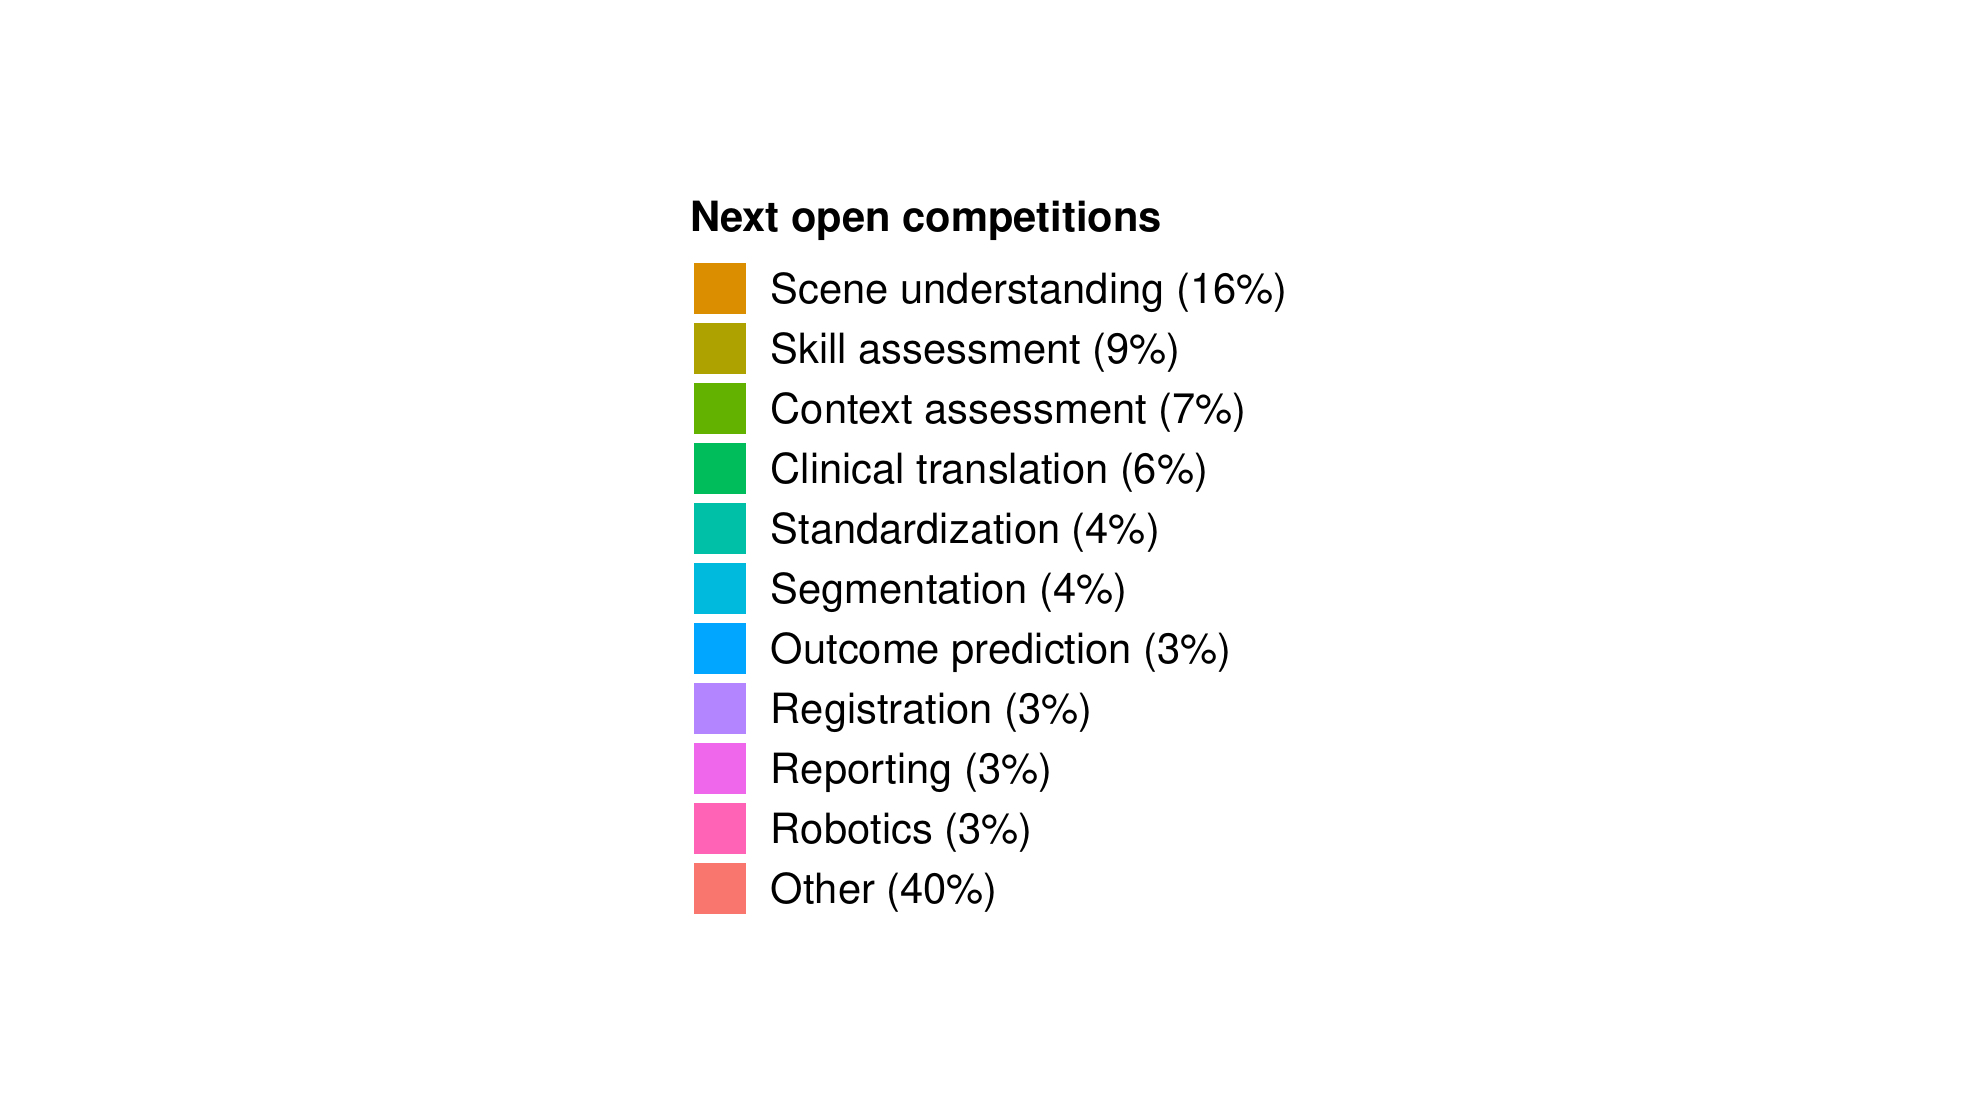}
  \end{subfigure}
\end{figure}

\newpage
\subsection{Personal experience with Surgical Data Science}

\noindent \newline \textit{\textbf{Q12:} What public data set have you found the most useful for your research in SDS so far?}

\noindent \newline 79\% of participants responded to this question. 82 partial replies were extracted from the free text and categorized. Of these, 71\% contained references to identifiable data sets (either general collections or subsets). 29\% contained other responses, e.g. including non-identifiable data sets, persons stating that they are not able to name one, because they are new to the field or they were using private data sets so far. Among the identifiable data sets, \citeappendix{appendix:endovis_endovis_nodate} was most frequently named (28\%). With 21\% of nominations Cholec80 \citepappendix{appendix:twinanda_endonet_2017} is the second most named data set, followed by JIGSAWS \citepappendix{appendix:gao_jhu-isi_2014} (17\%). Four data sets were named twice. 21\% of data sets were named once.

\noindent \newline \textit{\textbf{Q13:} What was your biggest failure in SDS, even though it looked promising at the beginning, to avoid others making the same mistake?}

\noindent \newline 68\% of participants were able to name a failure in SDS. 52 partial replies were extracted from the free text and categorized. Of these, 10\% contained references to non-identifiable projects 32\% of participants did not provide an answer for various reasons (e.g. confidentiality, novice in field).

\begin{figure}[pos=h]
  \begin{subfigure}[c]{0.4\textwidth}
    \includegraphics[width=\textwidth, trim=4cm 1cm 4cm 1cm, clip]{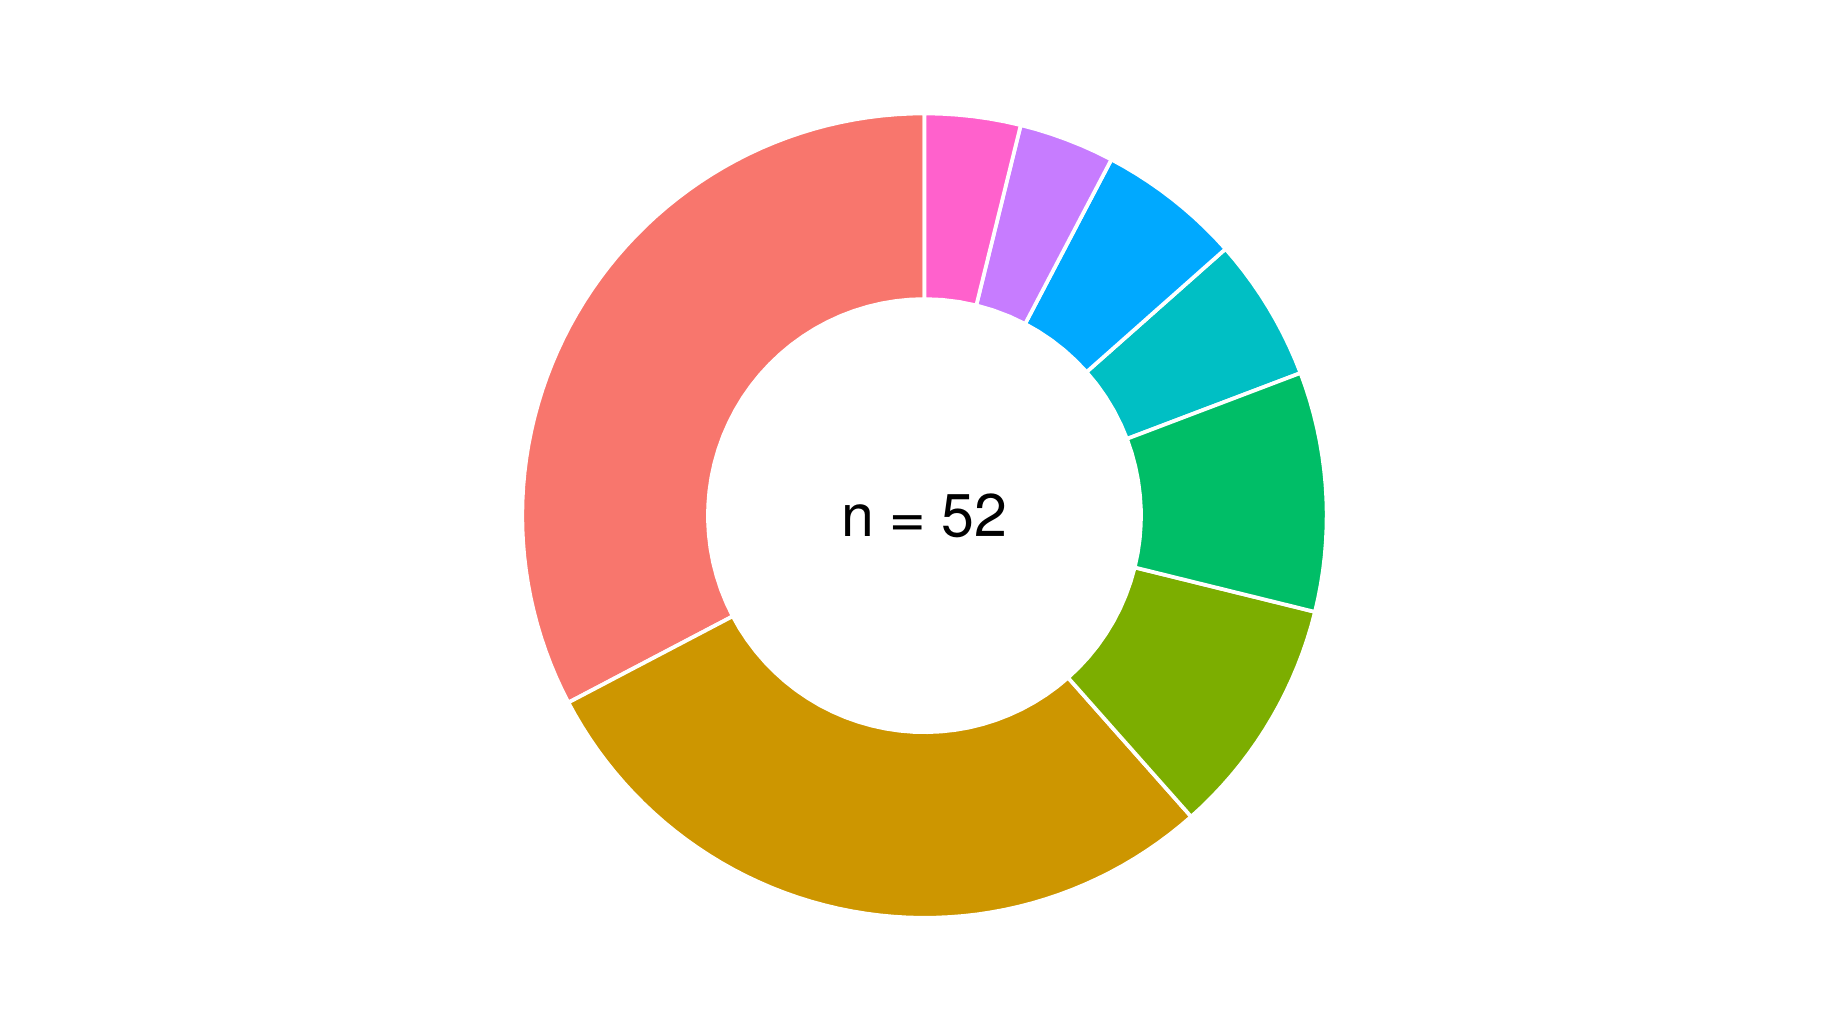}
  \end{subfigure}
  \hfill
  \begin{subfigure}[c]{0.59\textwidth}
    \includegraphics[height=5cm, trim=4.5cm 2cm 0cm 2cm, clip]{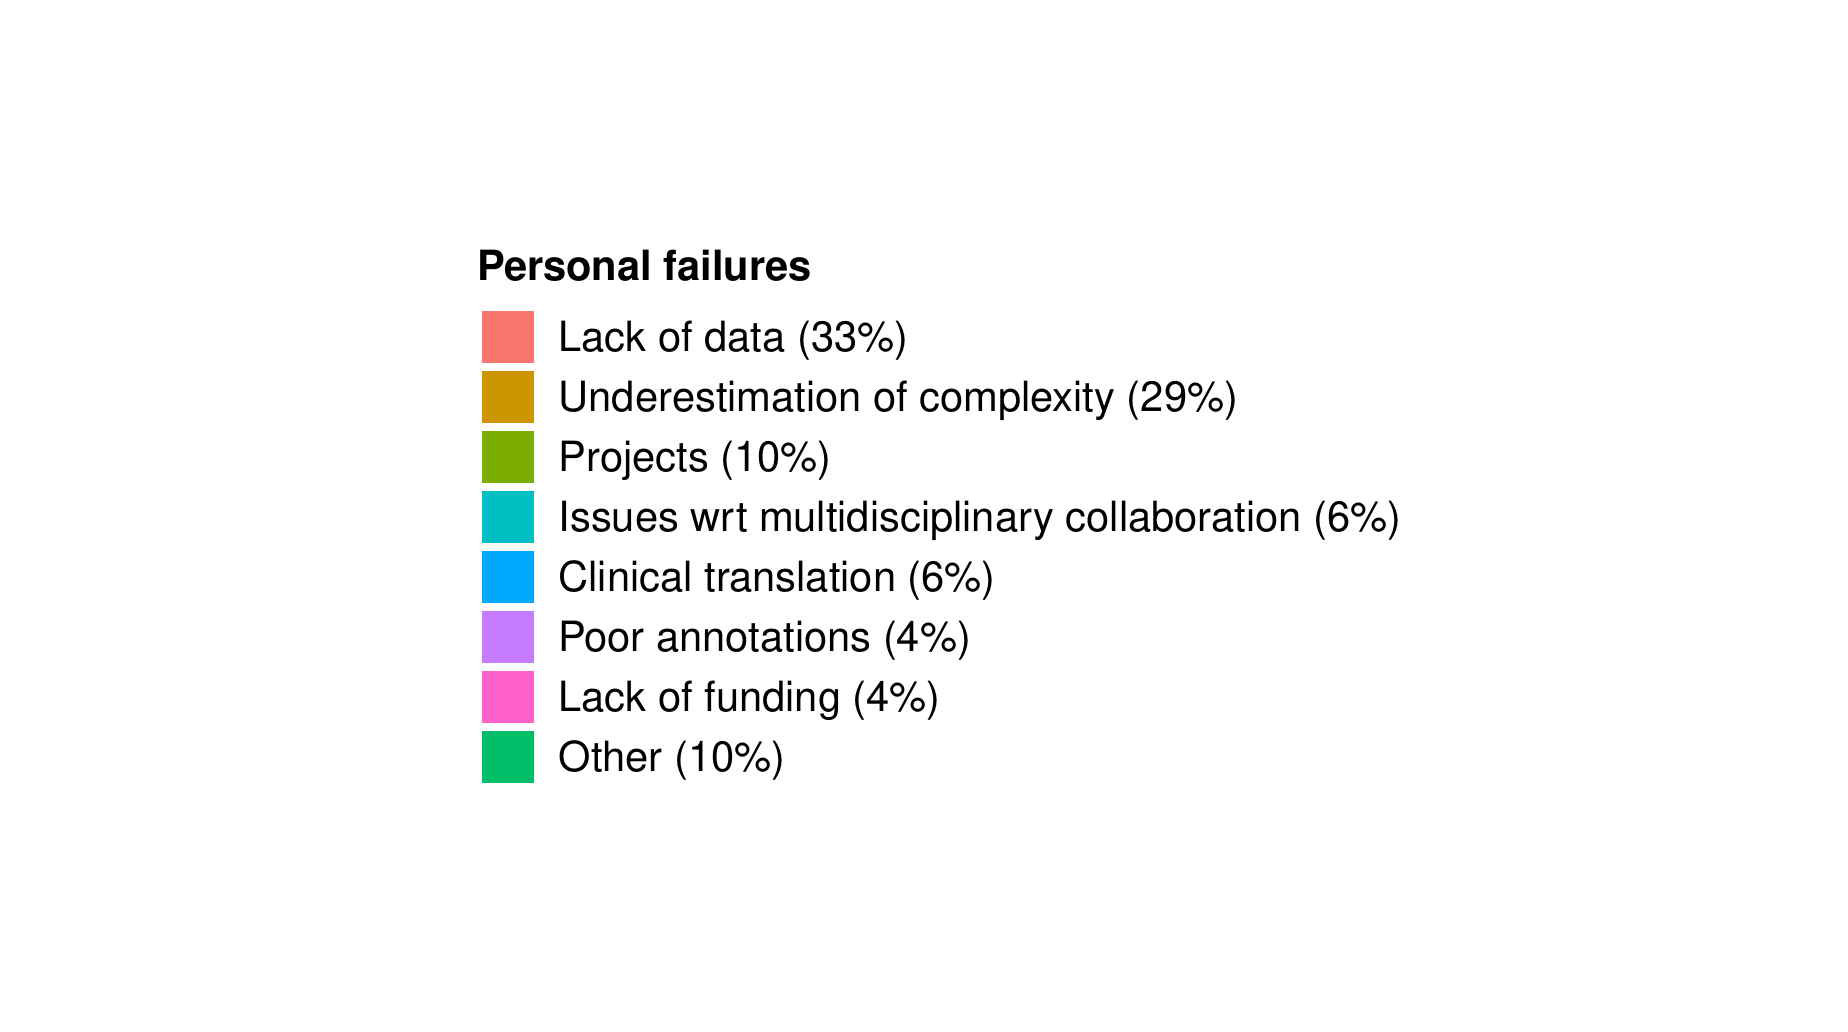}
  \end{subfigure}
\end{figure}

\noindent \newline \textit{\textbf{Q14:} What is your advice for avoiding these problems?}

\noindent \newline 64 partial replies were extracted from the free text and categorized. 25\% of these replies recommend to collaborate (early) with different stakeholders (e.g. clinicians, statisticians, technology experts) to succeed in SDS projects. Having access to more data in general (17\%) and investing in a robust infrastructure for data acquisition (6\%) as well as high-quality annotations (5\%) specifically is also advised. Defining smaller project goals (9\%) can help to identify pitfalls. Topics related to education and dissemination (e.g. understanding well-posedness of a problem) (8\%) as well as proper validation (5\%) are also covered by the participants’ advice.

\begin{figure}[pos=h]
  \begin{subfigure}[c]{0.4\textwidth}
    \includegraphics[width=\textwidth, trim=4cm 1cm 4cm 1cm, clip]{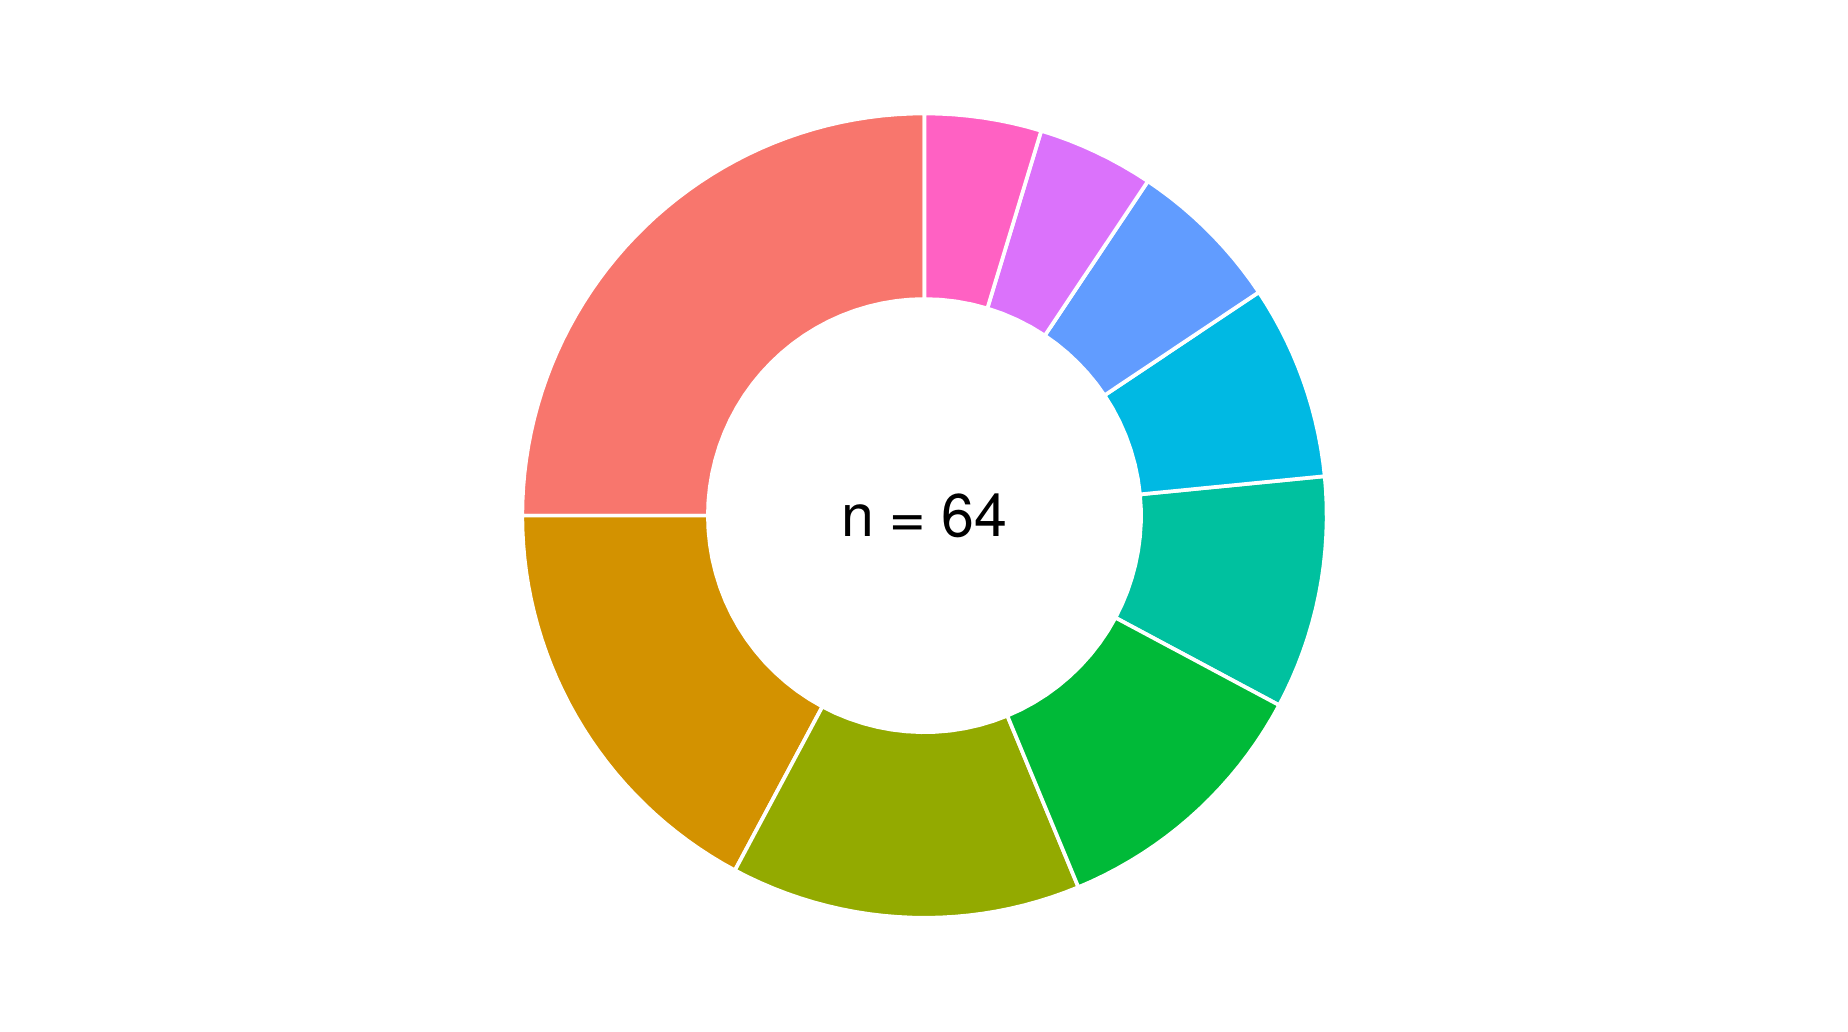}
  \end{subfigure}
  \hfill
  \begin{subfigure}[c]{0.59\textwidth}
    \includegraphics[height=5cm, trim=5.2cm 2cm 0cm 2cm, clip]{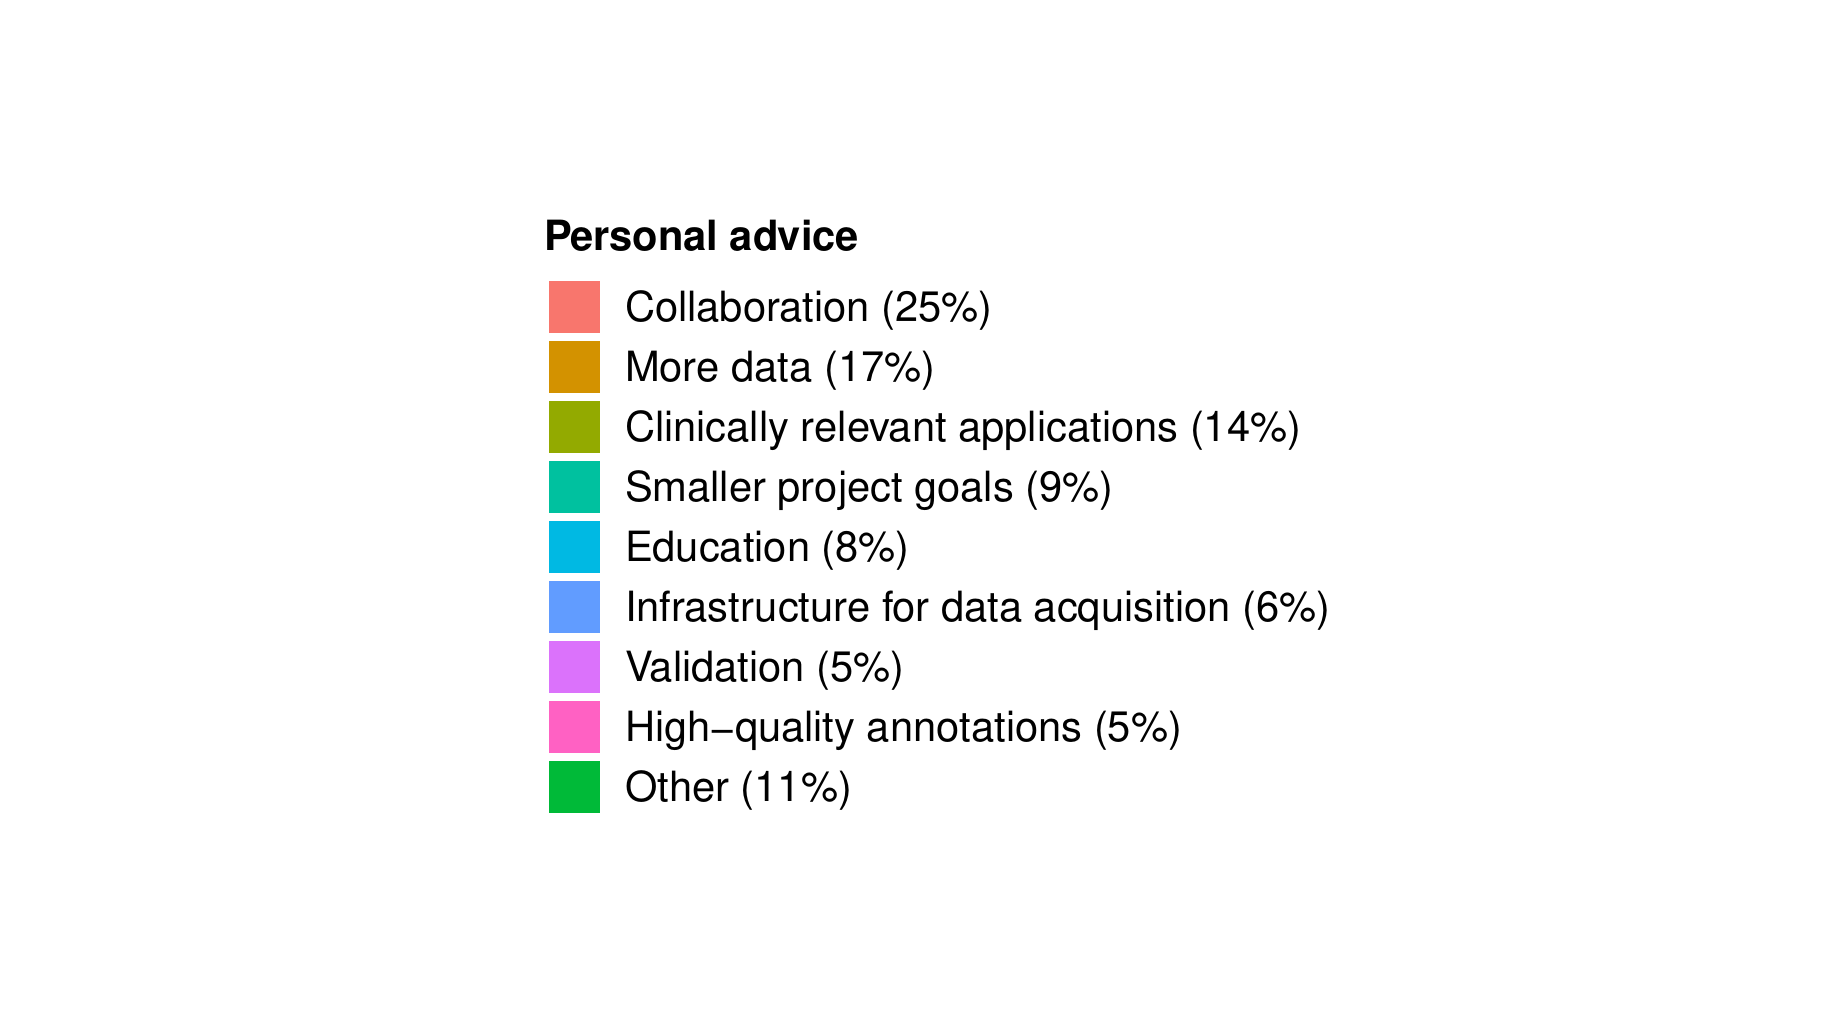}
  \end{subfigure}
\end{figure}

\subsection{Joint Surgical Data Science Project}

\noindent \newline \textit{\textbf{Q15:} Would you be interested to work on a joint surgical data science project with other workshop attendees?}

\begin{figure}[pos=h]
  \begin{subfigure}[c]{0.4\textwidth}
    \includegraphics[width=\textwidth, trim=4cm 1cm 4cm 1cm, clip]{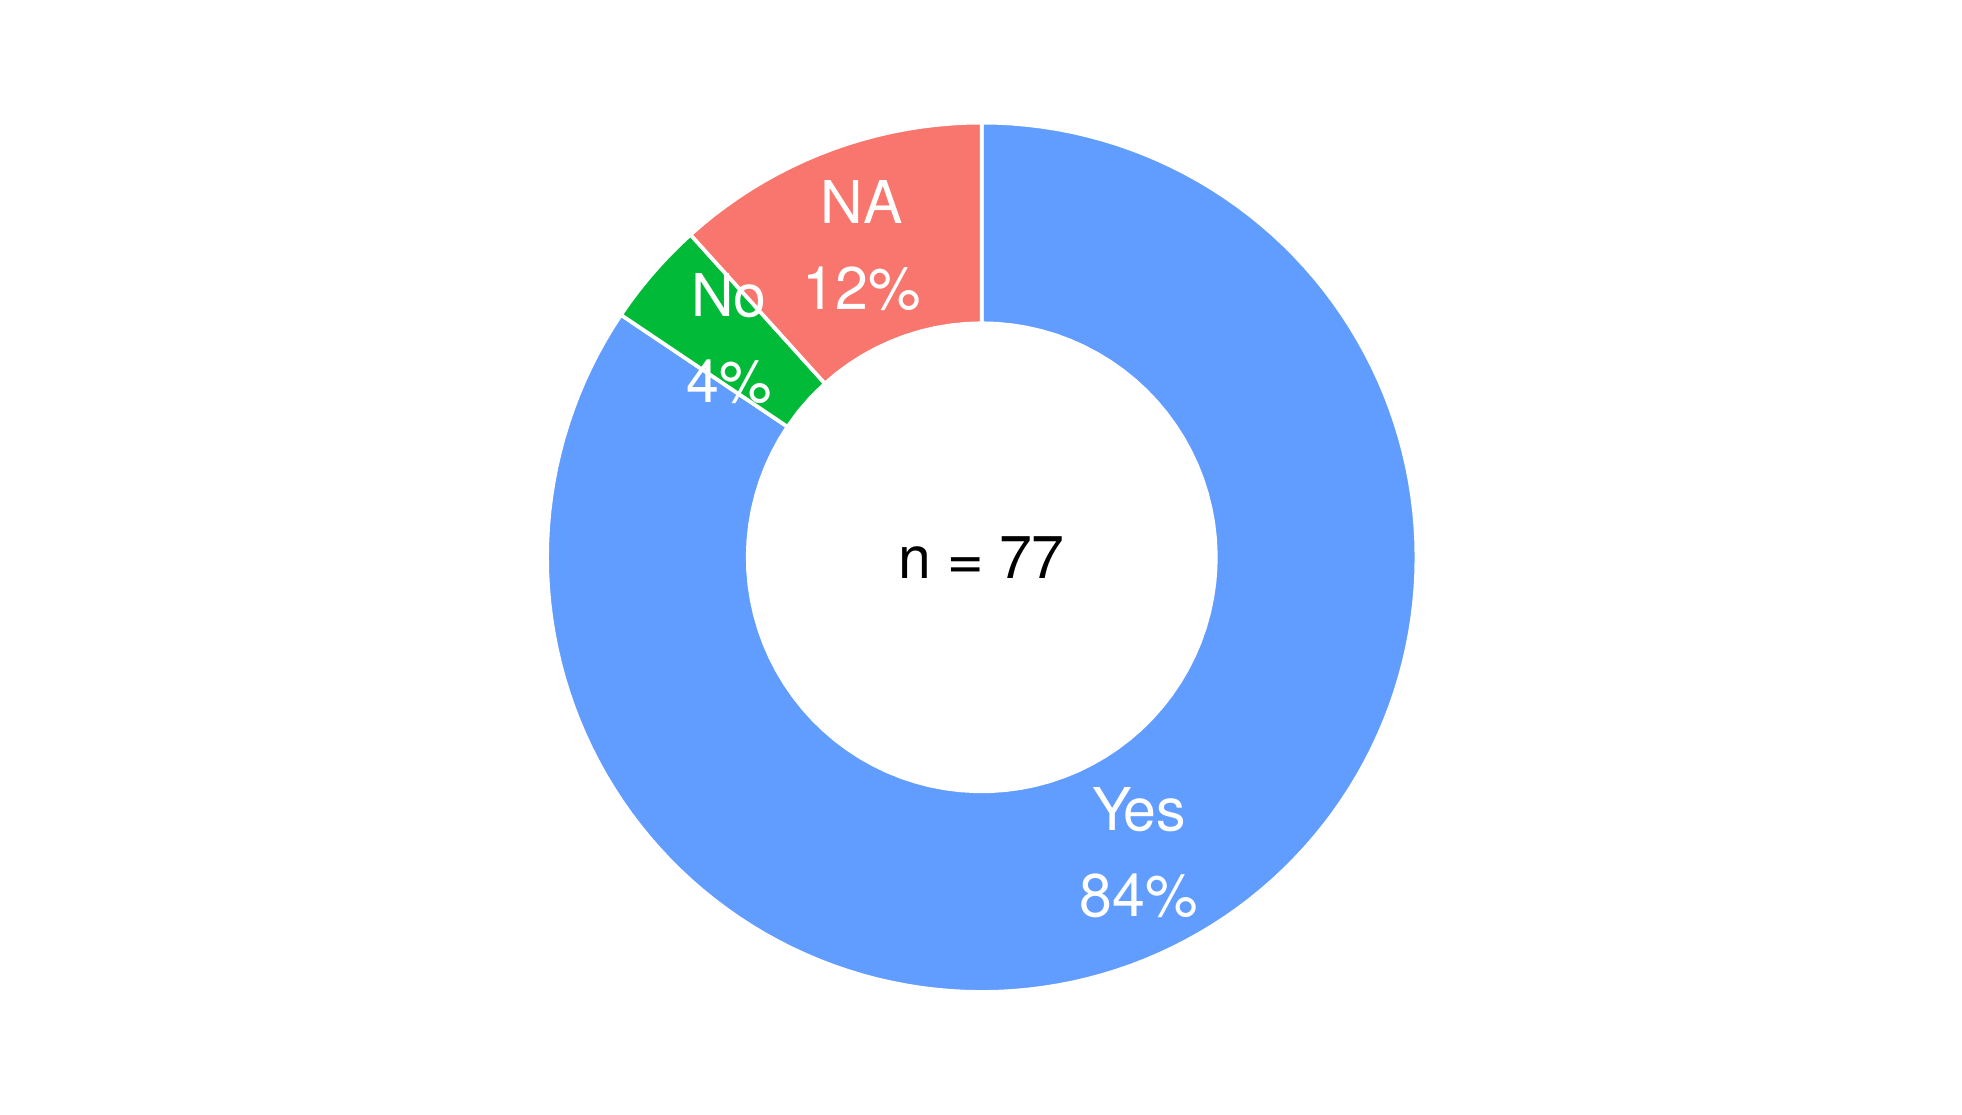}
  \end{subfigure}
  \hfill
  \begin{subfigure}[c]{0.59\textwidth}
    \includegraphics[height=5cm]{figures/blank.pdf}
  \end{subfigure}
\end{figure}

\noindent \textit{\textbf{Q16:} Do you (potentially) have data to contribute to such a project?}

\begin{figure}[pos=h]
  \begin{subfigure}[c]{0.4\textwidth}
    \includegraphics[width=\textwidth, trim=4cm 1cm 4cm 1cm, clip]{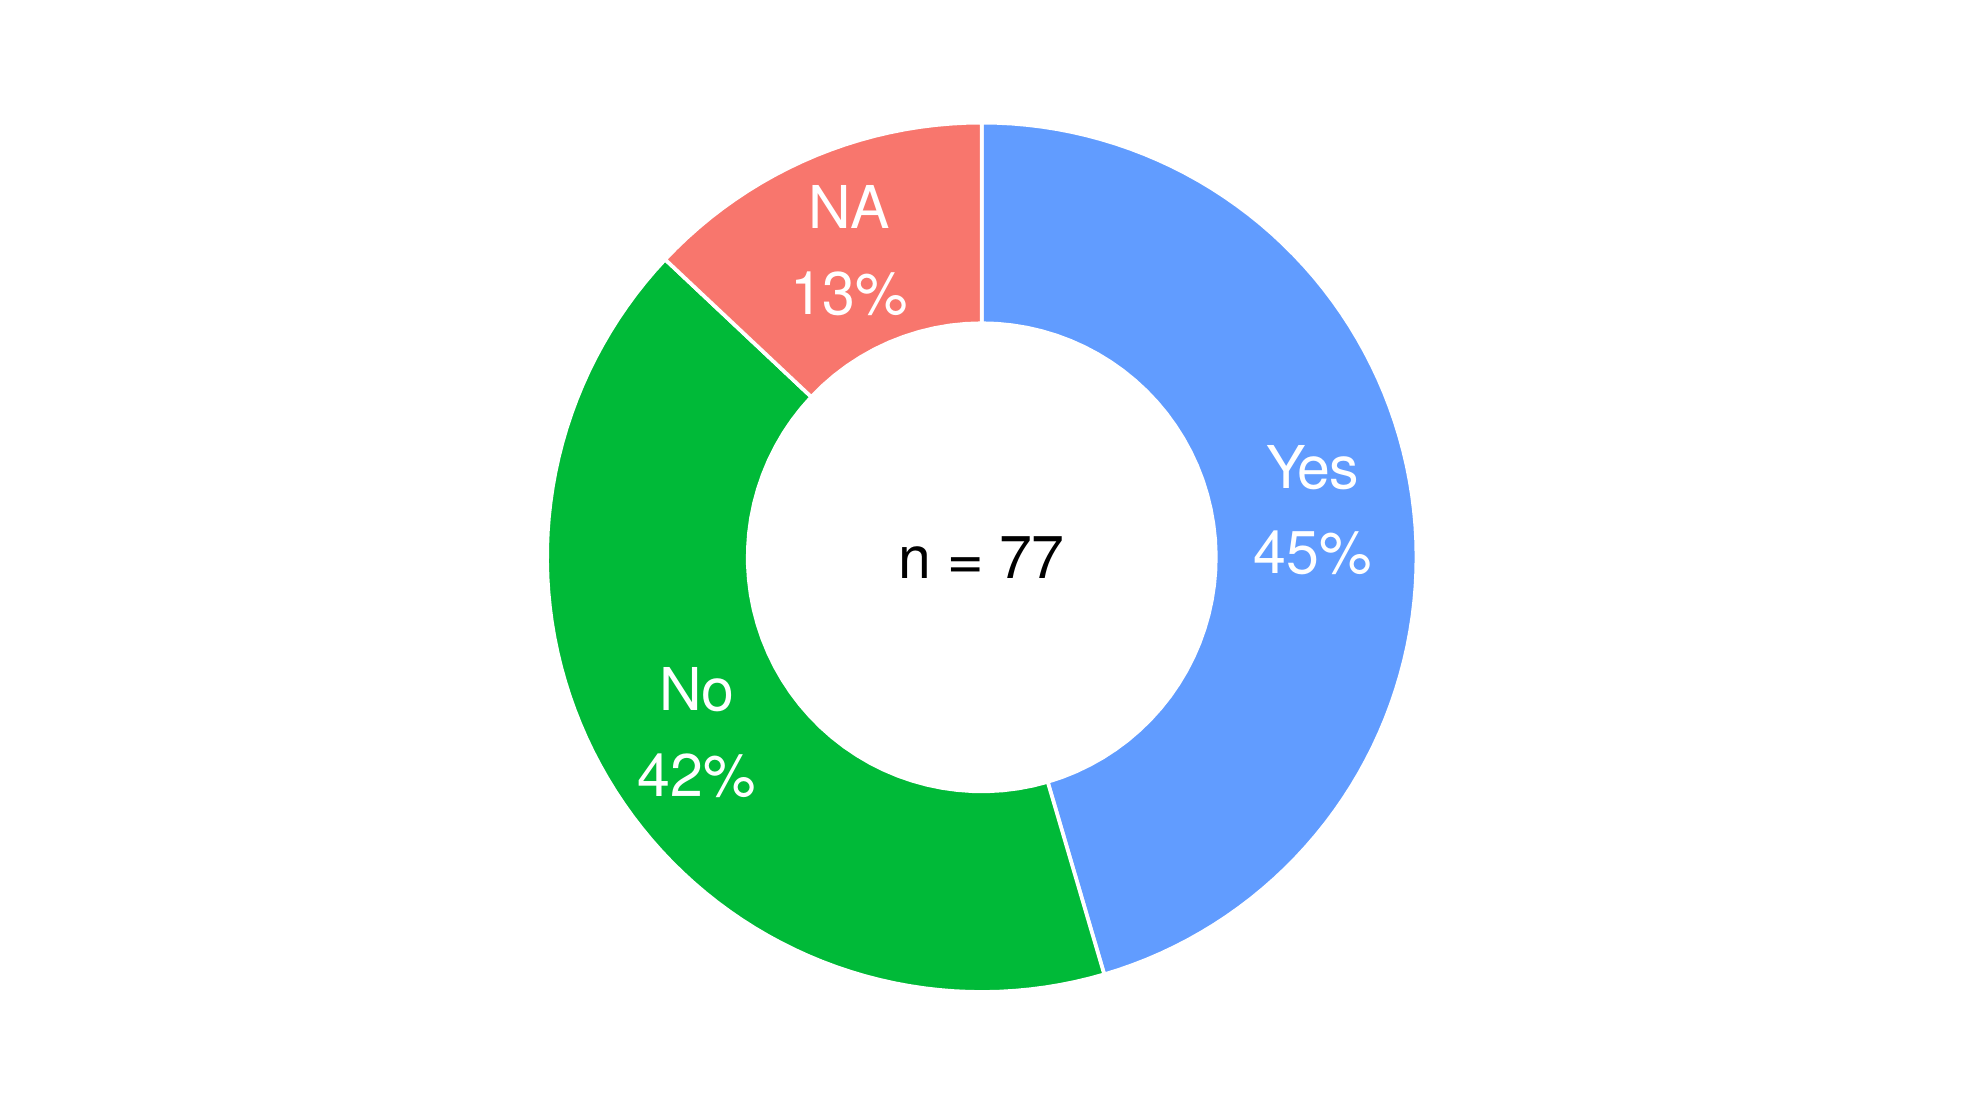}
  \end{subfigure}
  \hfill
  \begin{subfigure}[c]{0.59\textwidth}
    \includegraphics[height=5cm]{figures/blank.pdf}
  \end{subfigure}
\end{figure}

\noindent \textit{\textbf{Q17:} If yes, what kind of data?}

\noindent \newline The kind of data was specified in different levels of detail (e.g. from single words describing the format to more detailed descriptions of the anatomical structures, devices, modalities and parameters used for data acquisition). This is due to the open formulation of the question. The level of detail was not specified. 45\% of participants opted for “Yes”. 11\% of these did not specify the kind of data. 42\% of participants opted for “No”. Of these, 6\% specified the kind of data and 3\% specified a reason.

\newpage
\subsection{Where do we stand?}

\noindent \newline \textit{\textbf{Q18:} What do you regard as the most important developments in the field since the last workshop in June 2016?}

\noindent \newline 38\% of participants responded to this question. 36 partial replies were extracted from the free text and categorized.

\begin{figure}[pos=h]
  \begin{subfigure}[c]{0.4\textwidth}
    \includegraphics[width=\textwidth, trim=4cm 1cm 4cm 1cm, clip]{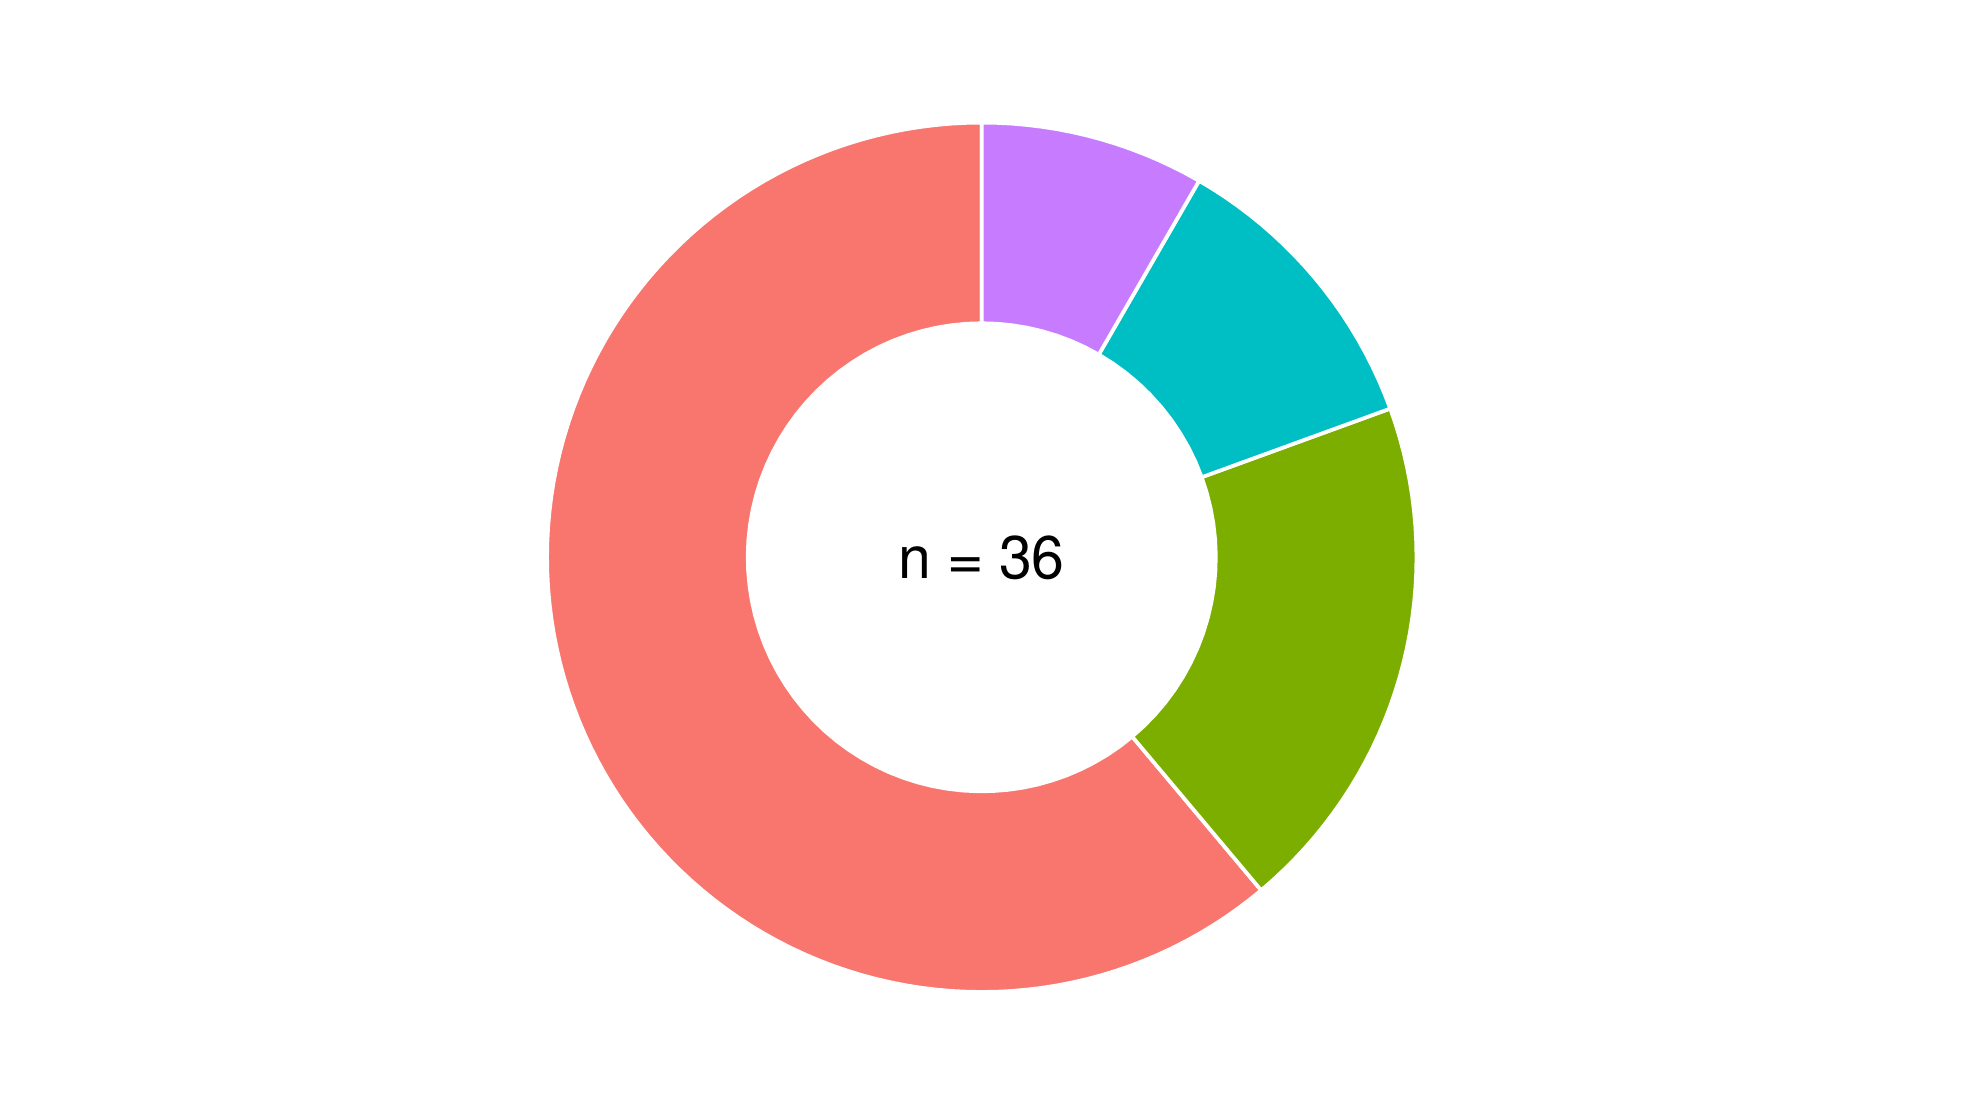}
  \end{subfigure}
  \hfill
  \begin{subfigure}[c]{0.59\textwidth}
    \includegraphics[height=5cm, trim=4.5cm 2cm 0cm 2cm, clip]{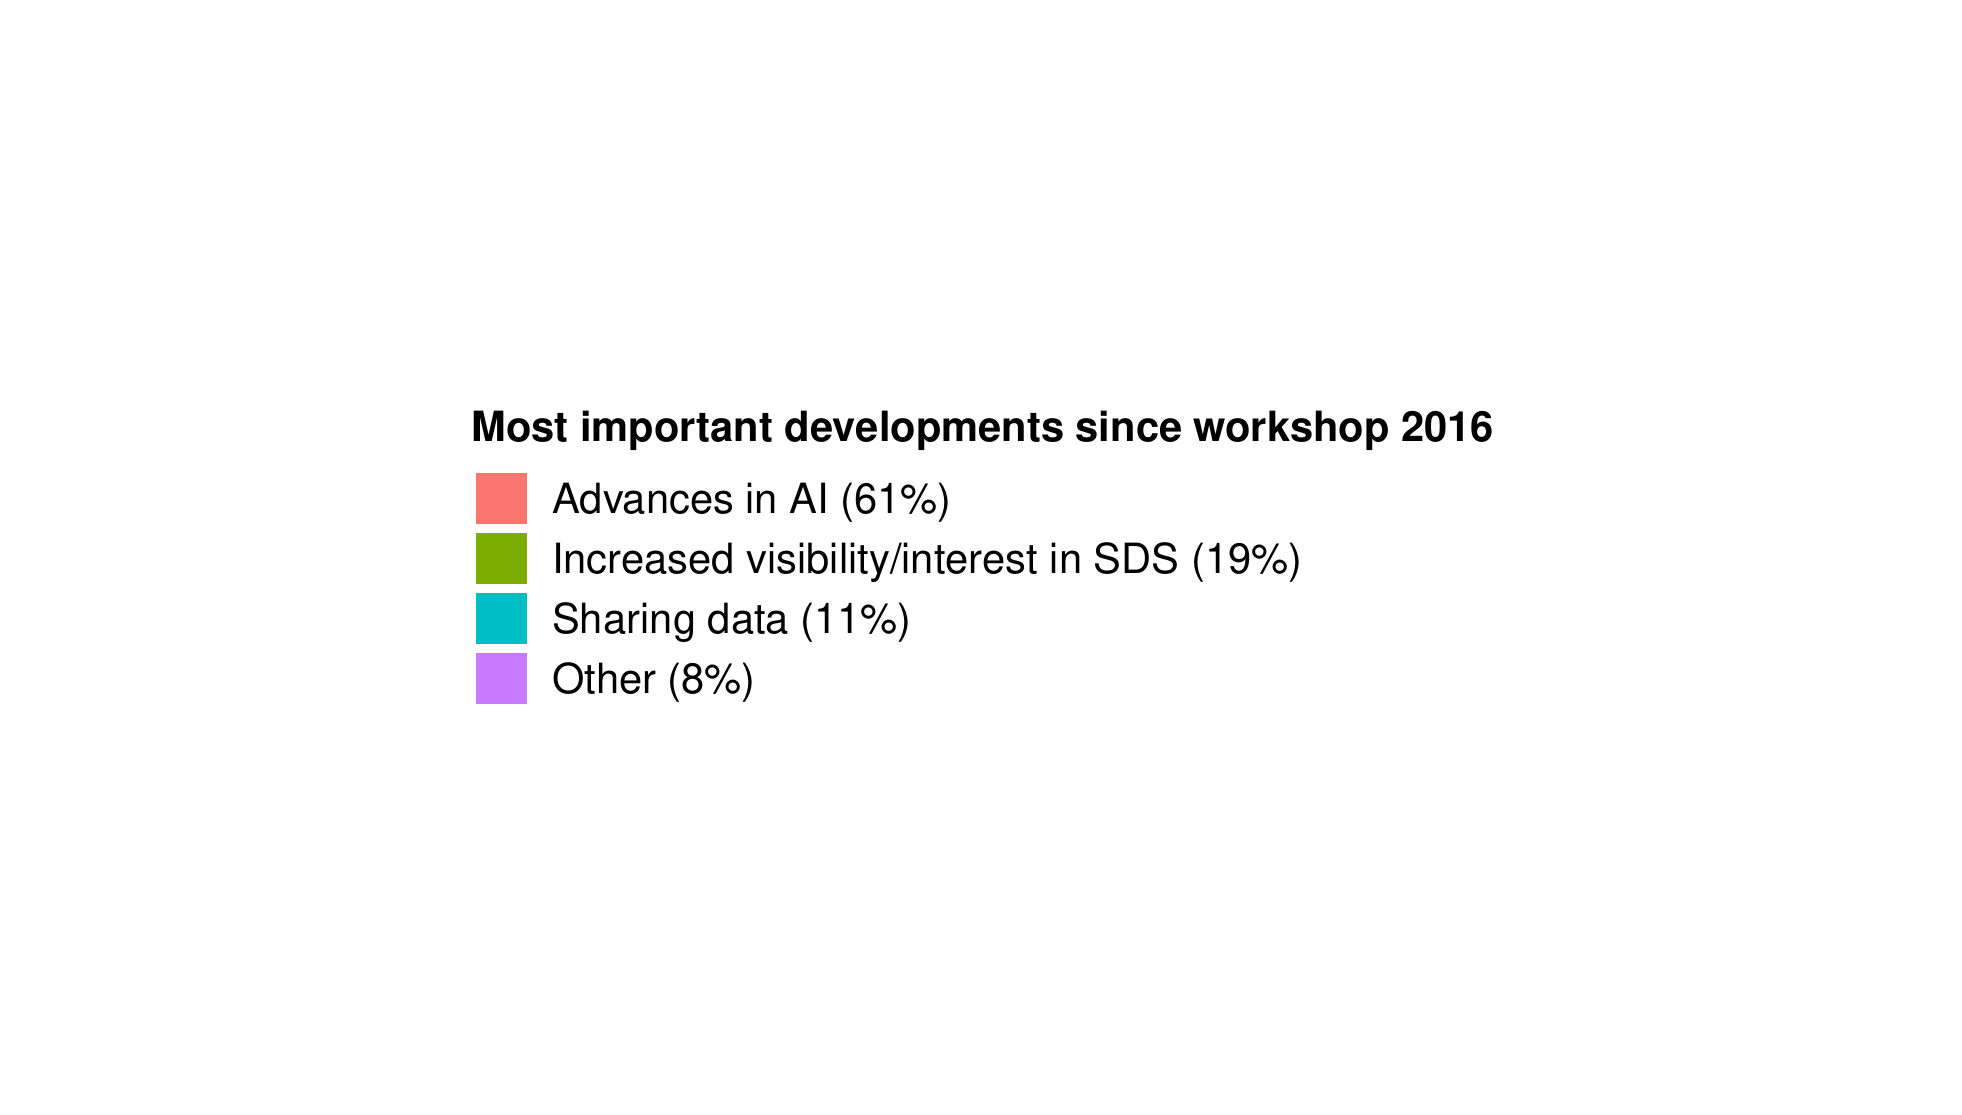}
  \end{subfigure}
\end{figure}

\noindent \textit{\textbf{Q19:} Surgical Data Science failures: Are you aware of projects that have failed (optionally and preferably: name them)?}

\noindent \newline 27\% of participants were aware of at least one project that failed, yielded to 28 failing projects in total. IBM Watson was the only project mentioned multiple times (which is not even a SDS project). 73\% of participants did not name or were not aware of any failing project. Of these, 5\% still named reasons for failures.

\vspace{\baselineskip}

\noindent \textit{\textbf{Q20:} What was the (main) reason for failure?}

\begin{figure}[pos=h]
  \begin{subfigure}[c]{0.4\textwidth}
    \includegraphics[width=\textwidth, trim=4cm 1cm 4cm 1cm, clip]{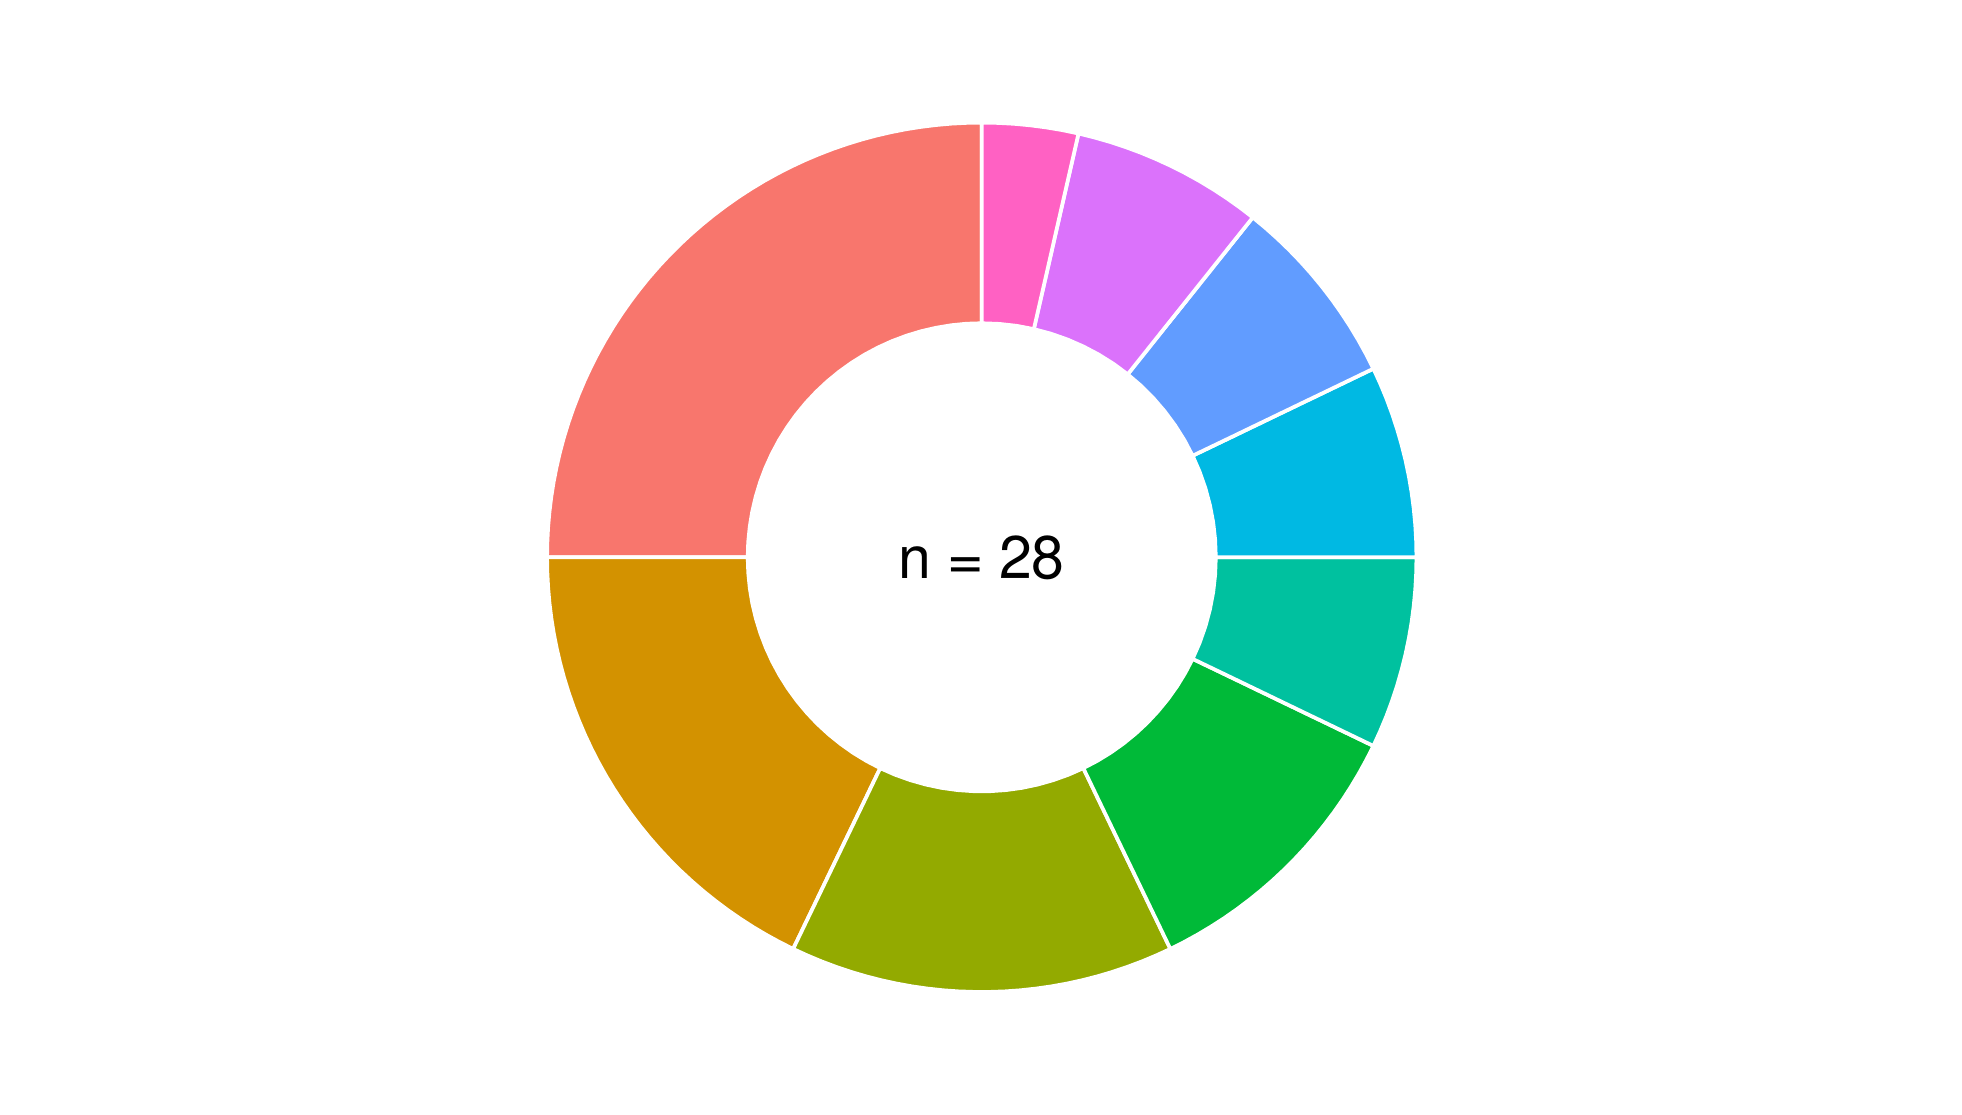}
  \end{subfigure}
  \hfill
  \begin{subfigure}[c]{0.59\textwidth}
    \includegraphics[height=5cm, trim=4.5cm 2cm 0cm 2cm, clip]{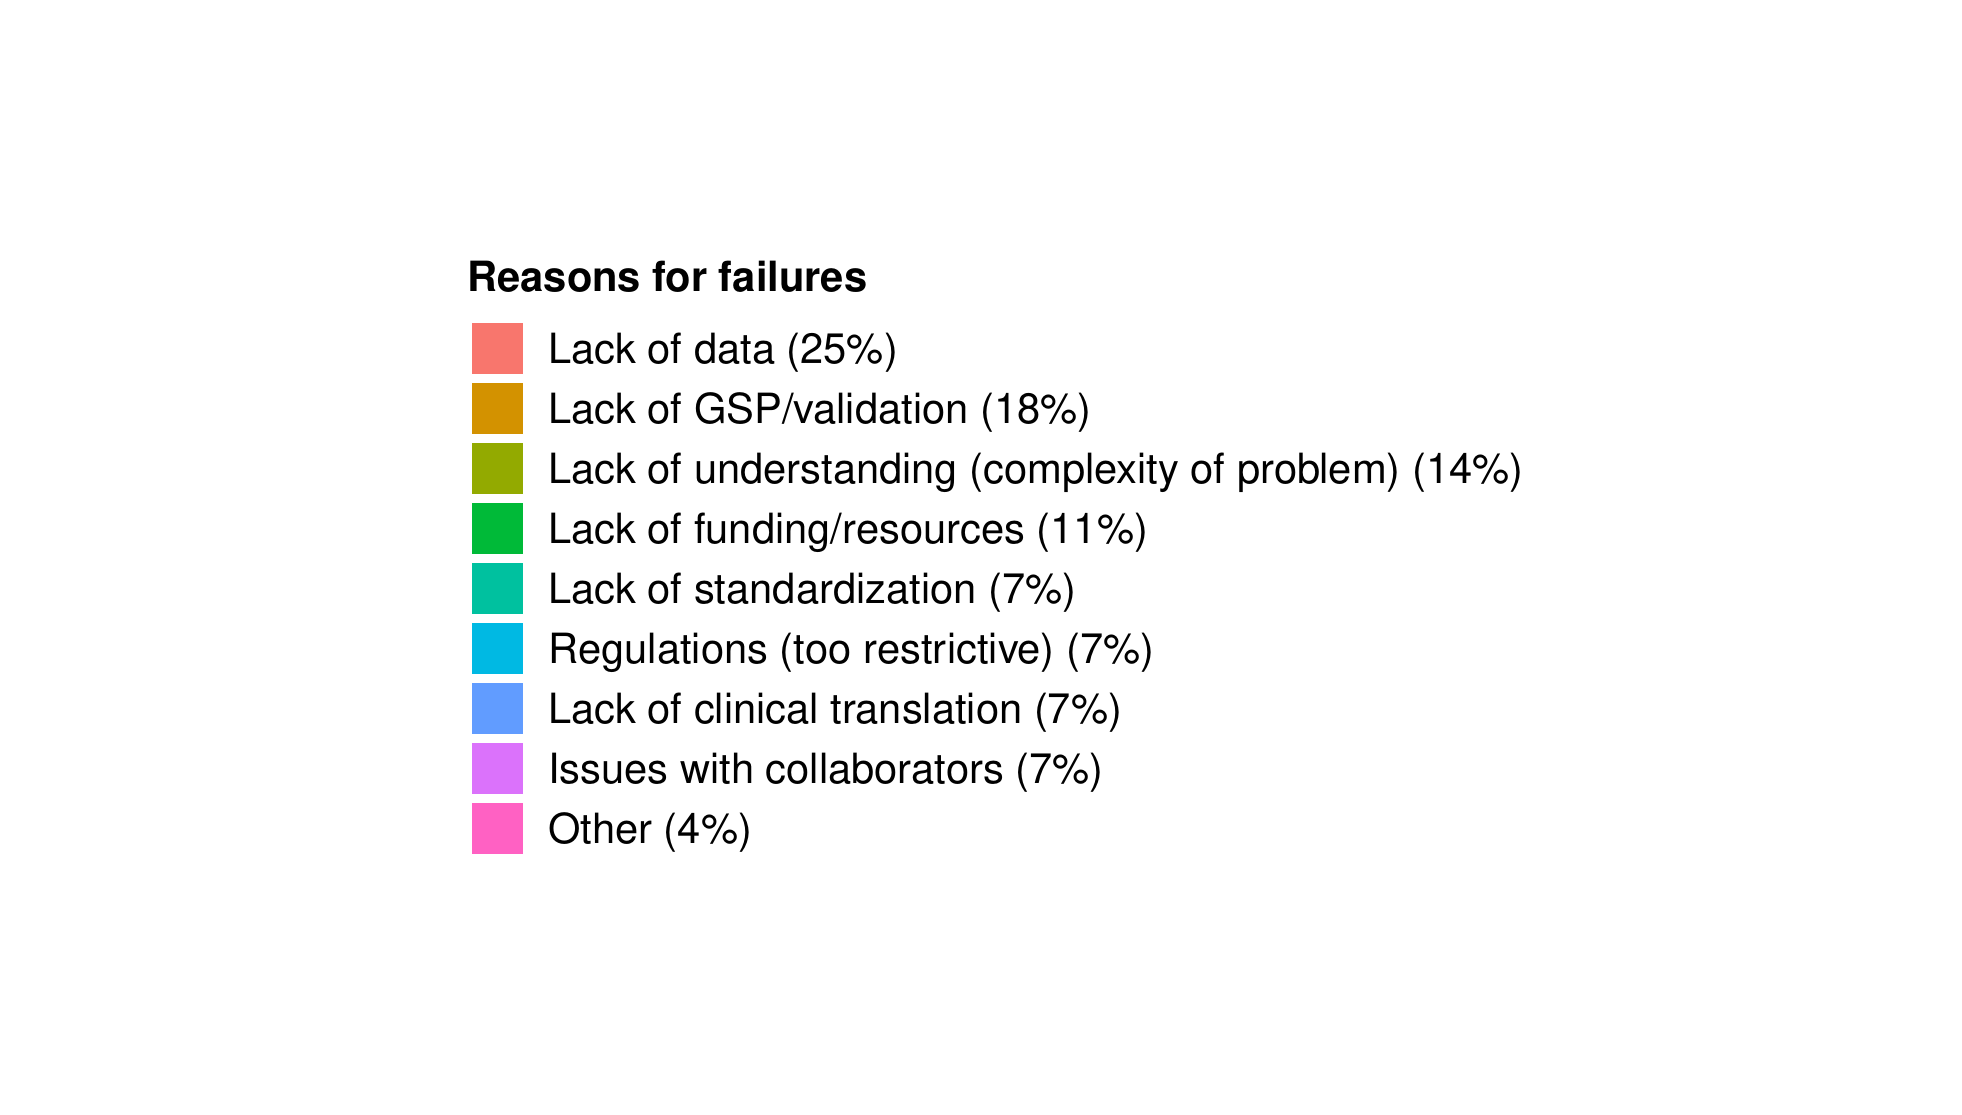}
  \end{subfigure}
\end{figure}
